# Supplementary material for: Learning A Physical Long-term Predictor
Source: arXiv:1703.00247 source file (2017-03-01)
Supplement: Supplementary file 1 [file supp.tex]

\begingroup
\def\rowheight{9.5em}
\begin{figure*}[h]
\centering
\begin{minipage}[t]{\linewidth}
\includegraphics[height=\rowheight]{images/results/S1_samples/S1_00_time_40.pdf}
\includegraphics[height=\rowheight]{images/results/S1_samples/S1_00_time_40_ellipses.pdf}
\includegraphics[height=\rowheight]{images/results/S1_samples/S1_00_time_40_heatmap_20.pdf}
\includegraphics[height=\rowheight]{images/results/S1_samples/S1_00_time_40_heatmap_20_crop.pdf}
\includegraphics[height=\rowheight]{images/results/S1_samples/S1_00_time_40_heatmap_30.pdf}
\includegraphics[height=\rowheight]{images/results/S1_samples/S1_00_time_40_heatmap_30_crop.pdf}
\includegraphics[height=\rowheight]{images/results/S1_samples/S1_00_time_40_heatmap_40.pdf}
\includegraphics[height=\rowheight]{images/results/S1_samples/S1_00_time_40_heatmap_40_crop.pdf}
\end{minipage}\\
\caption{Randomly chosen output experiment \#0}
\end{figure*}
\begin{figure*}[h]
\centering
\begin{minipage}[t]{\linewidth}
\includegraphics[height=\rowheight]{images/results/S1_samples/S1_01_time_40.pdf}
\includegraphics[height=\rowheight]{images/results/S1_samples/S1_01_time_40_ellipses.pdf}
\includegraphics[height=\rowheight]{images/results/S1_samples/S1_01_time_40_heatmap_20.pdf}
\includegraphics[height=\rowheight]{images/results/S1_samples/S1_01_time_40_heatmap_30.pdf}
\includegraphics[height=\rowheight]{images/results/S1_samples/S1_01_time_40_heatmap_40.pdf}
\end{minipage}\\
\caption{Randomly chosen output experiment \#1}
\end{figure*}
\begin{figure*}[h]
\centering
\begin{minipage}[t]{\linewidth}
\includegraphics[height=\rowheight]{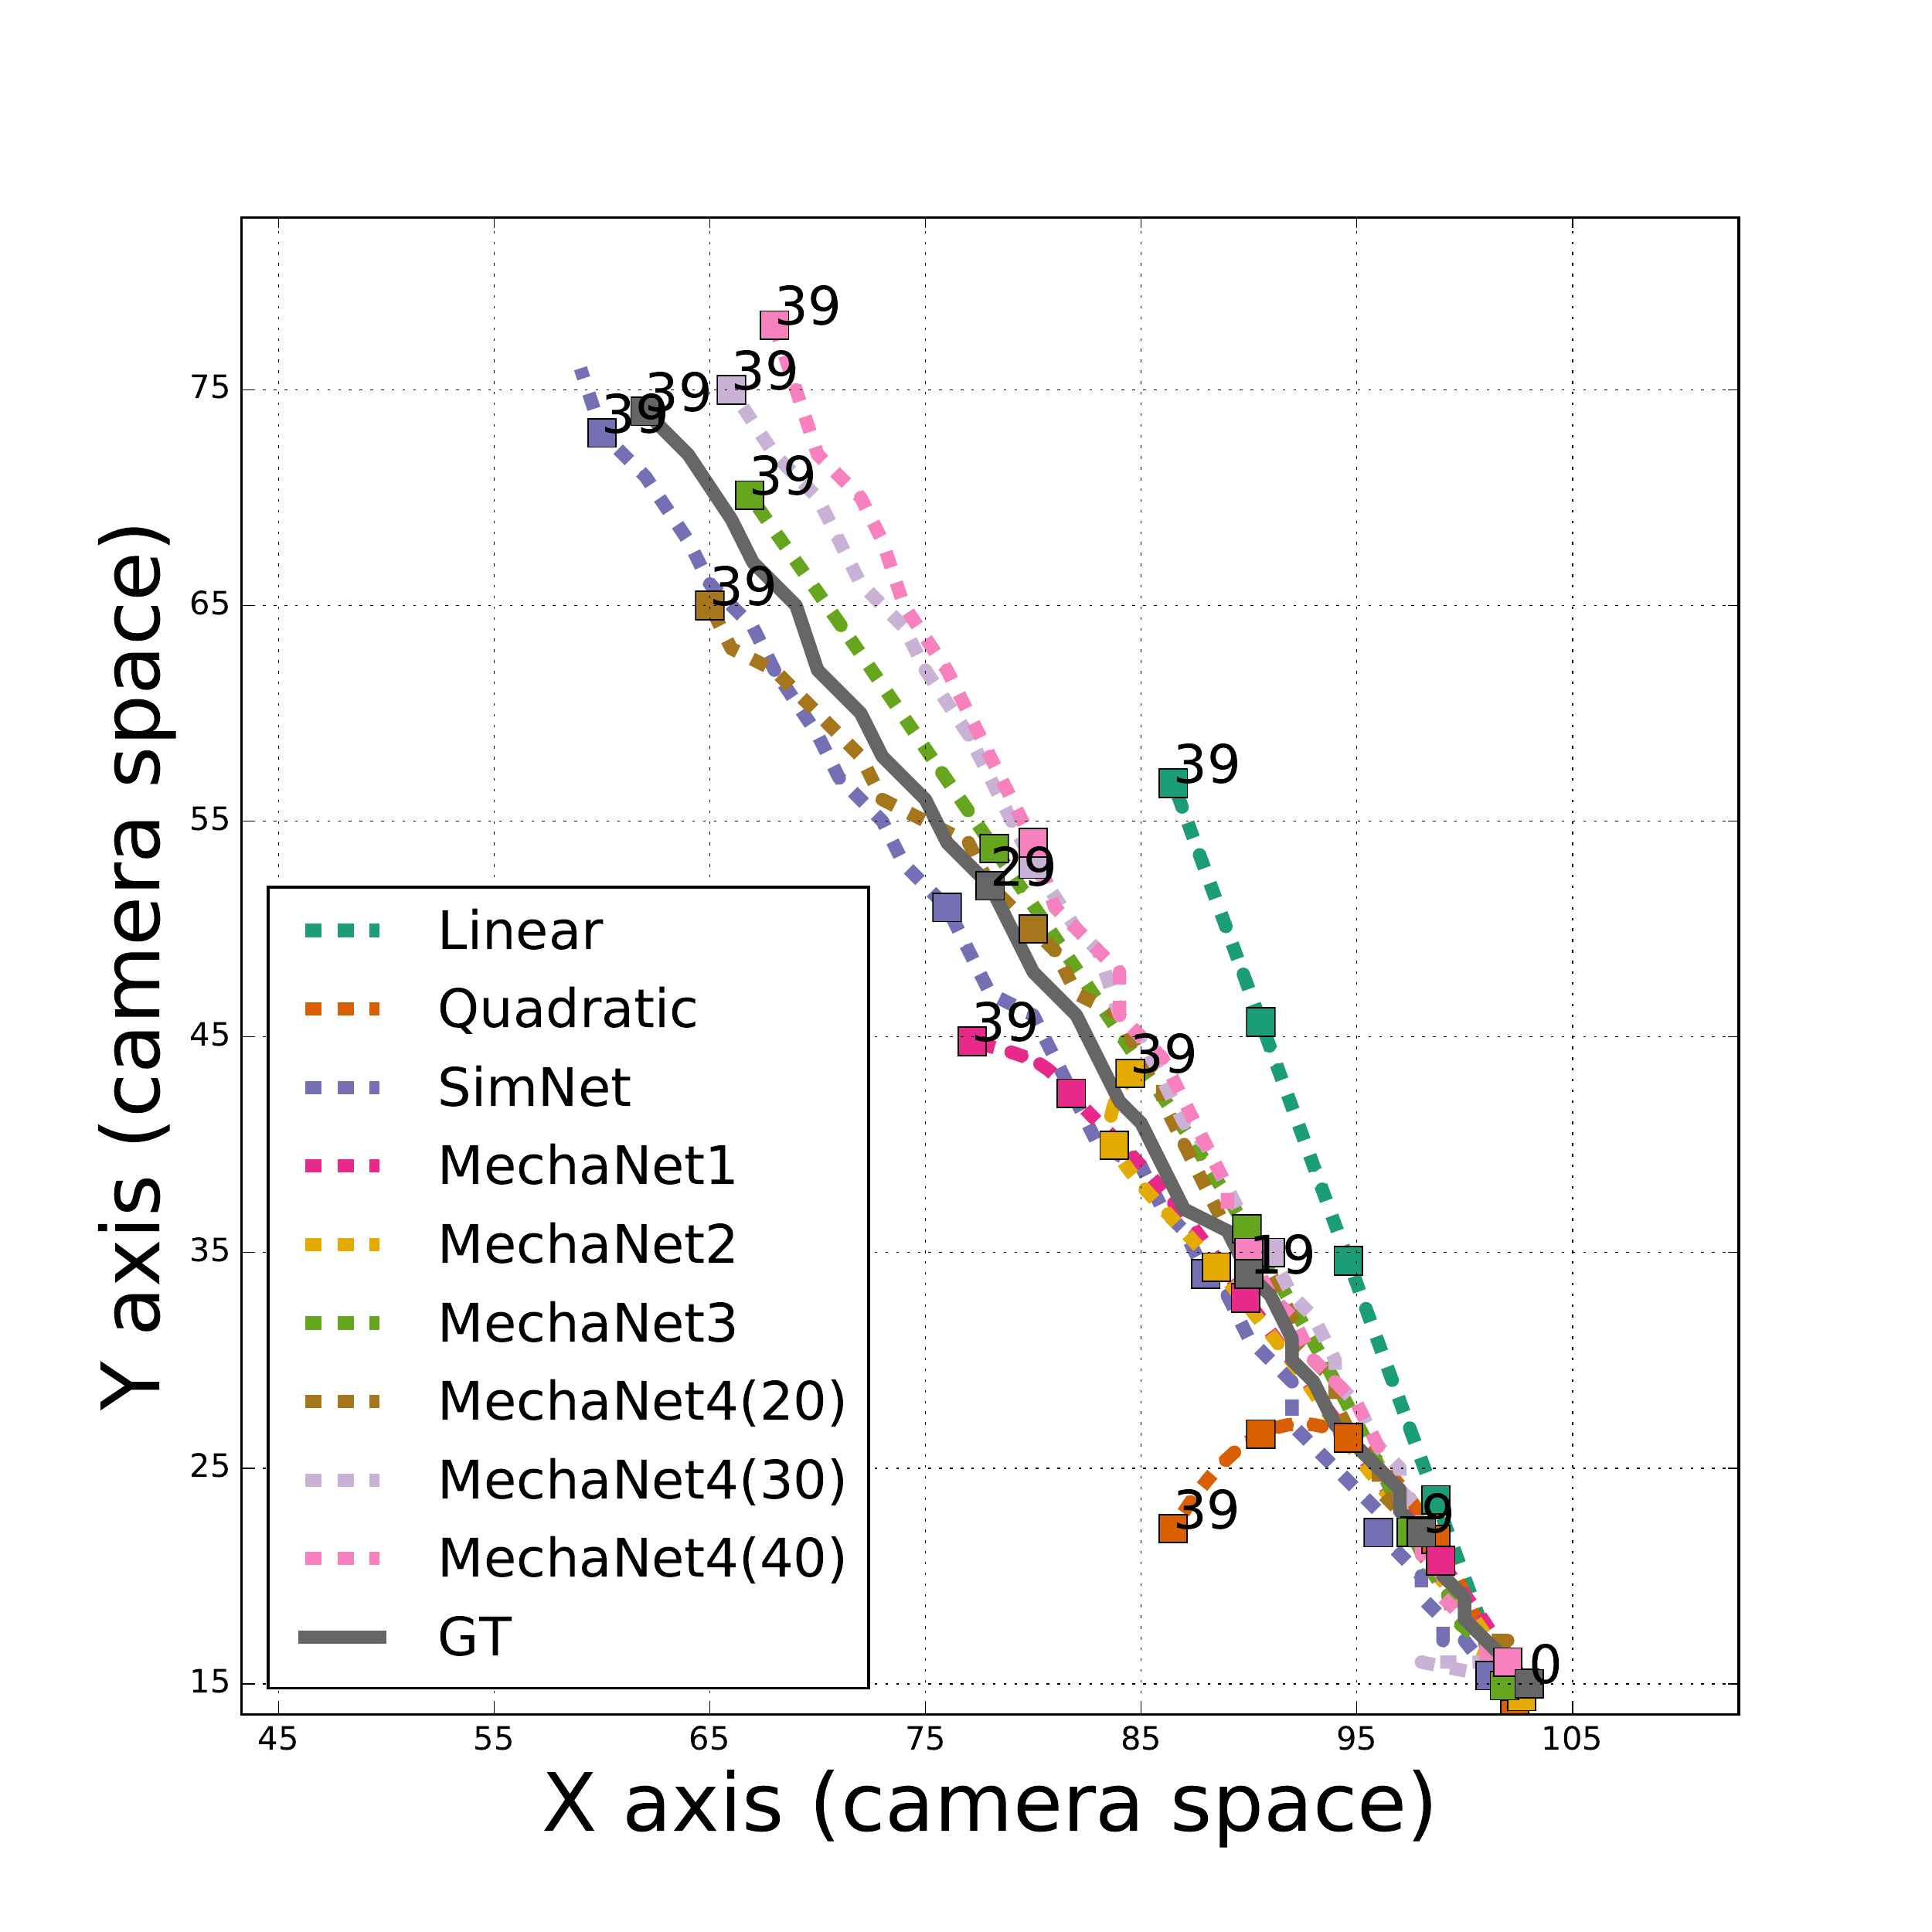}
\includegraphics[height=\rowheight]{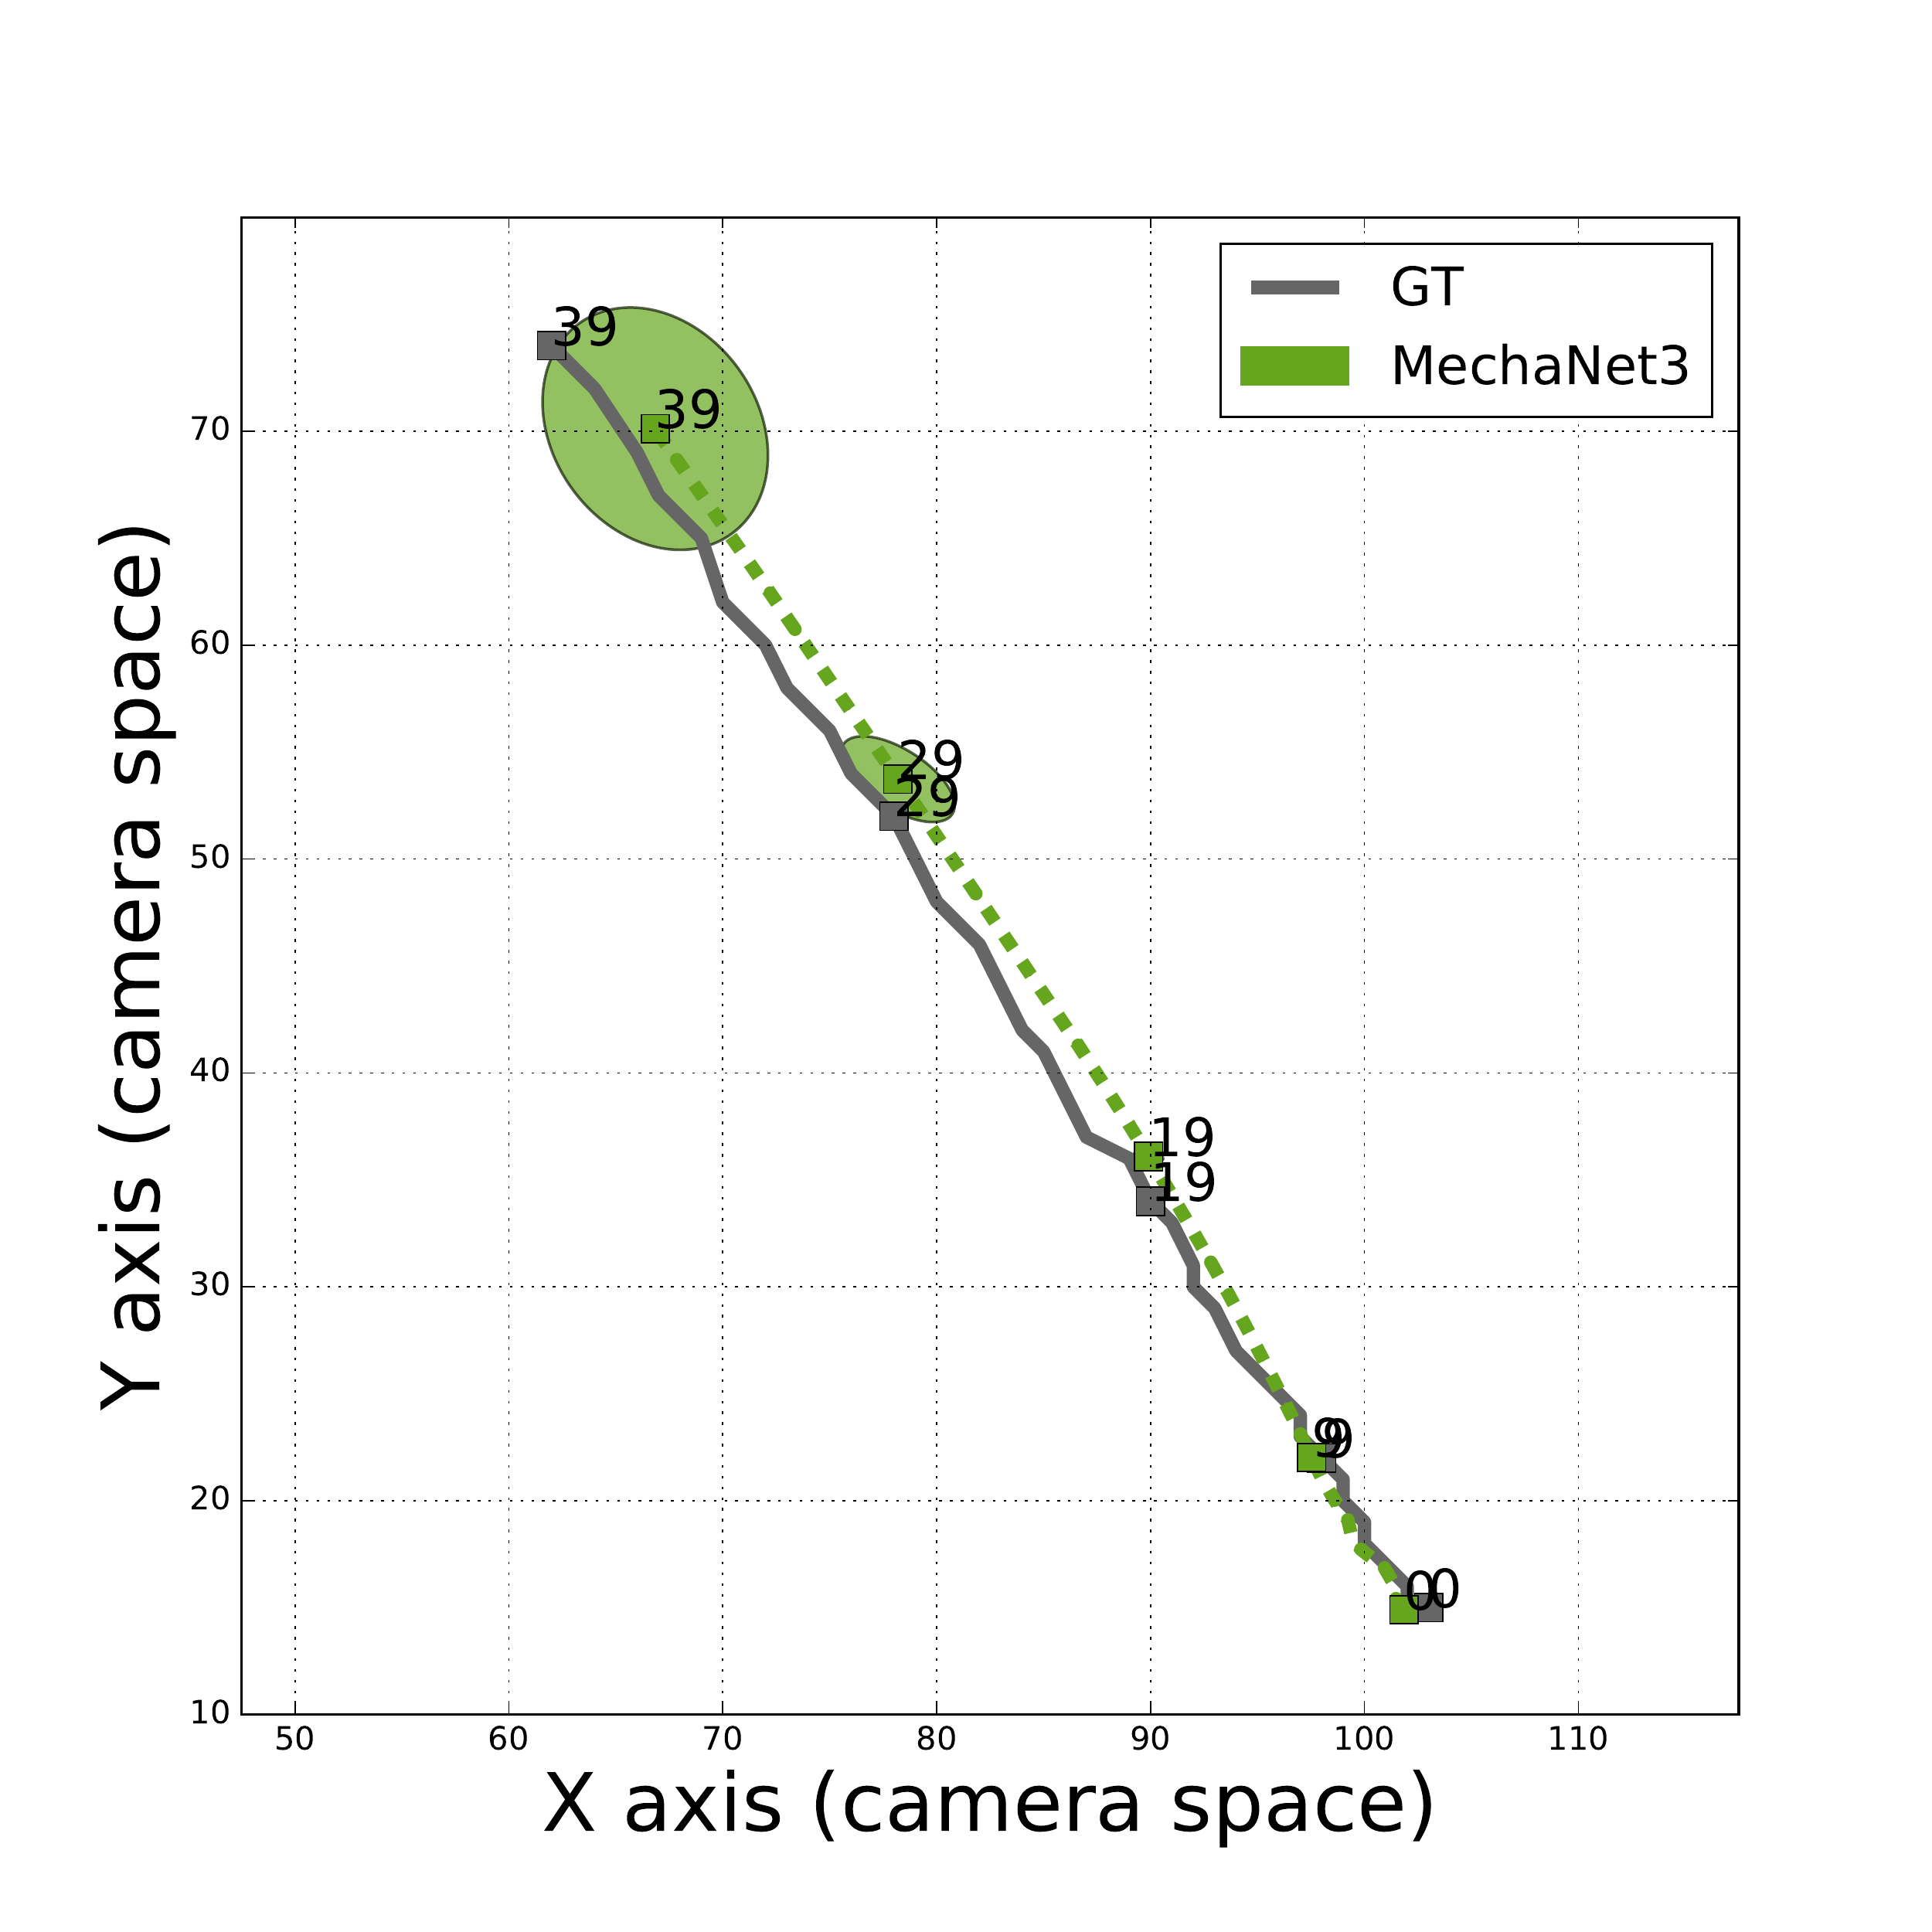}
\includegraphics[height=\rowheight]{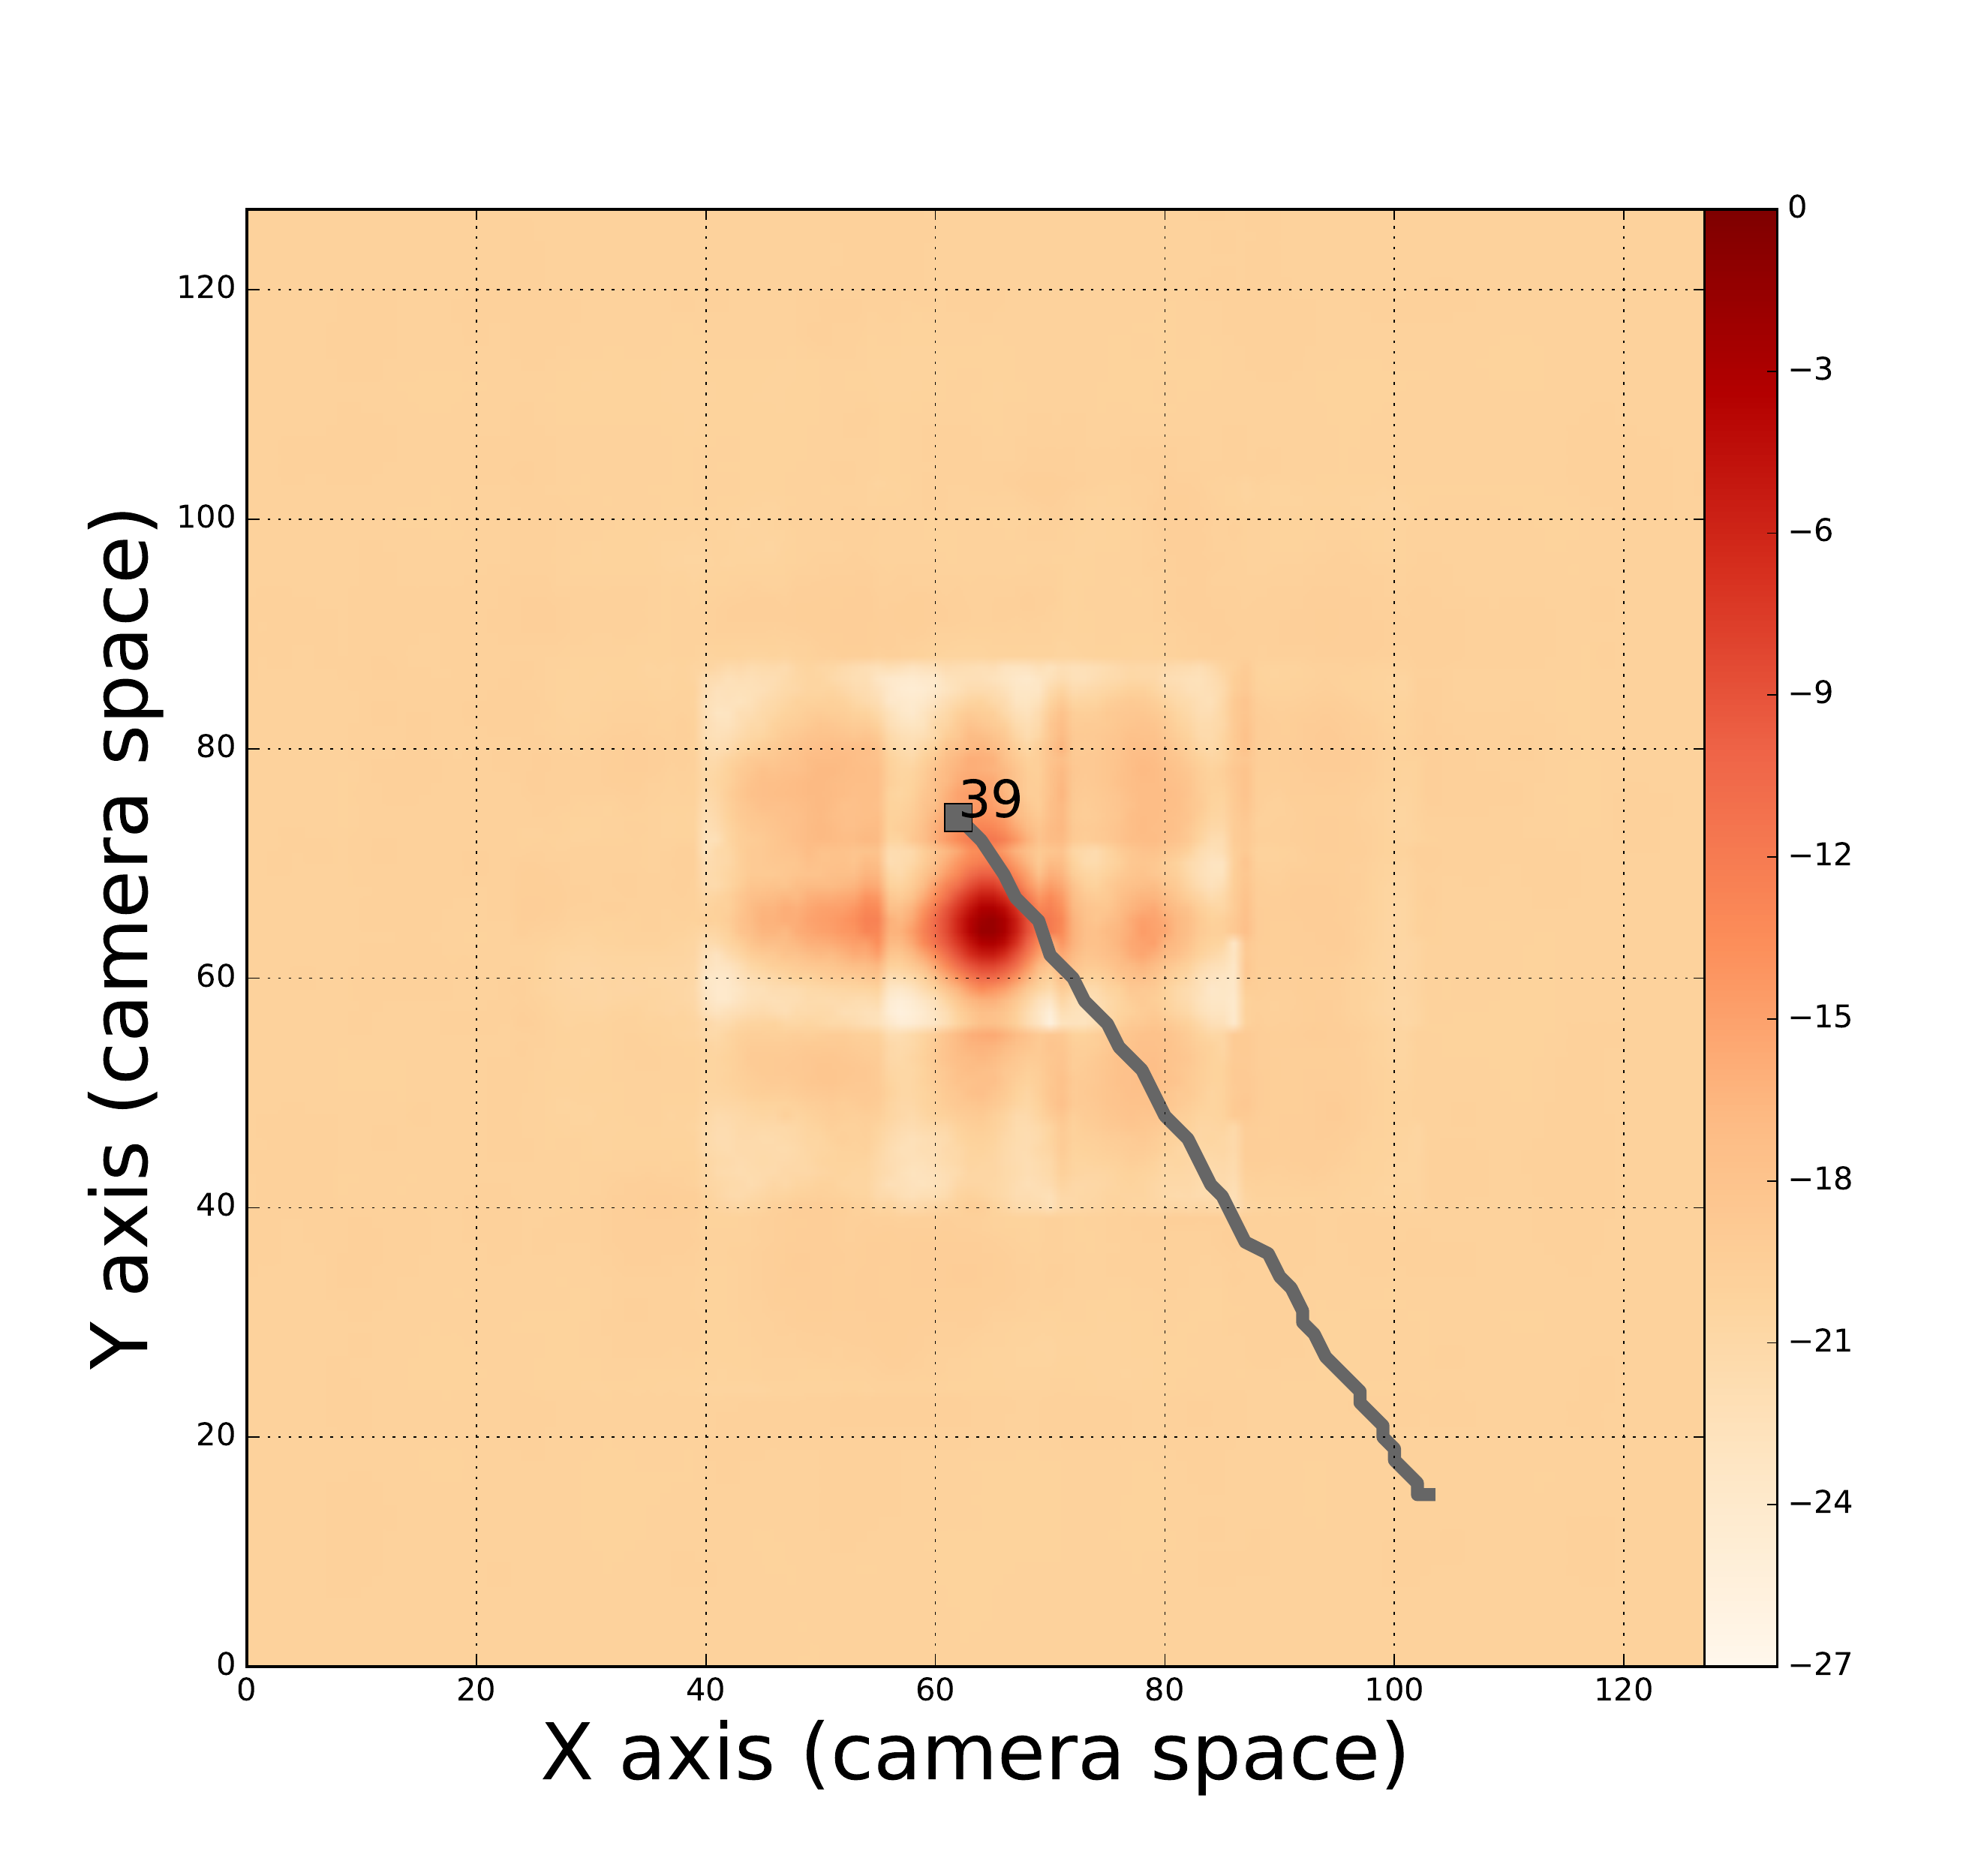}
\includegraphics[height=\rowheight]{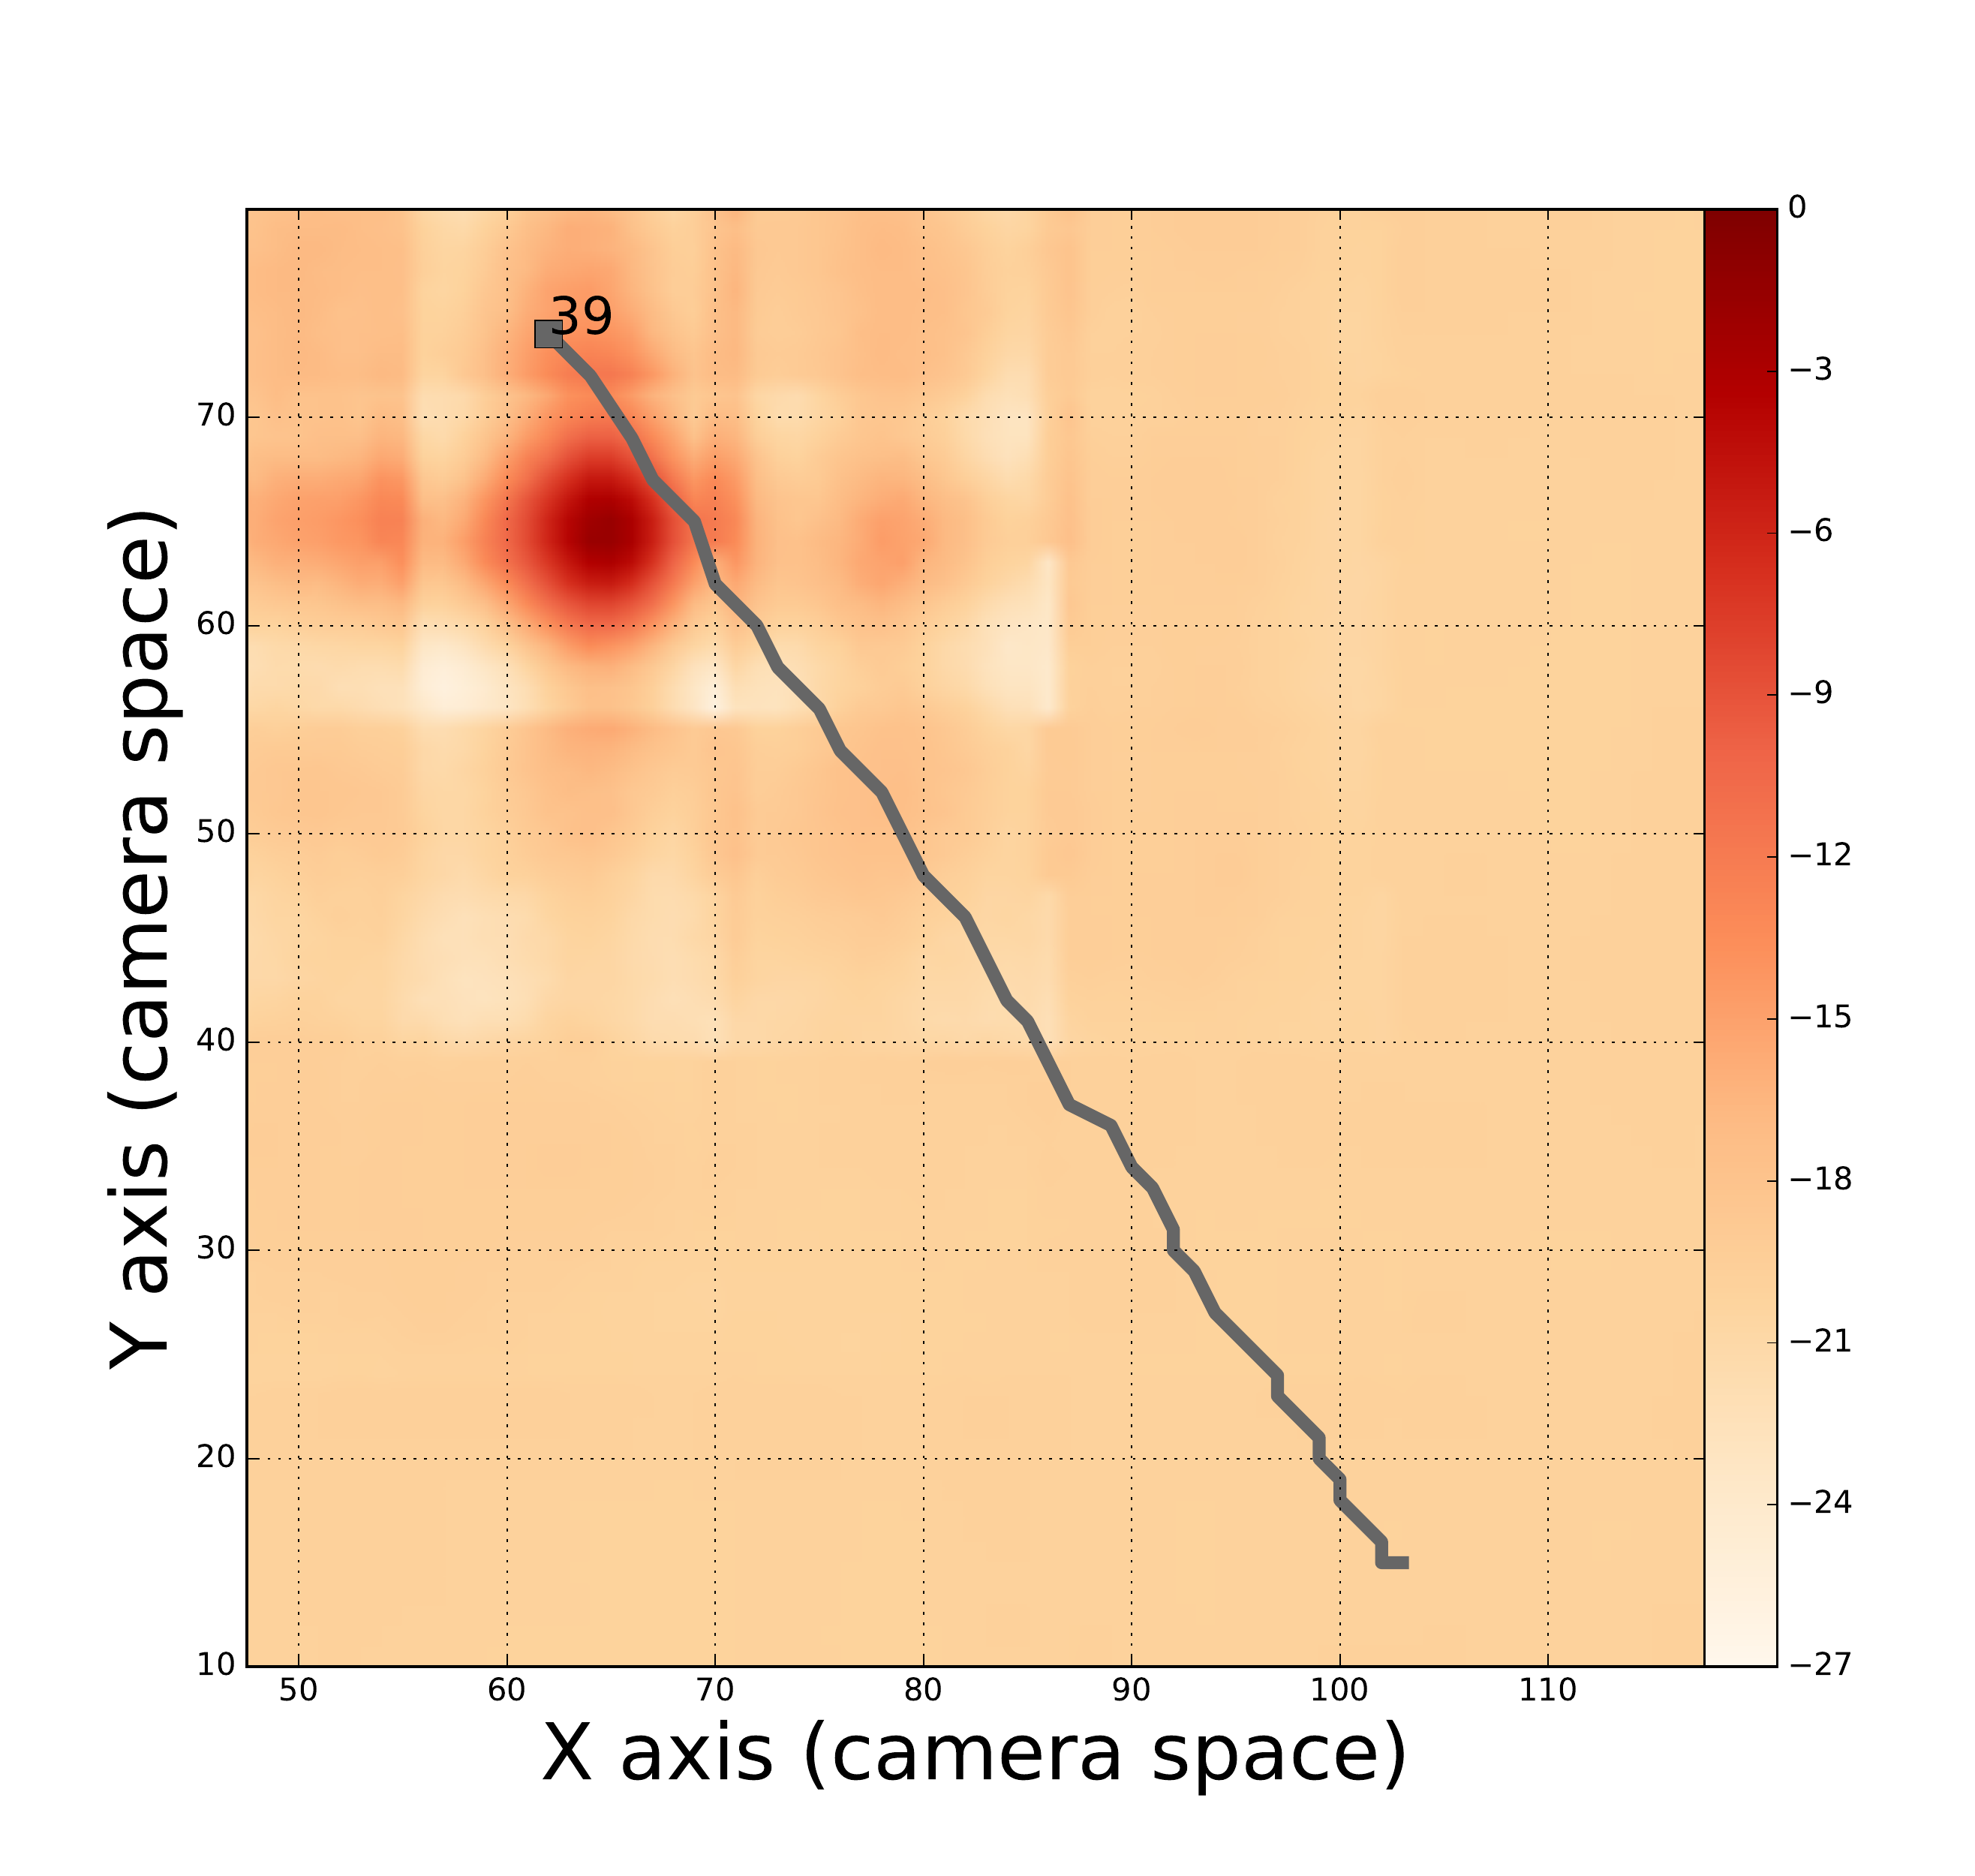}
\includegraphics[height=\rowheight]{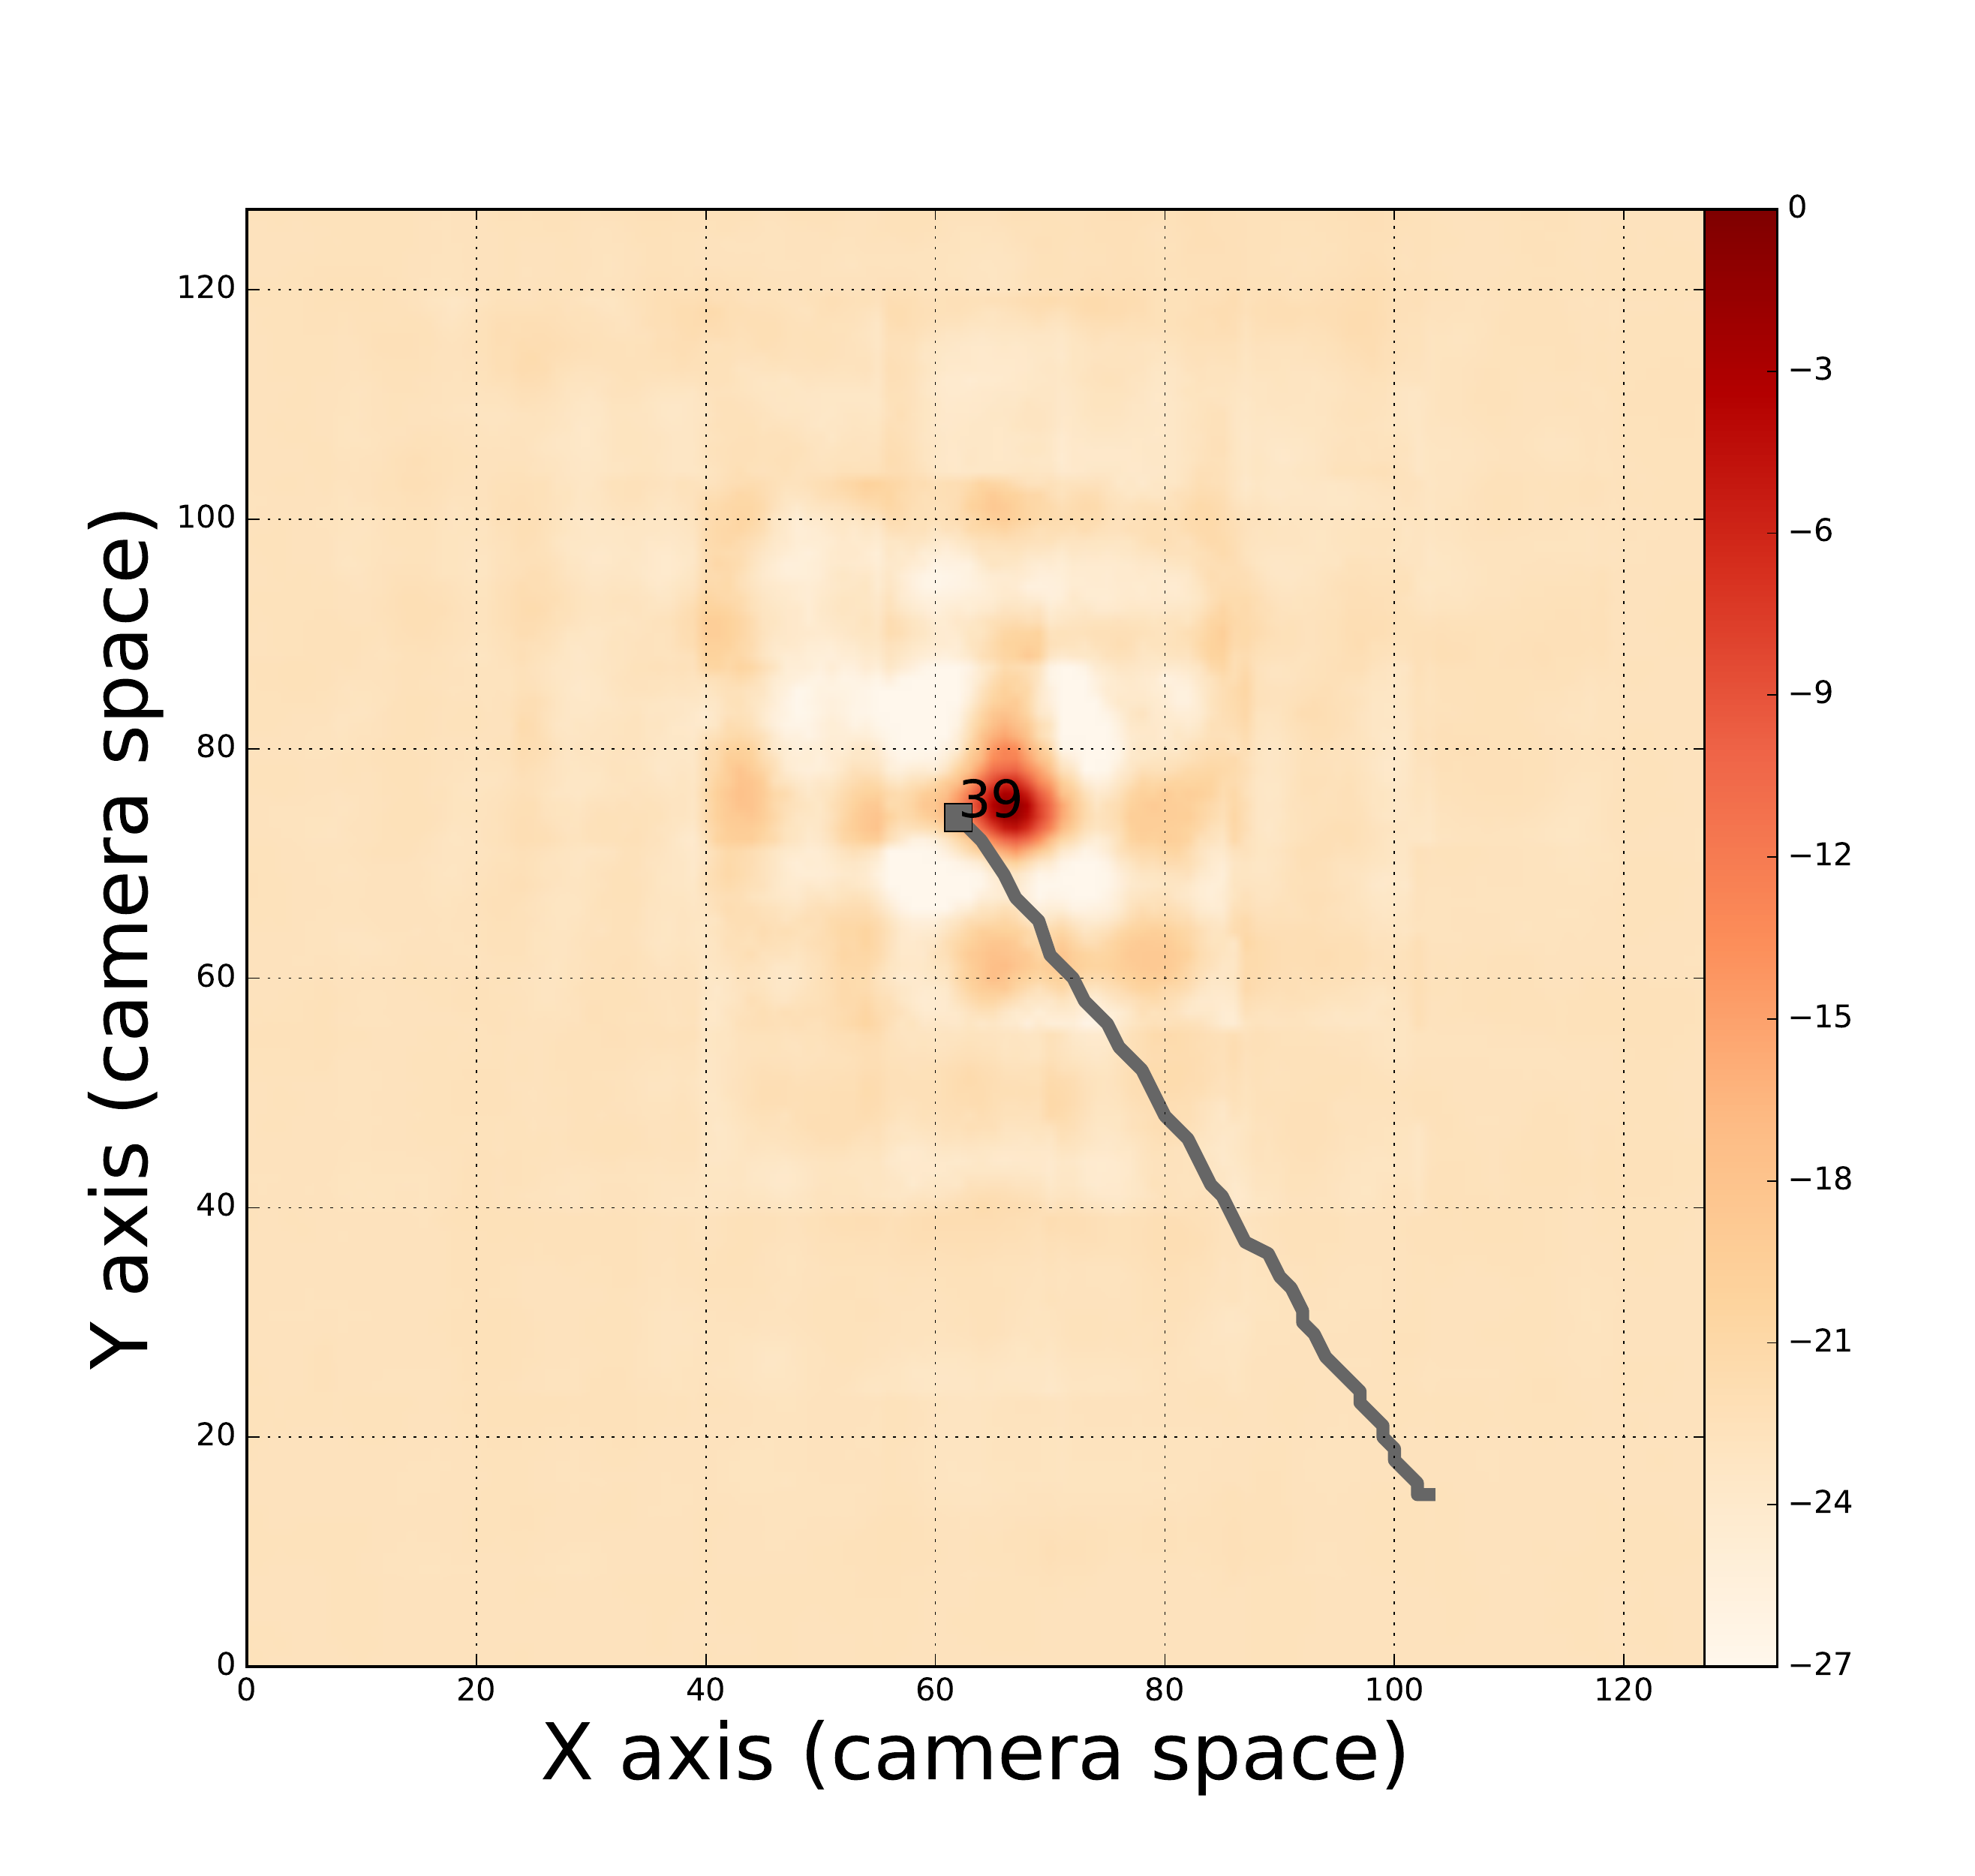}
\includegraphics[height=\rowheight]{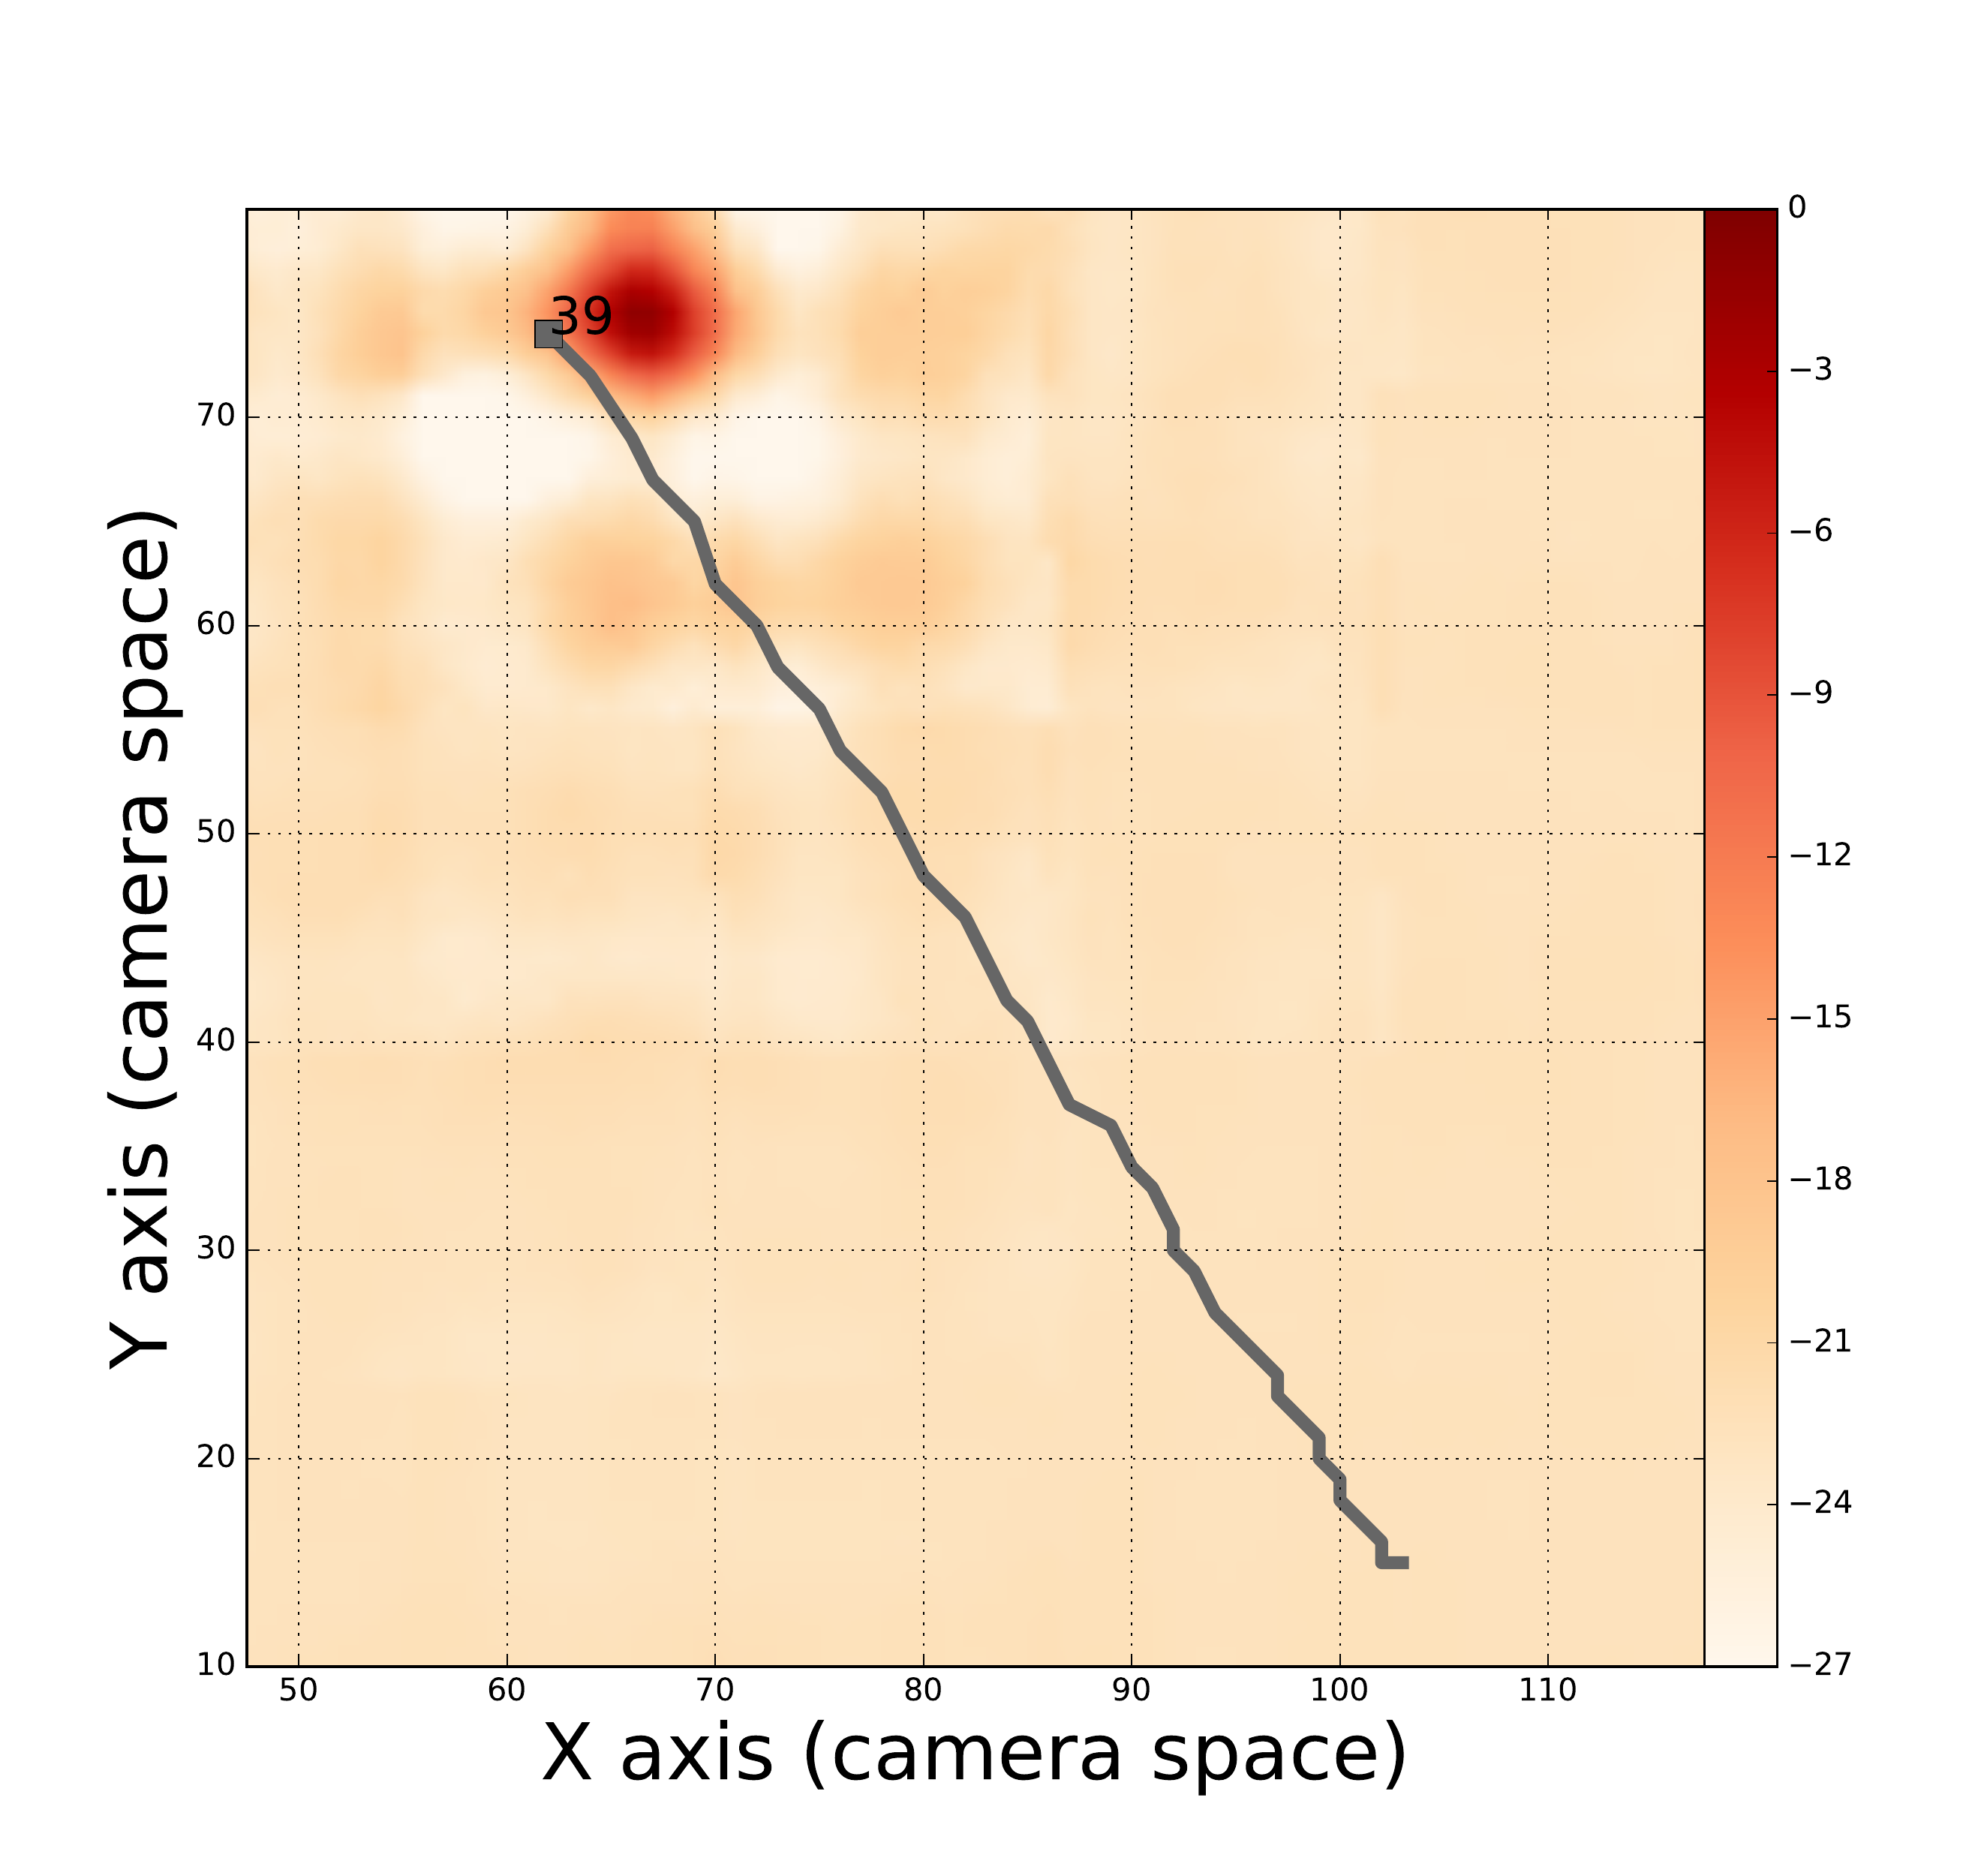}
\includegraphics[height=\rowheight]{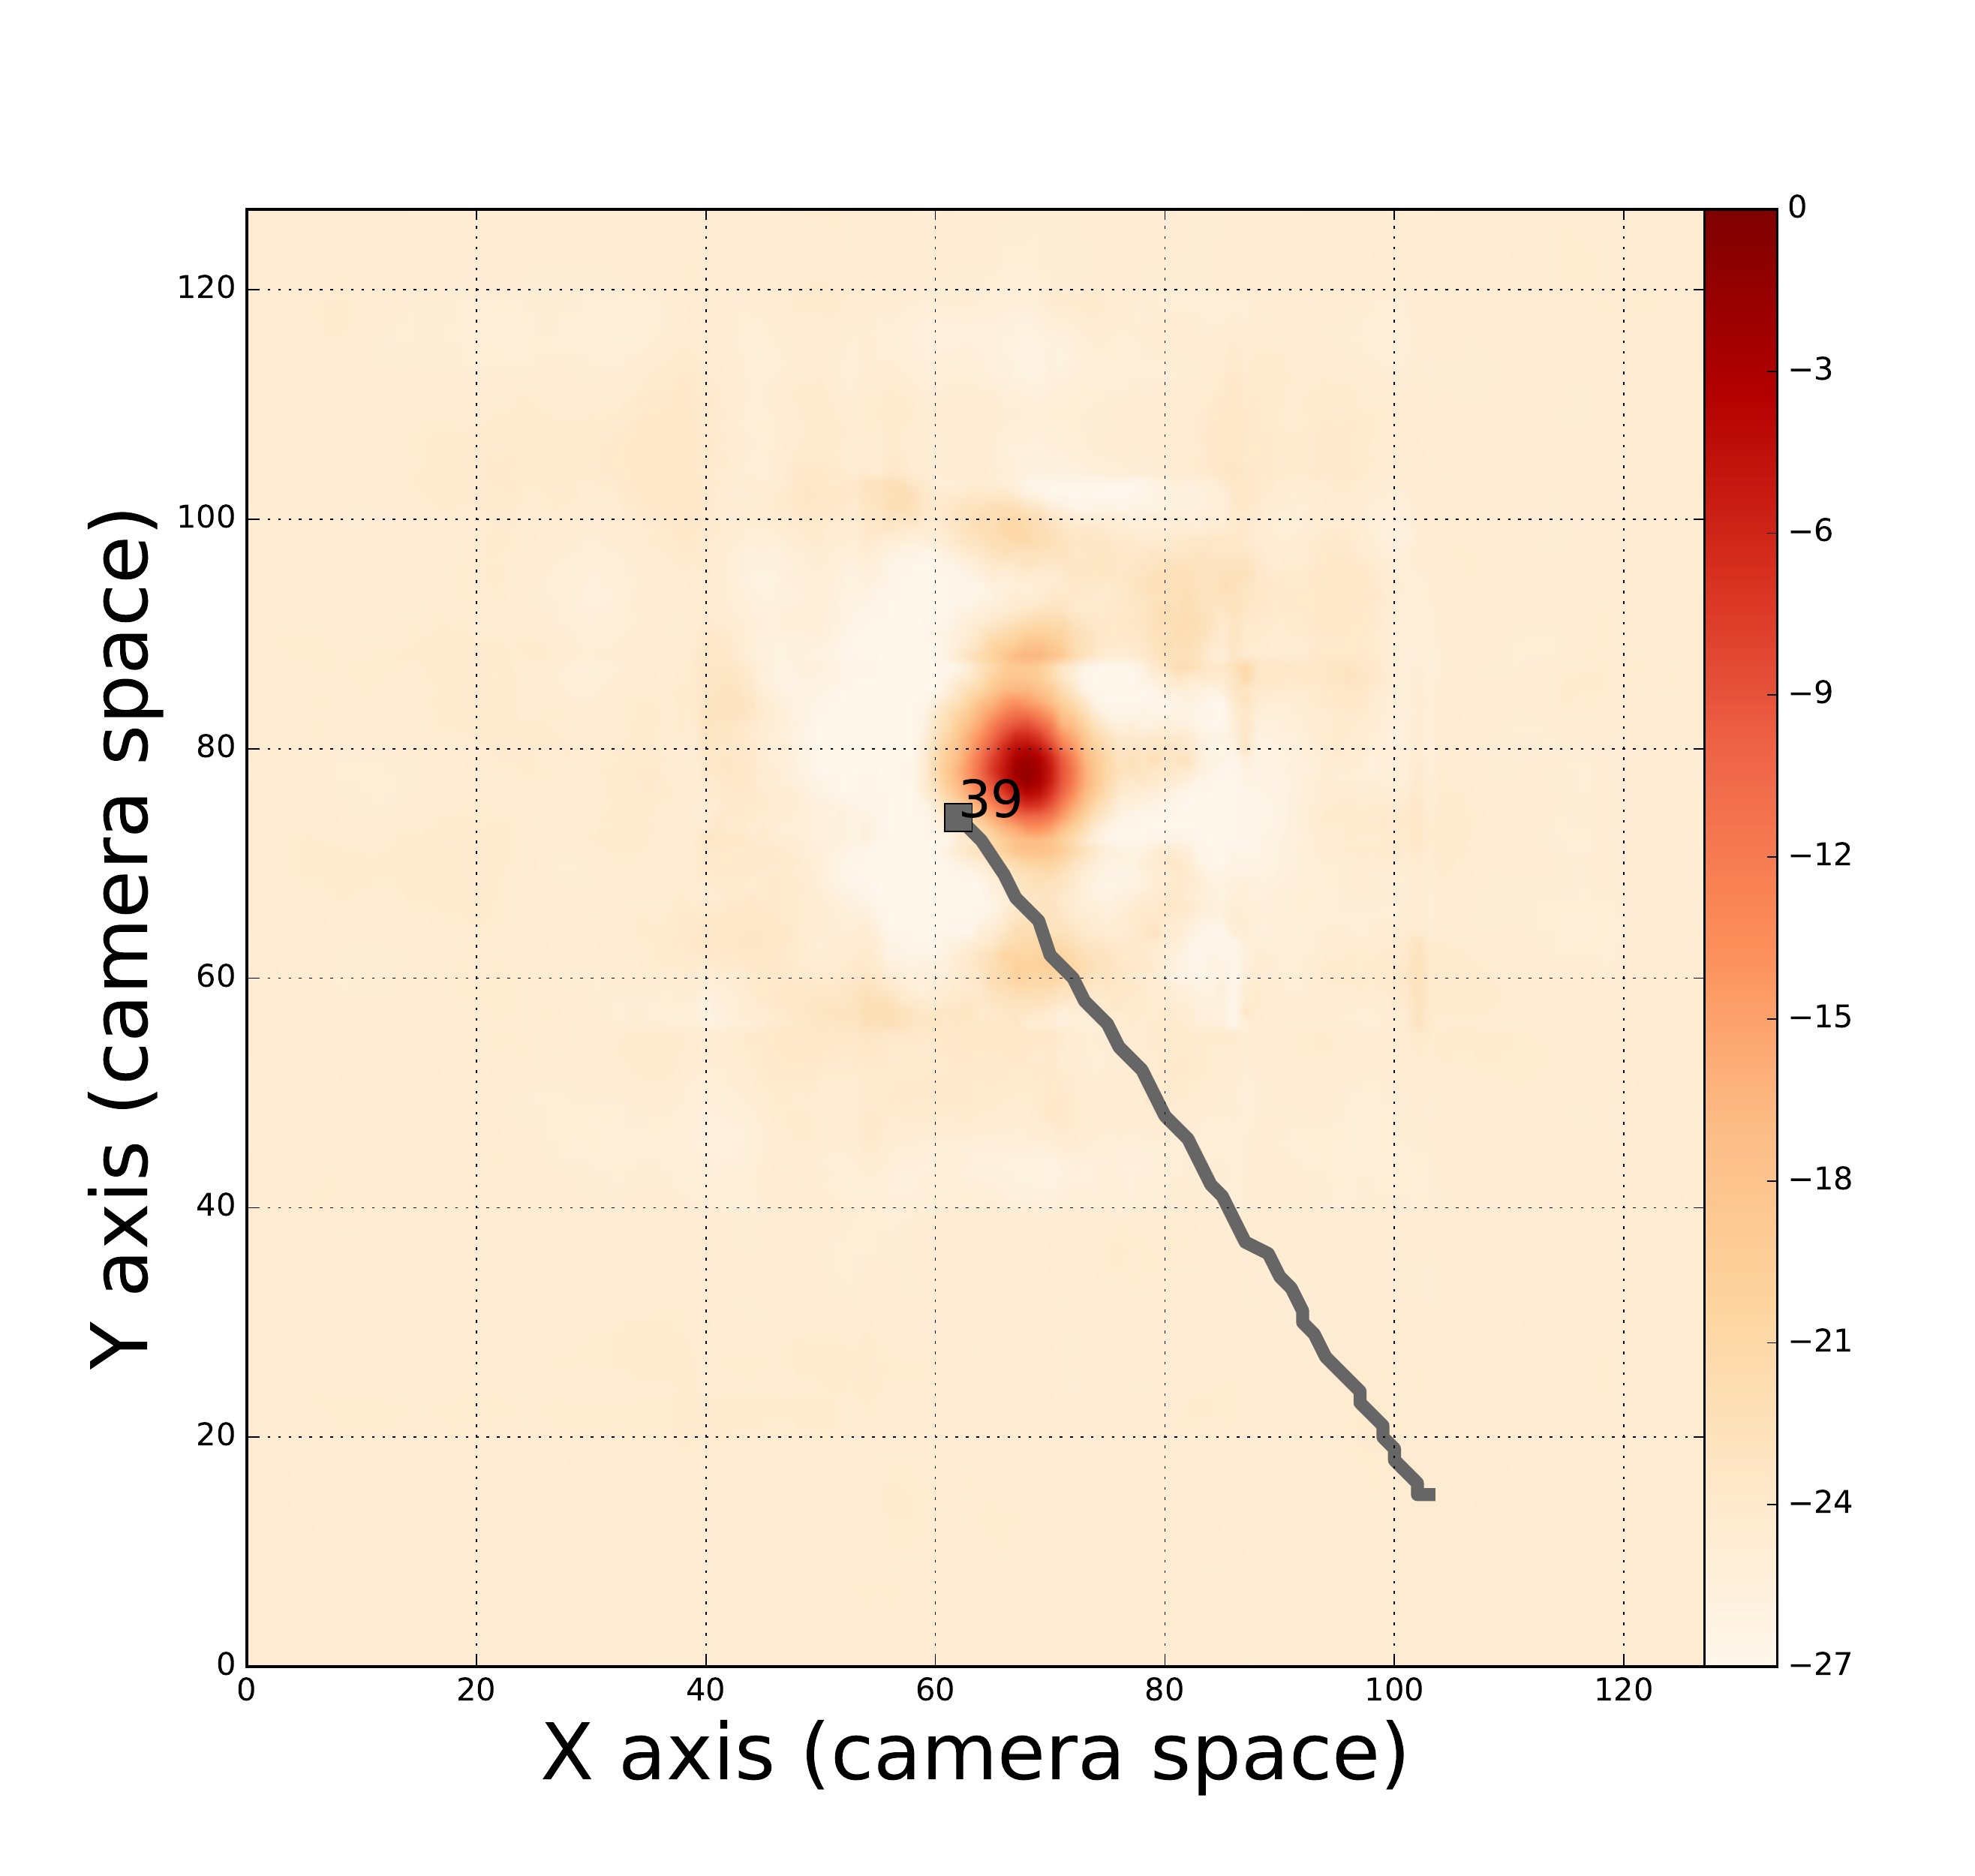}
\includegraphics[height=\rowheight]{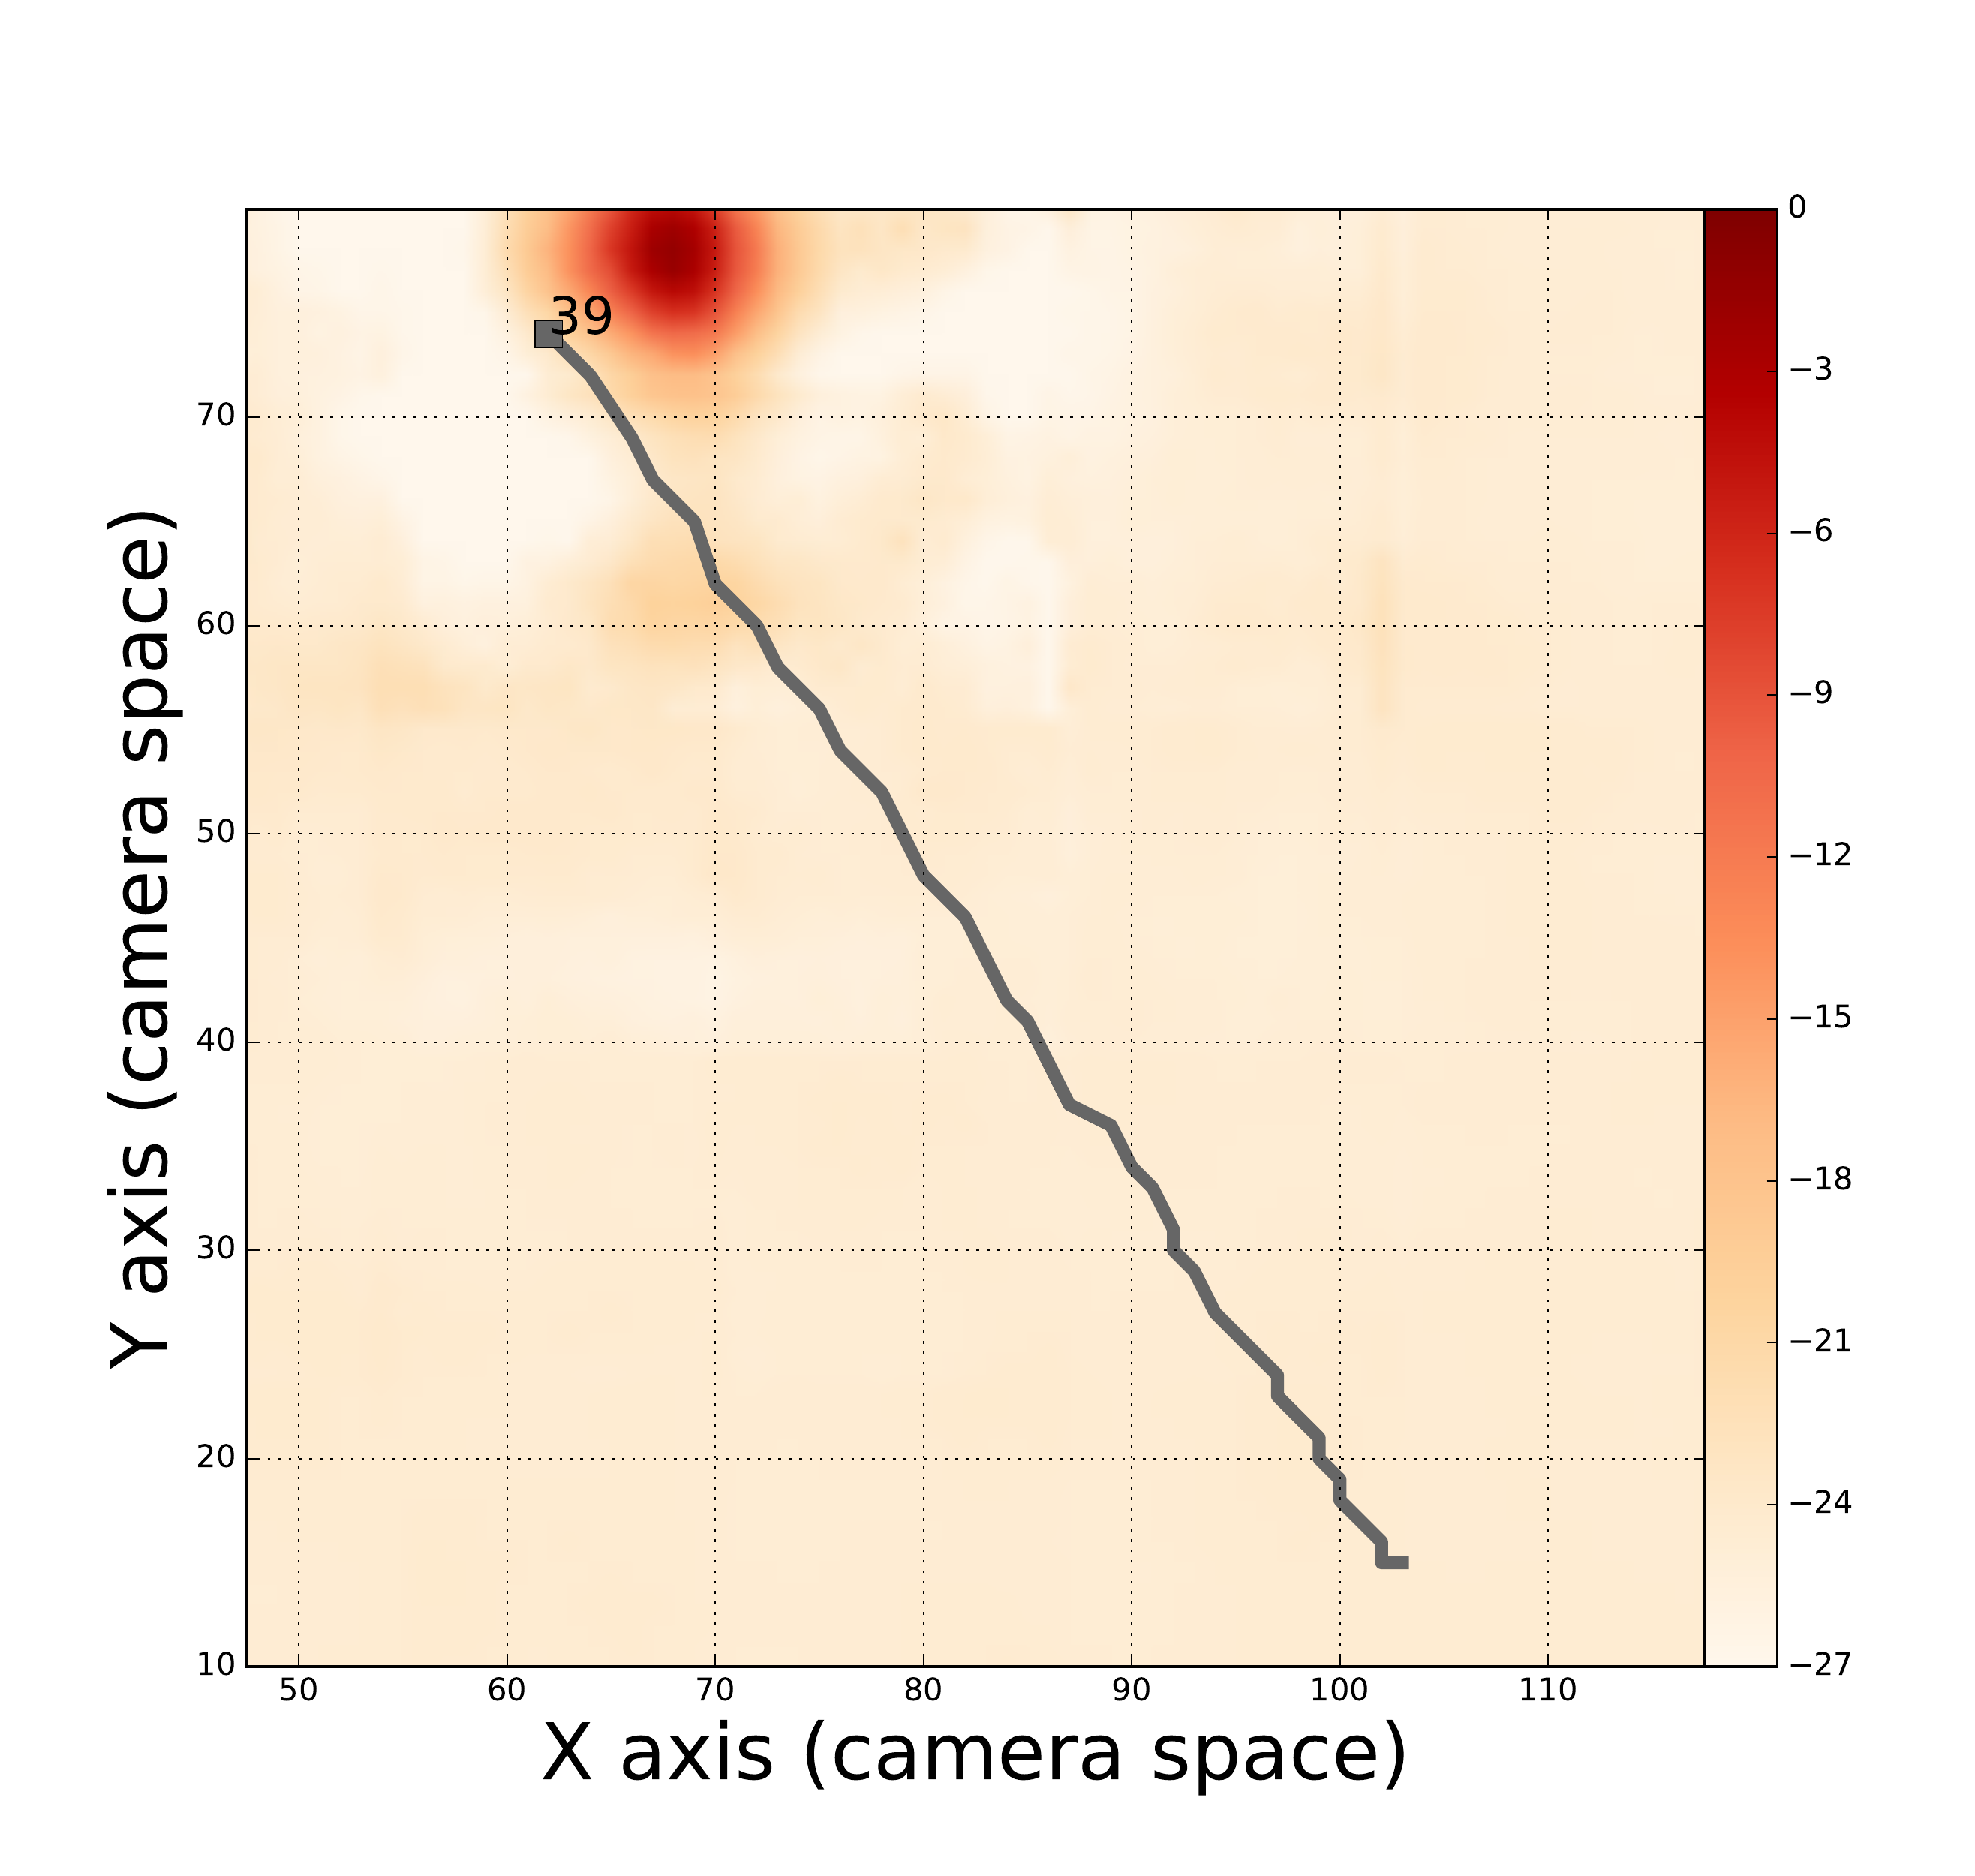}
\end{minipage}\\
\caption{Randomly chosen output experiment \#2}
\end{figure*}
\begin{figure*}[h]
\centering
\begin{minipage}[t]{\linewidth}
\includegraphics[height=\rowheight]{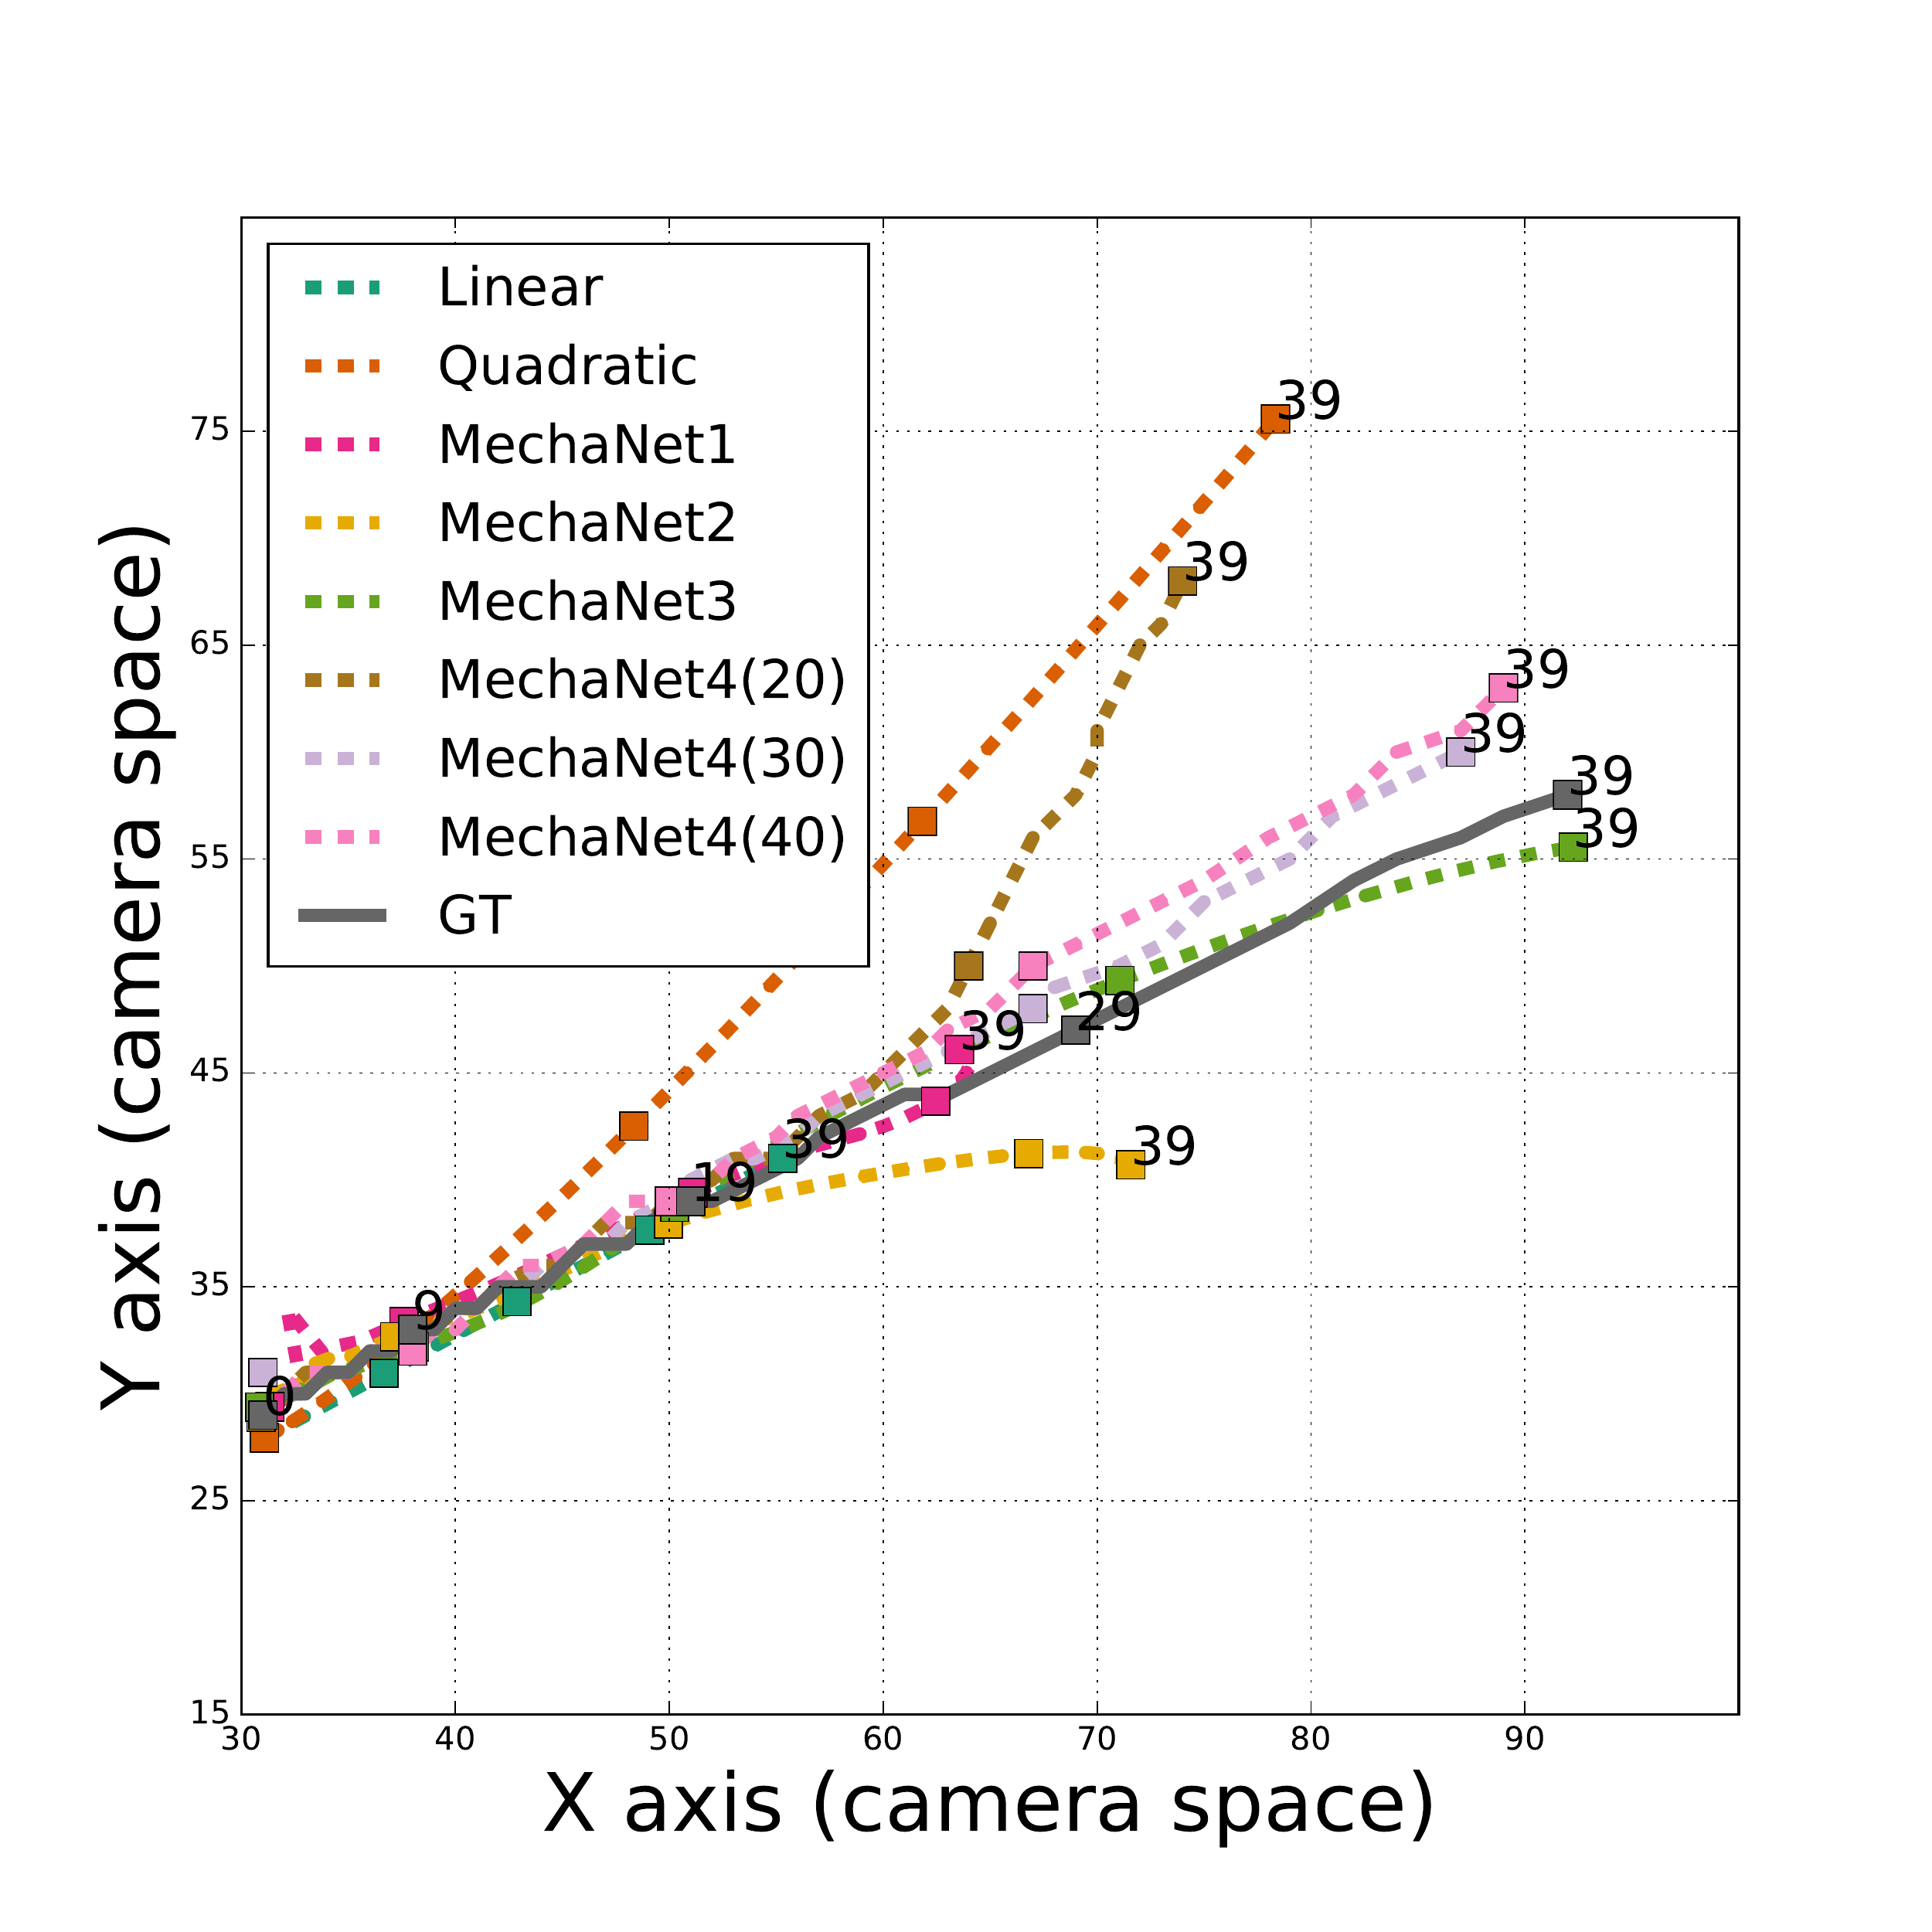}
\includegraphics[height=\rowheight]{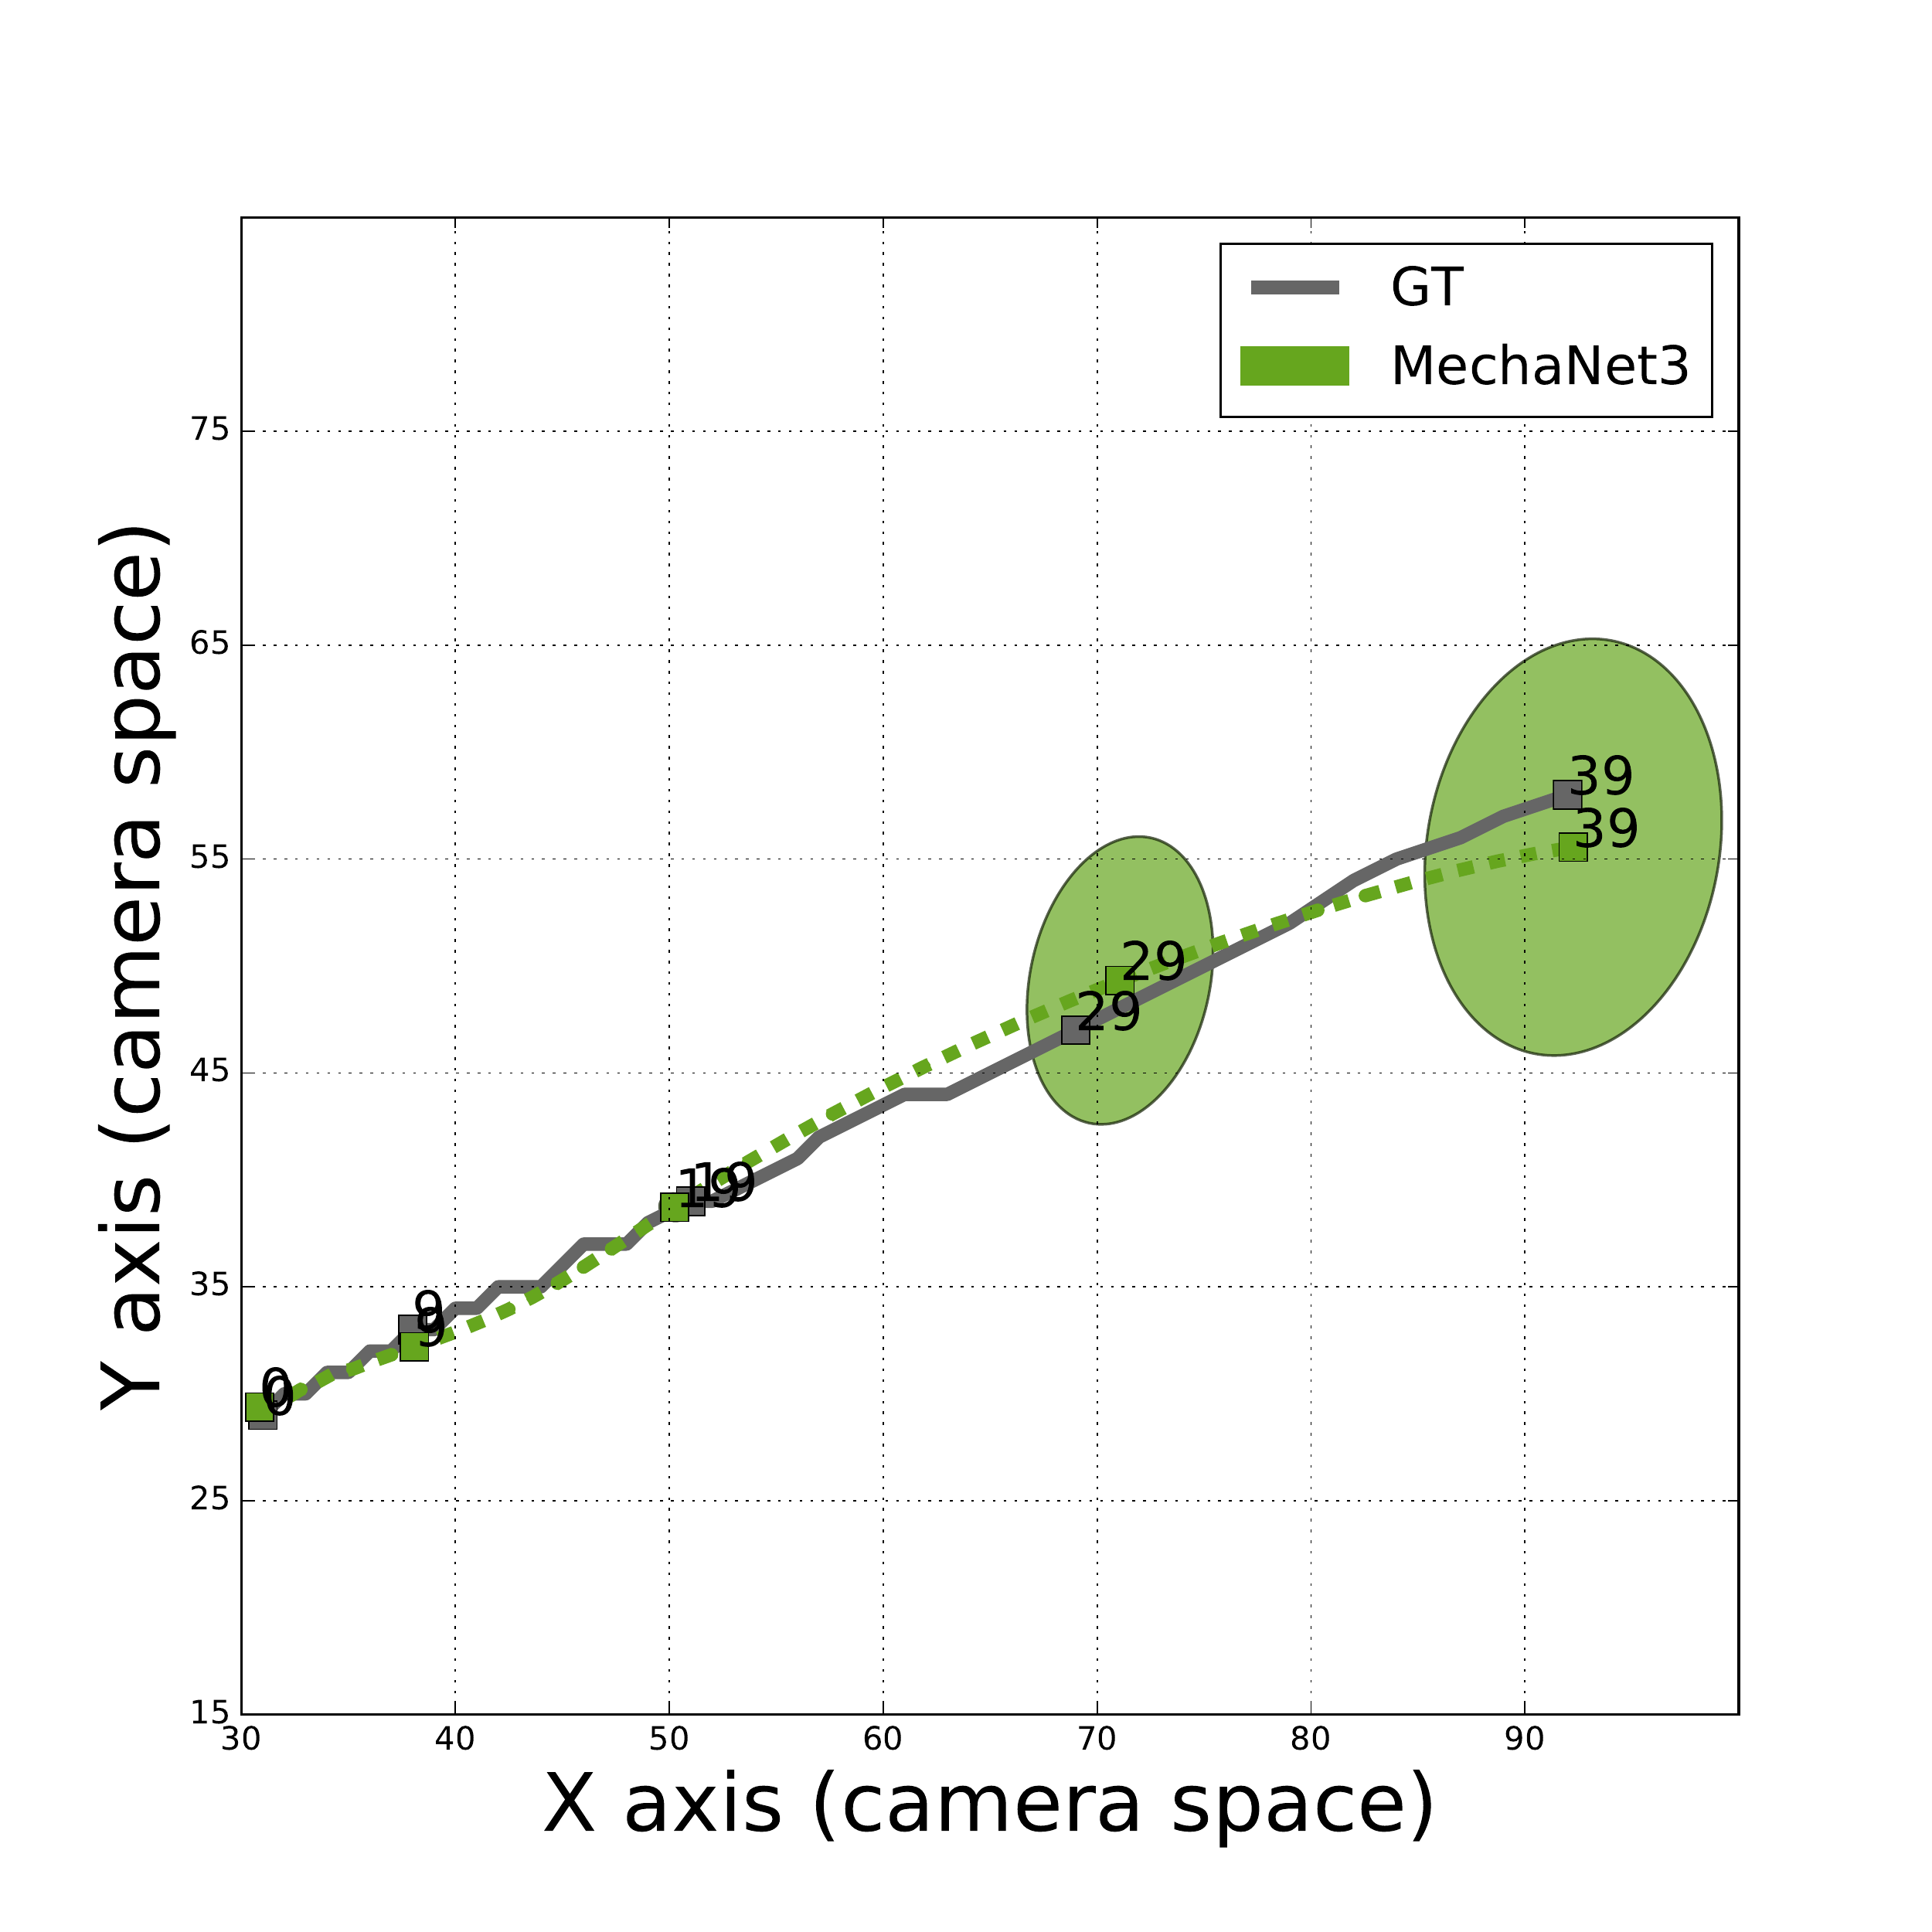}
\includegraphics[height=\rowheight]{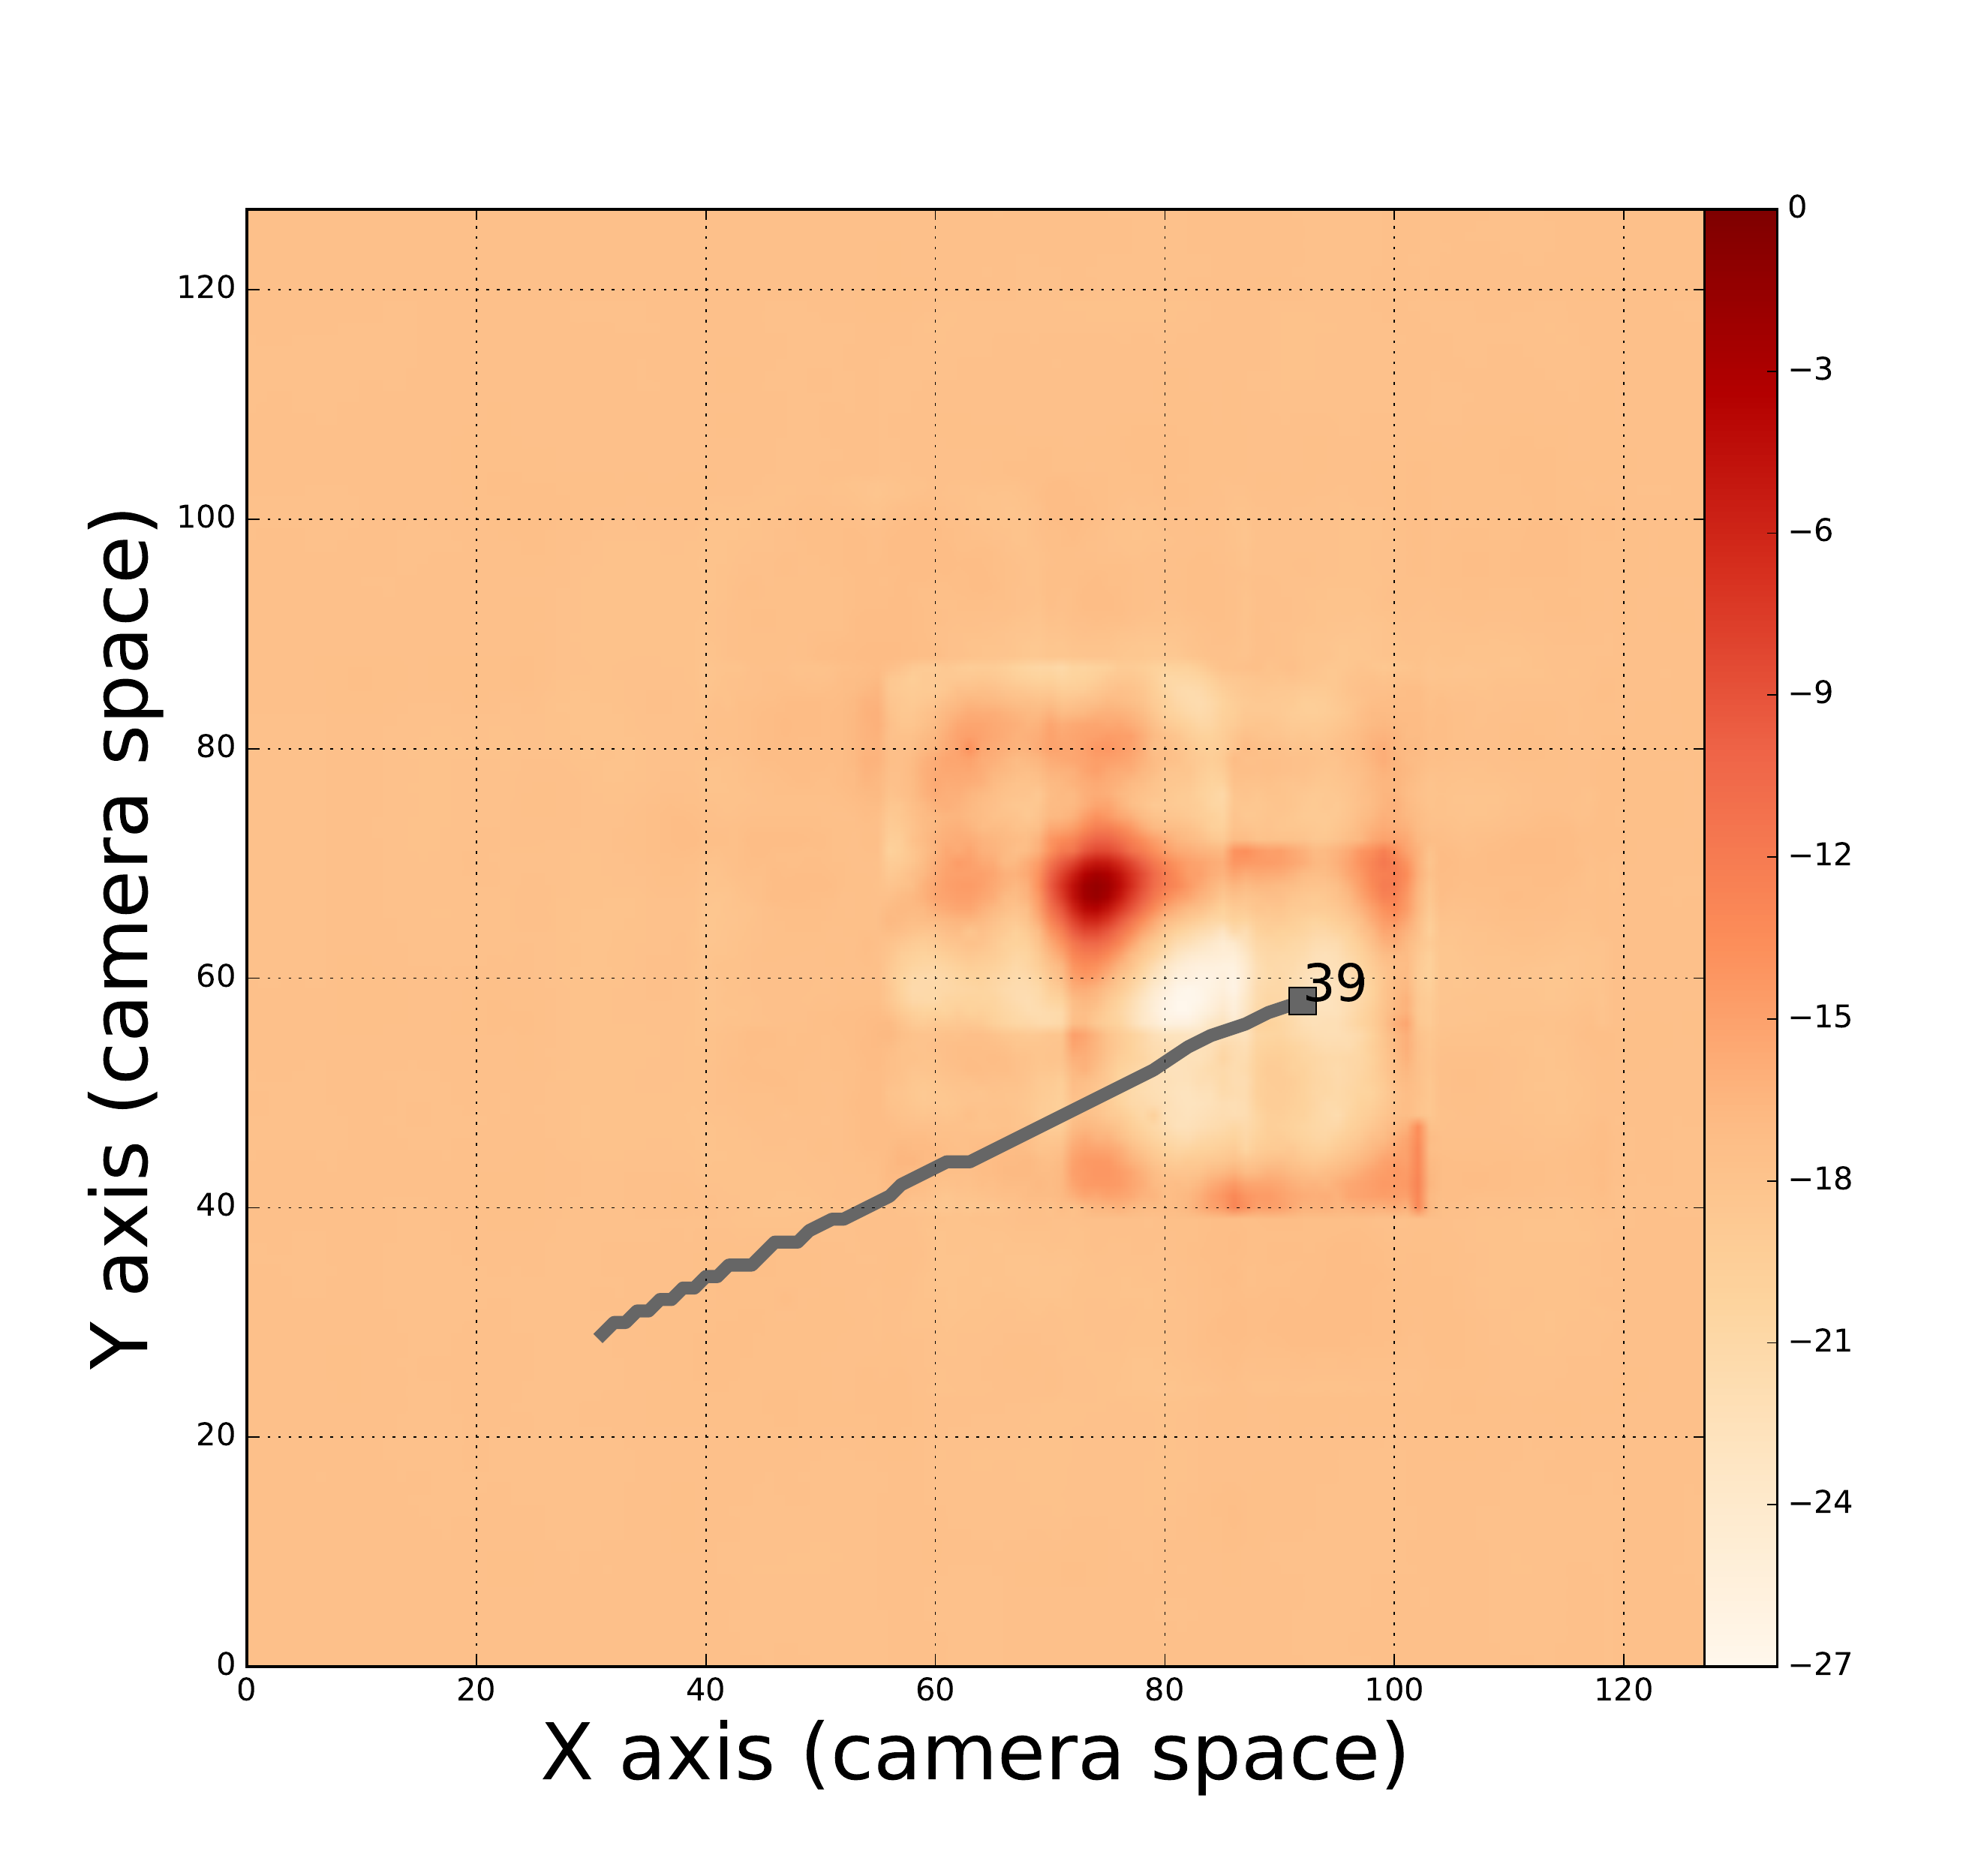}
\includegraphics[height=\rowheight]{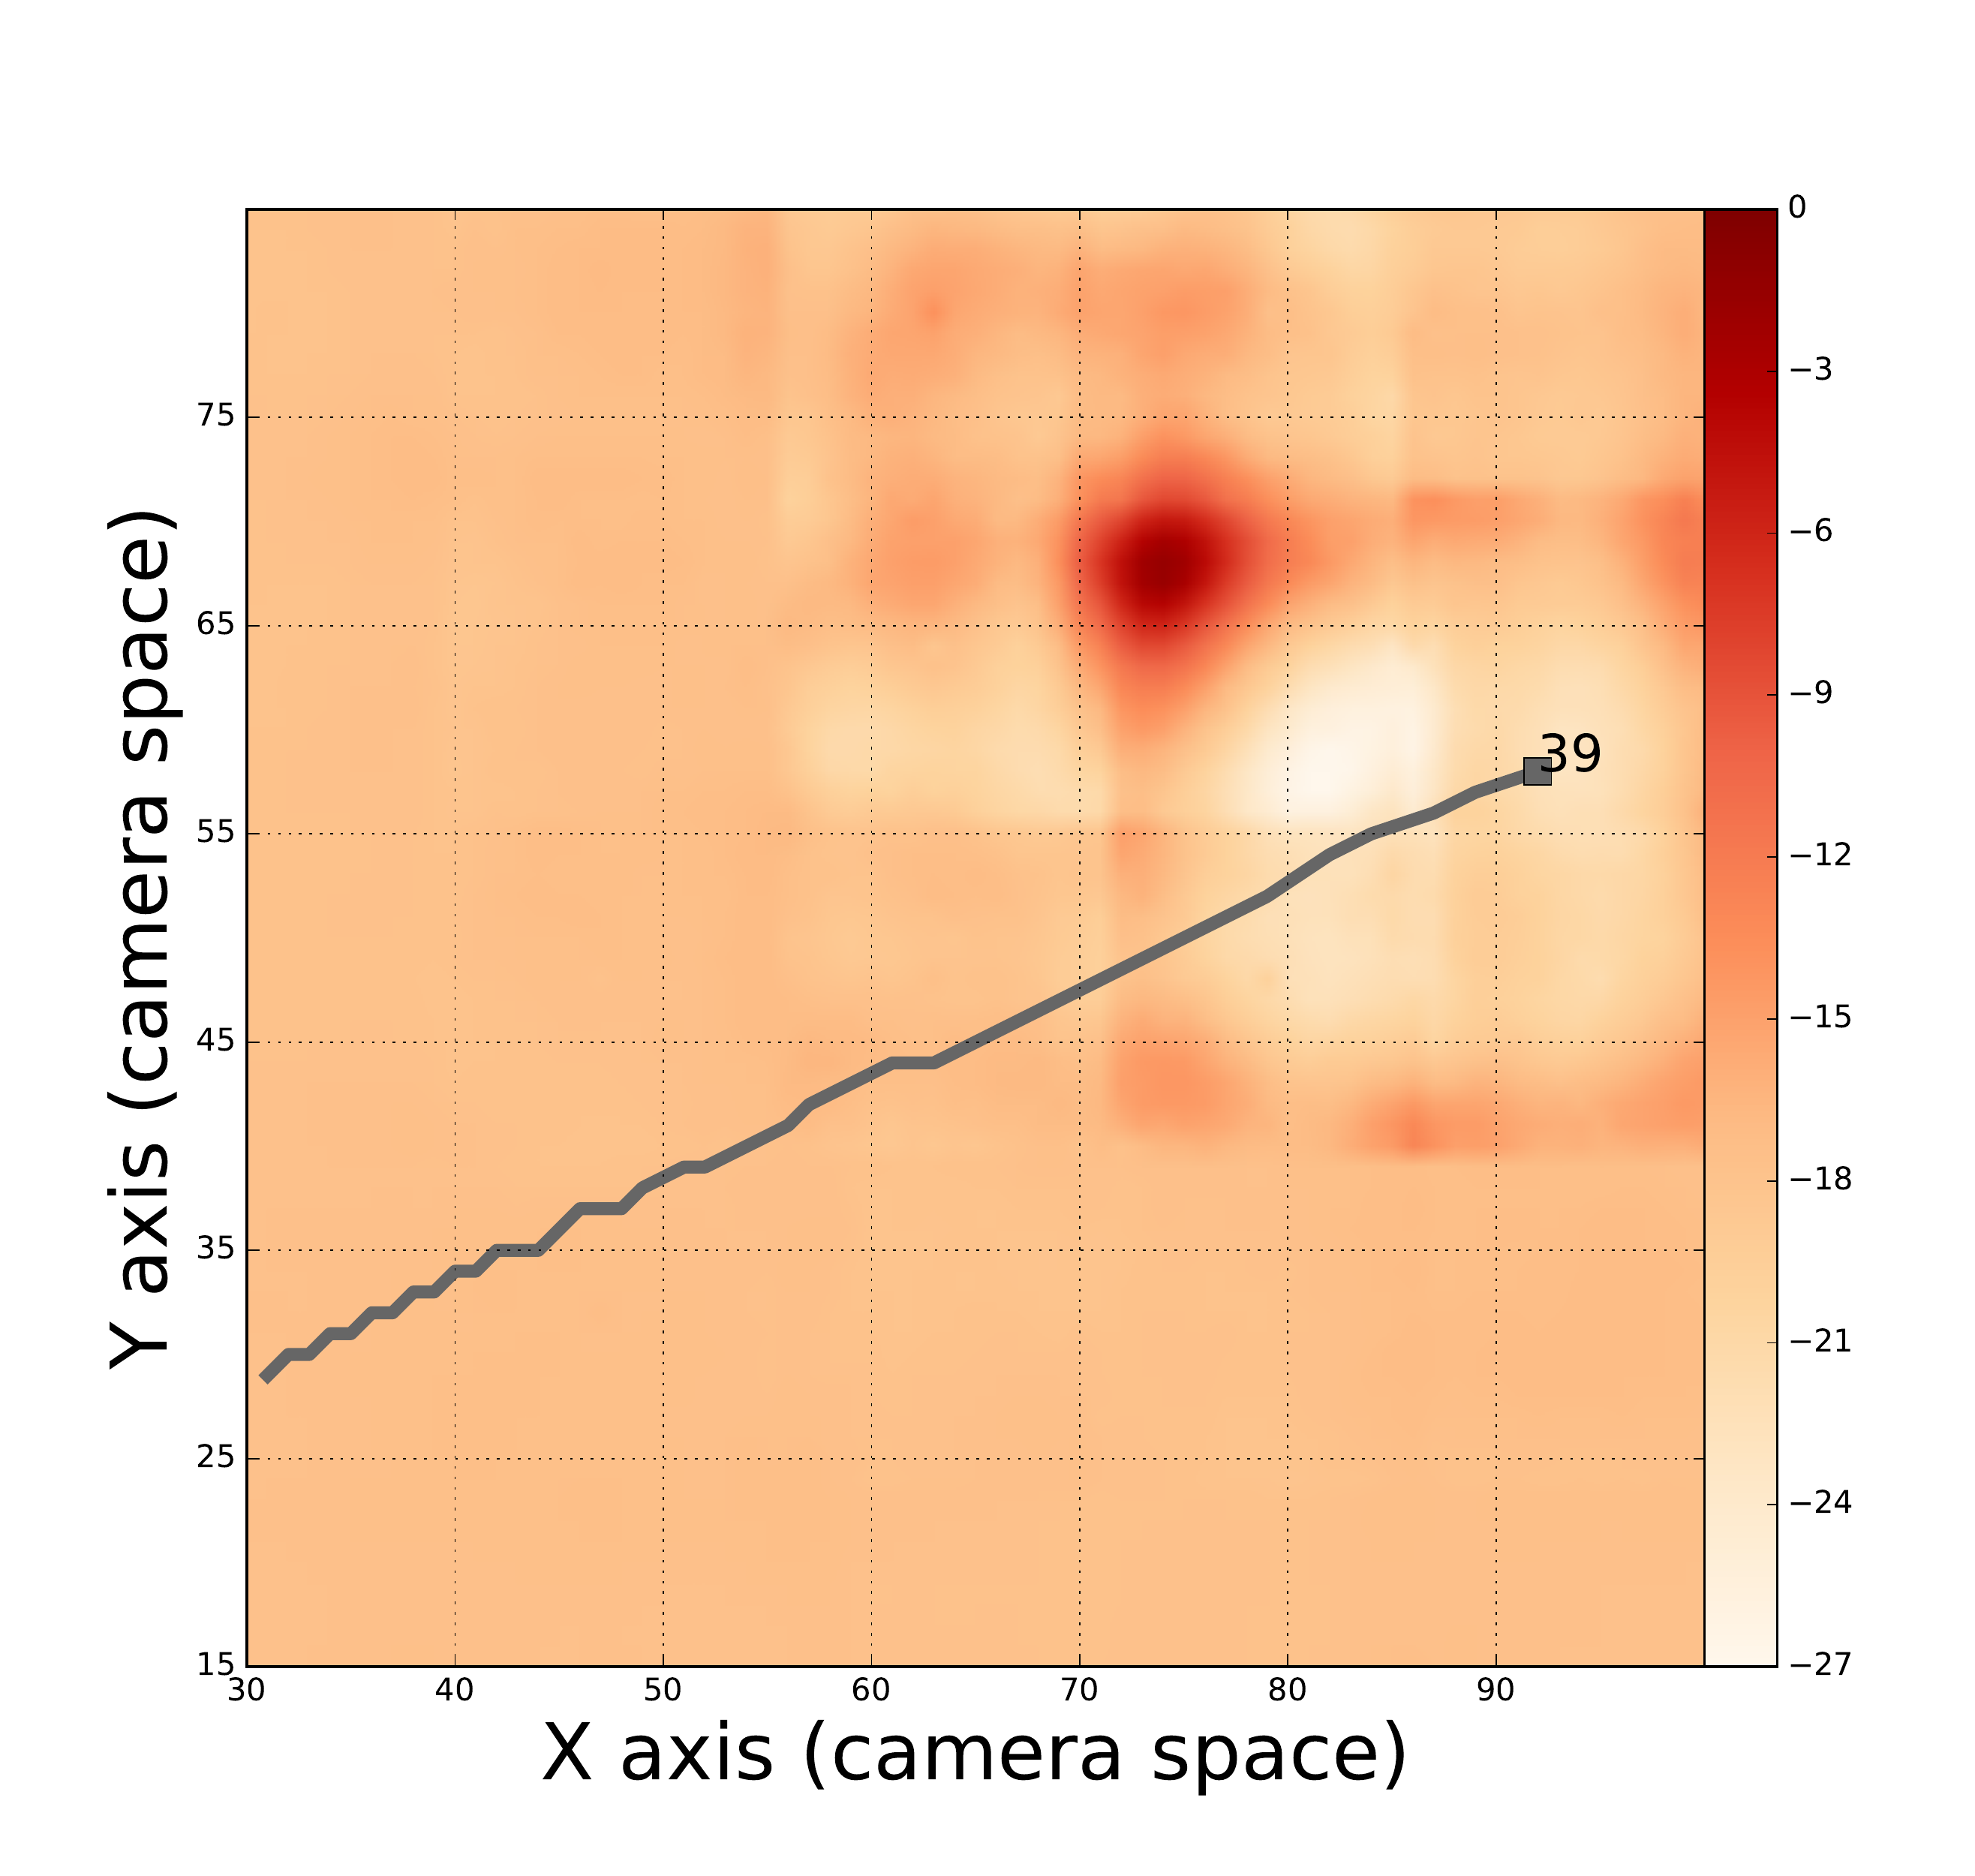}
\includegraphics[height=\rowheight]{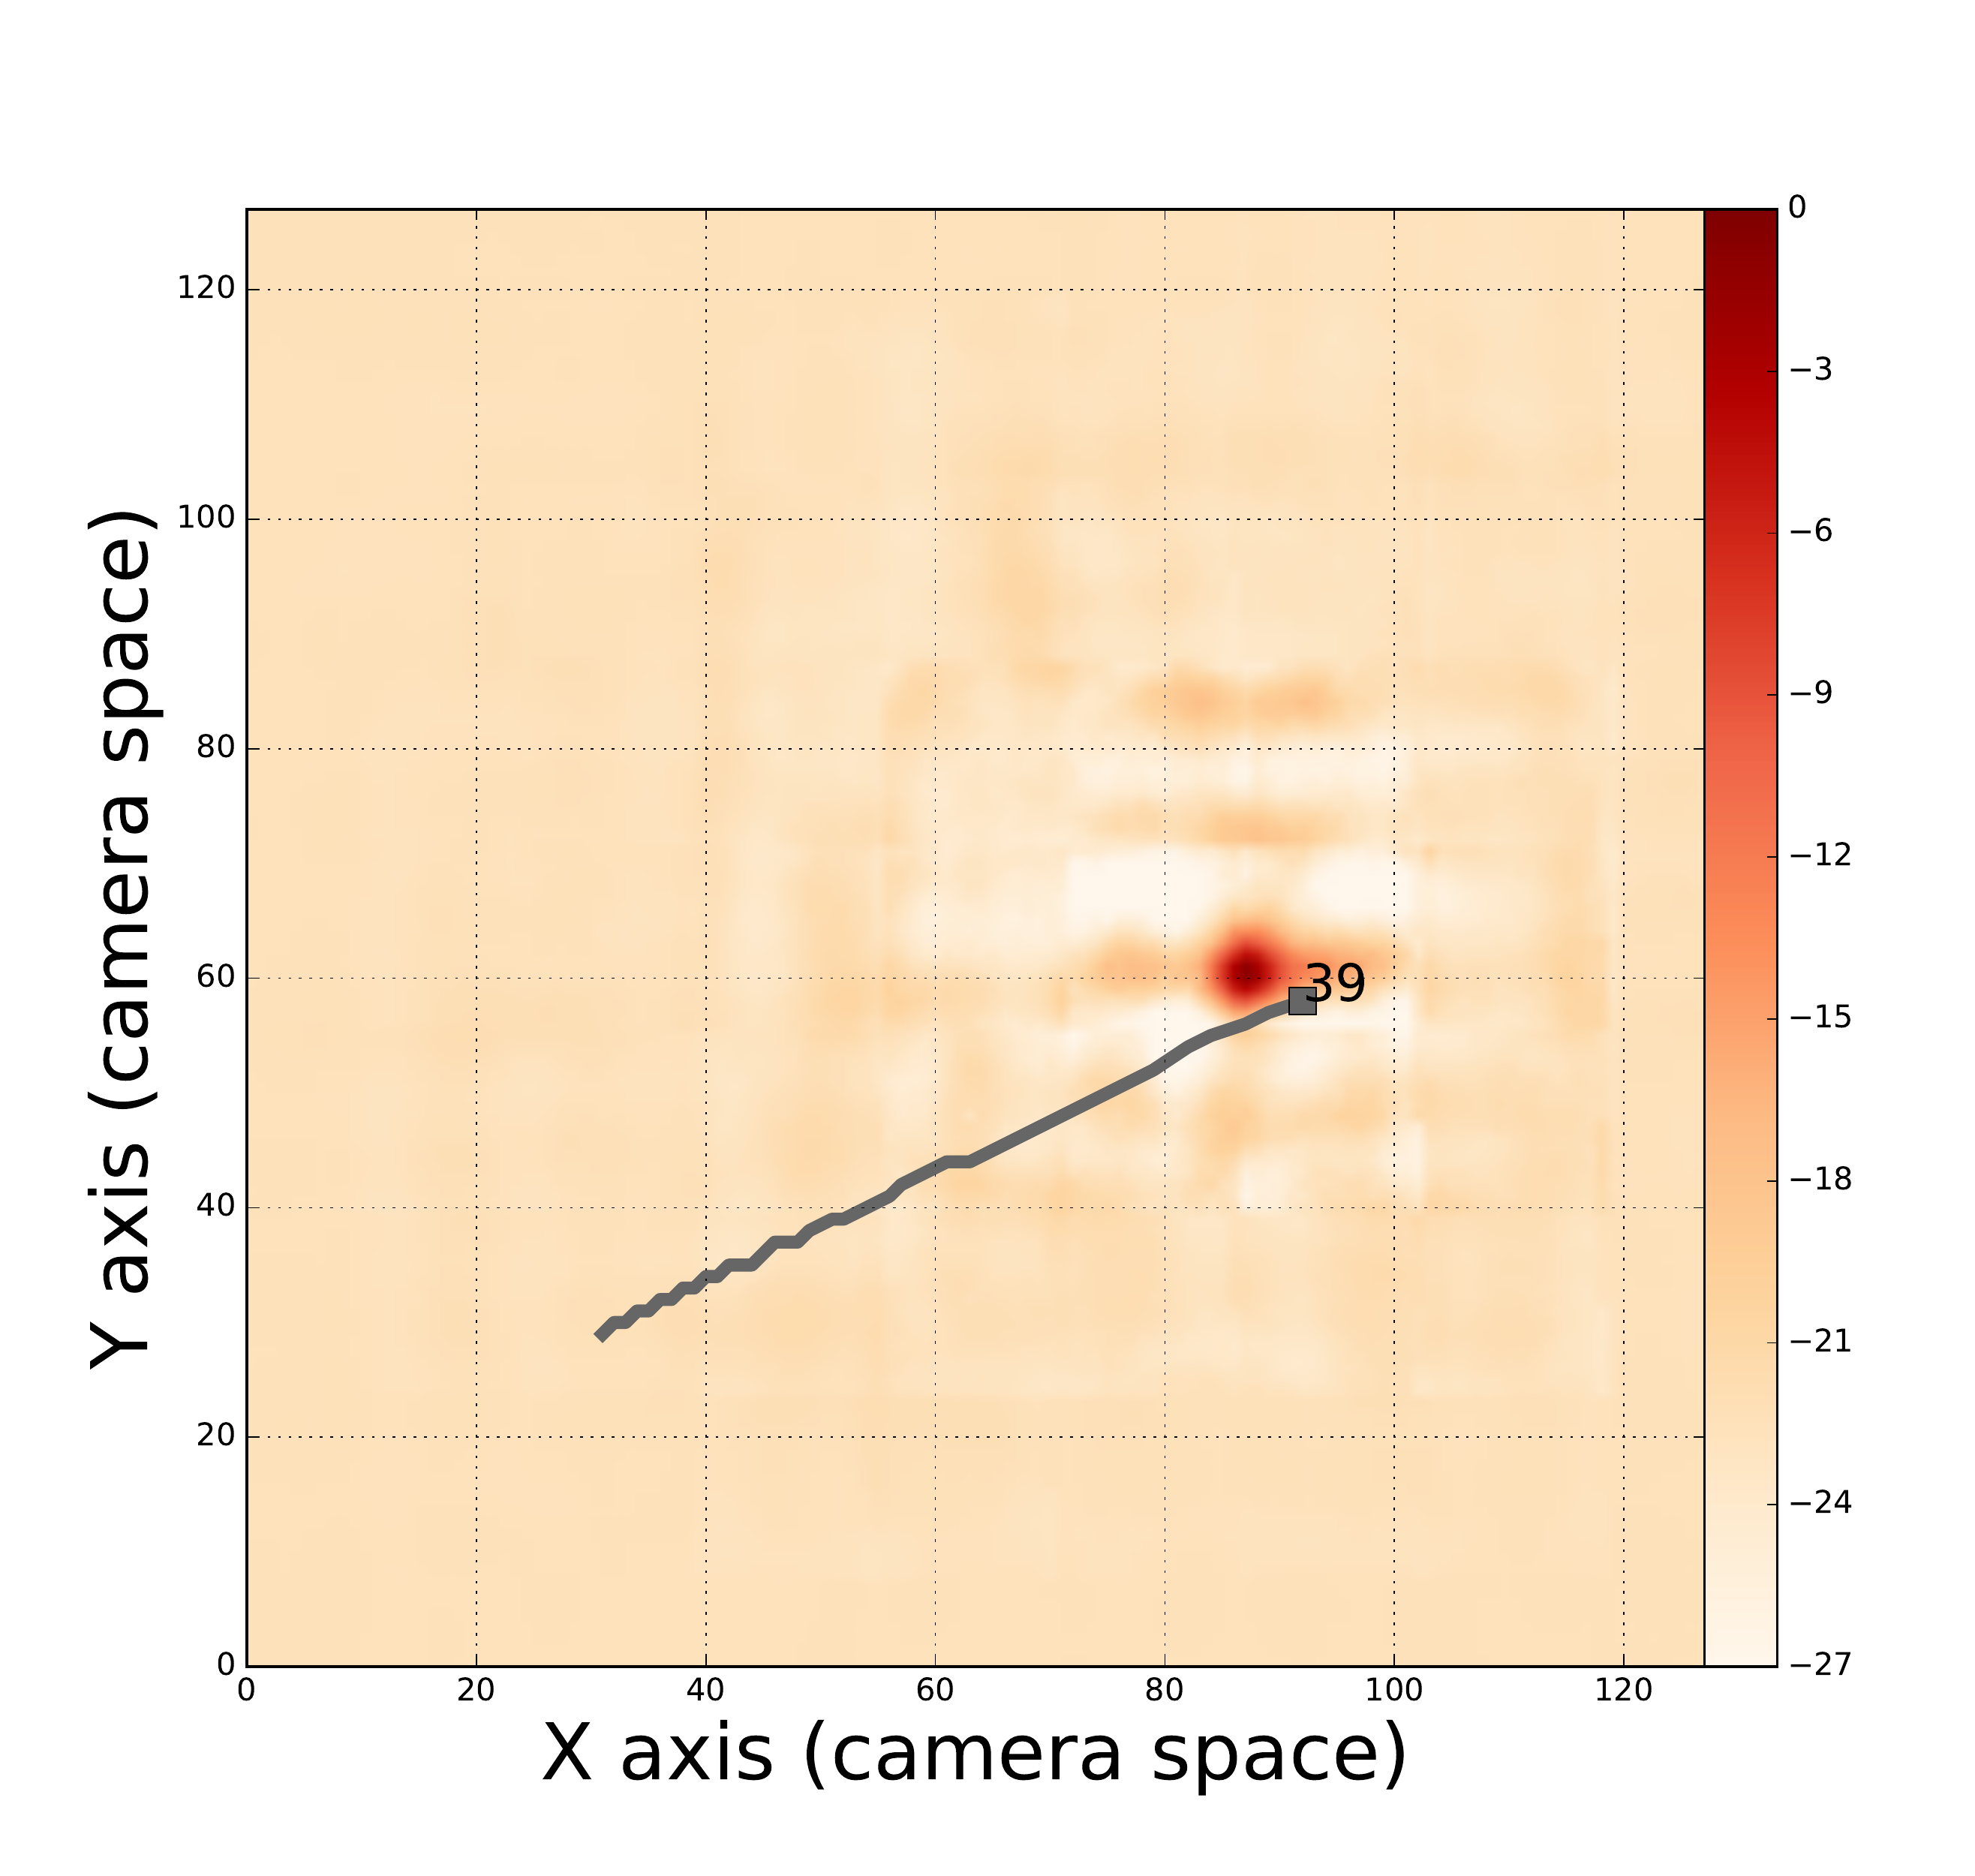}
\includegraphics[height=\rowheight]{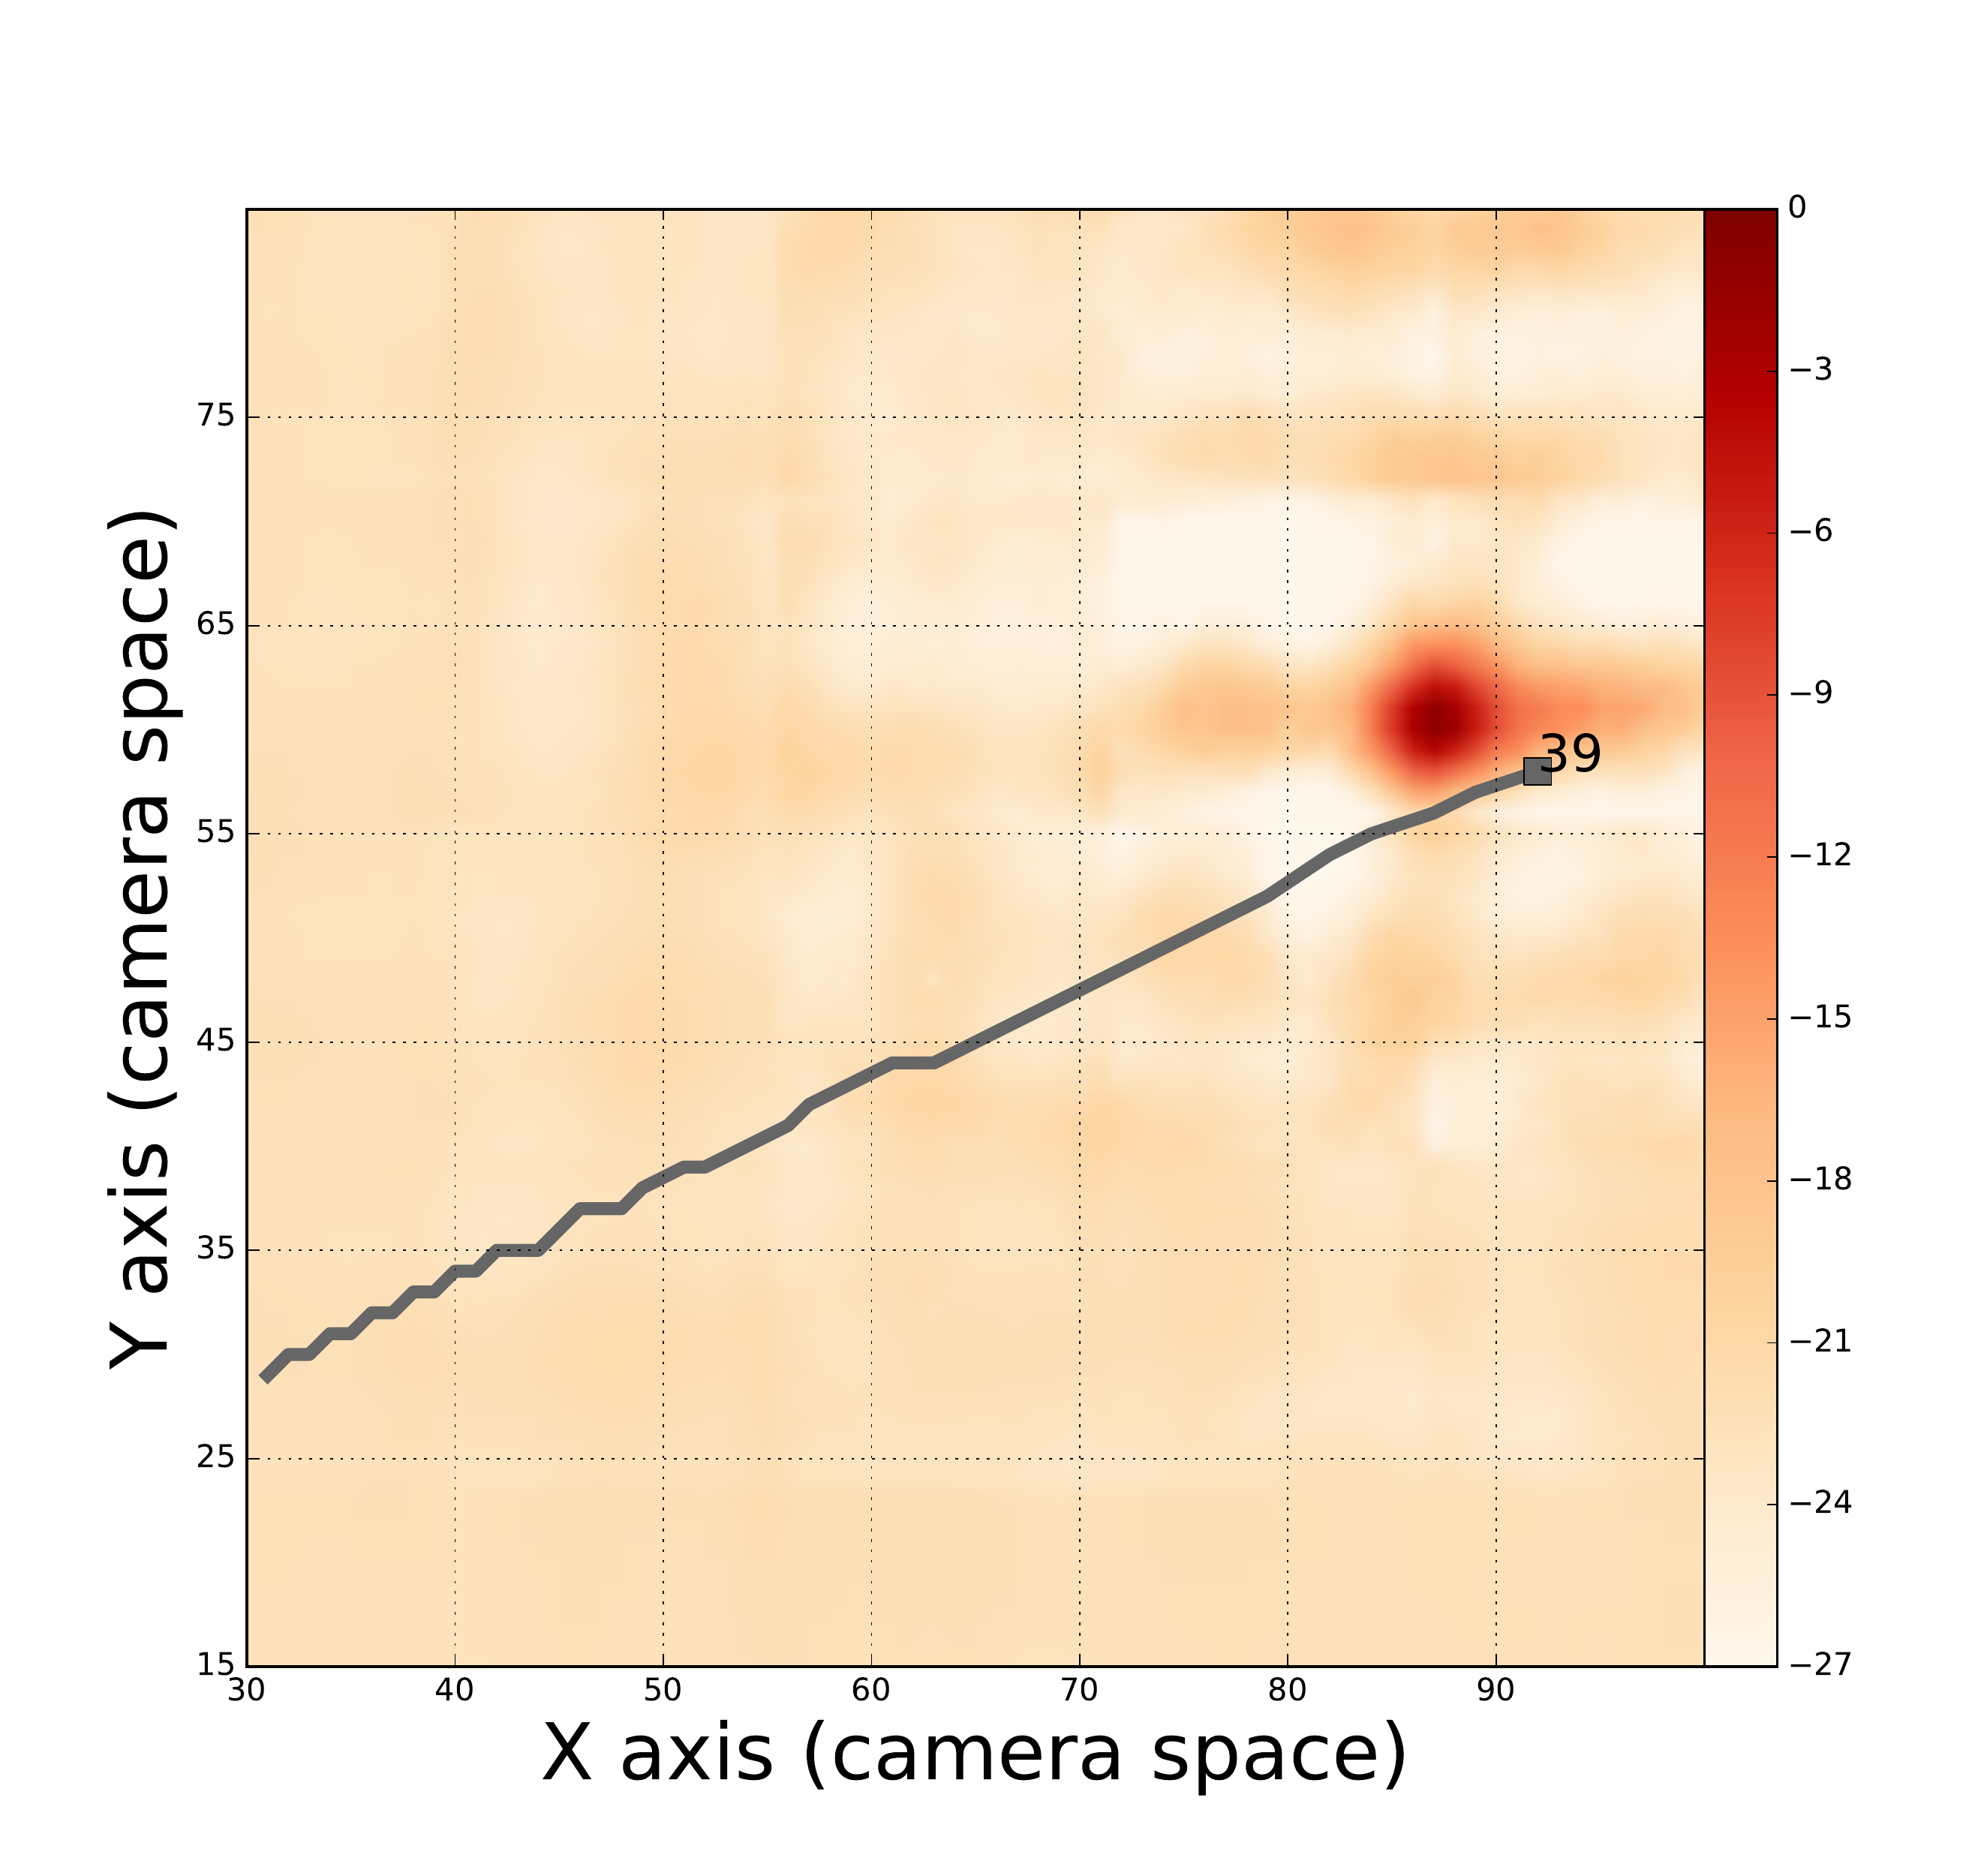}
\includegraphics[height=\rowheight]{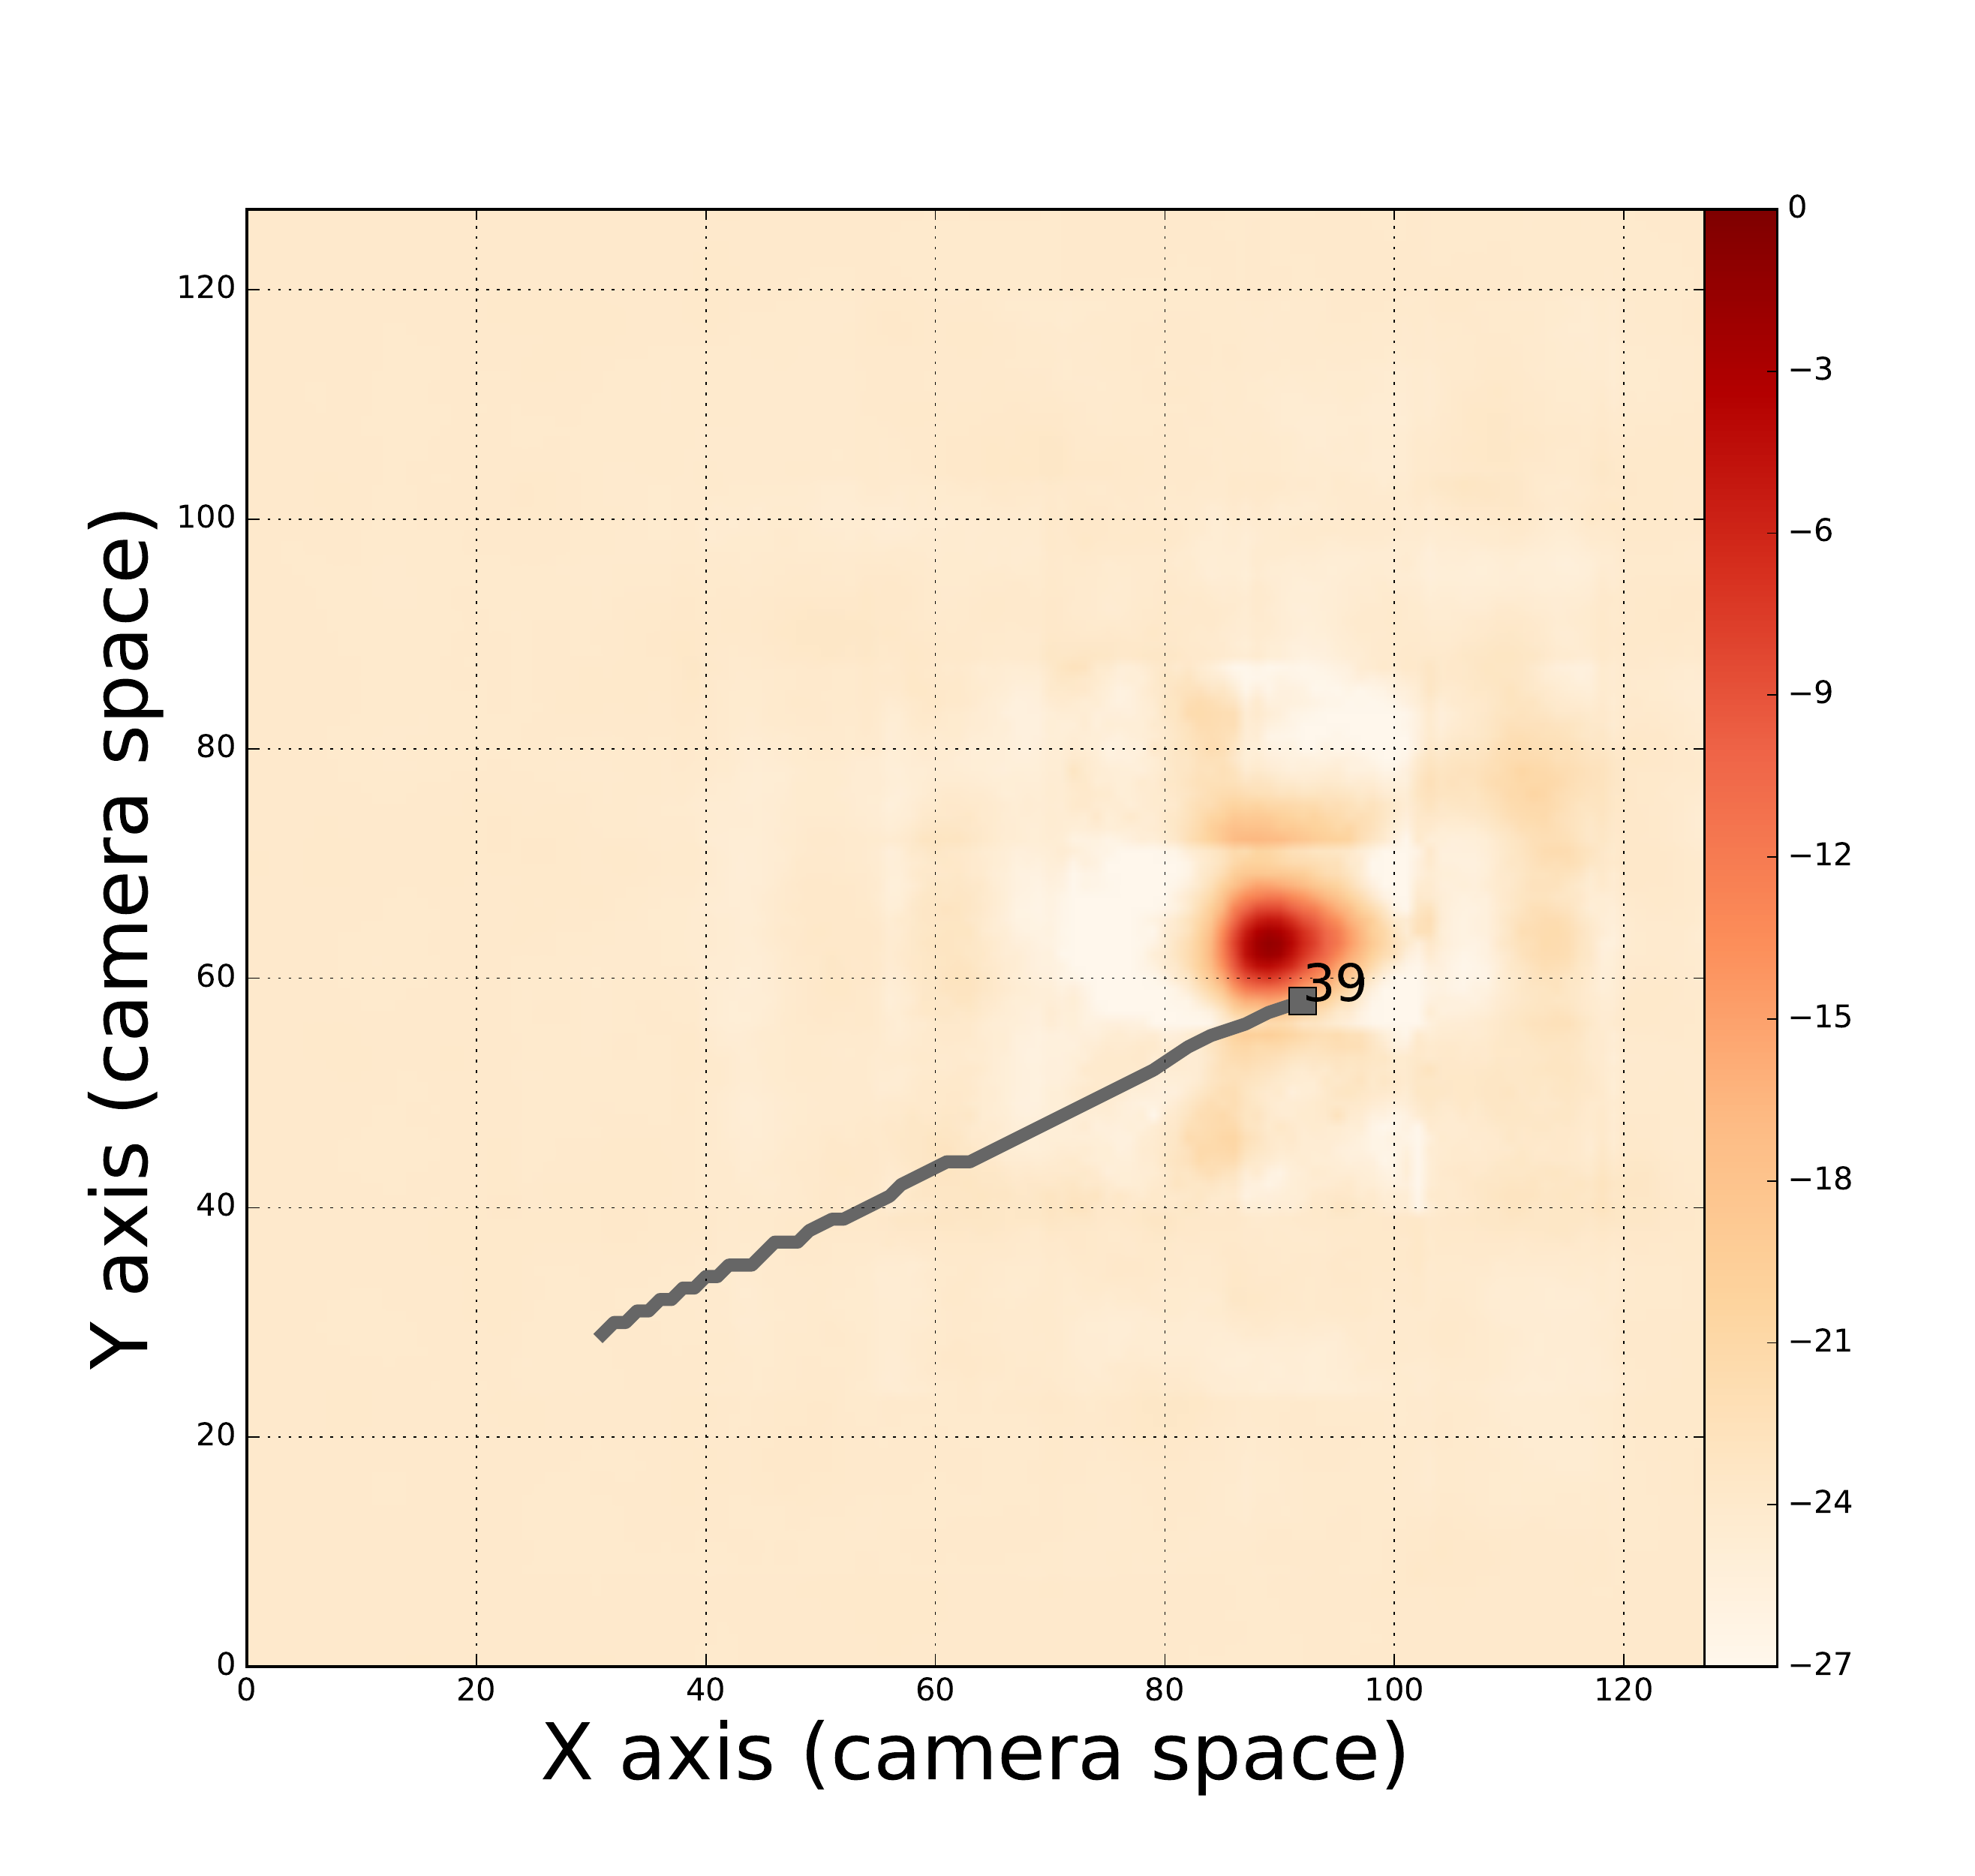}
\includegraphics[height=\rowheight]{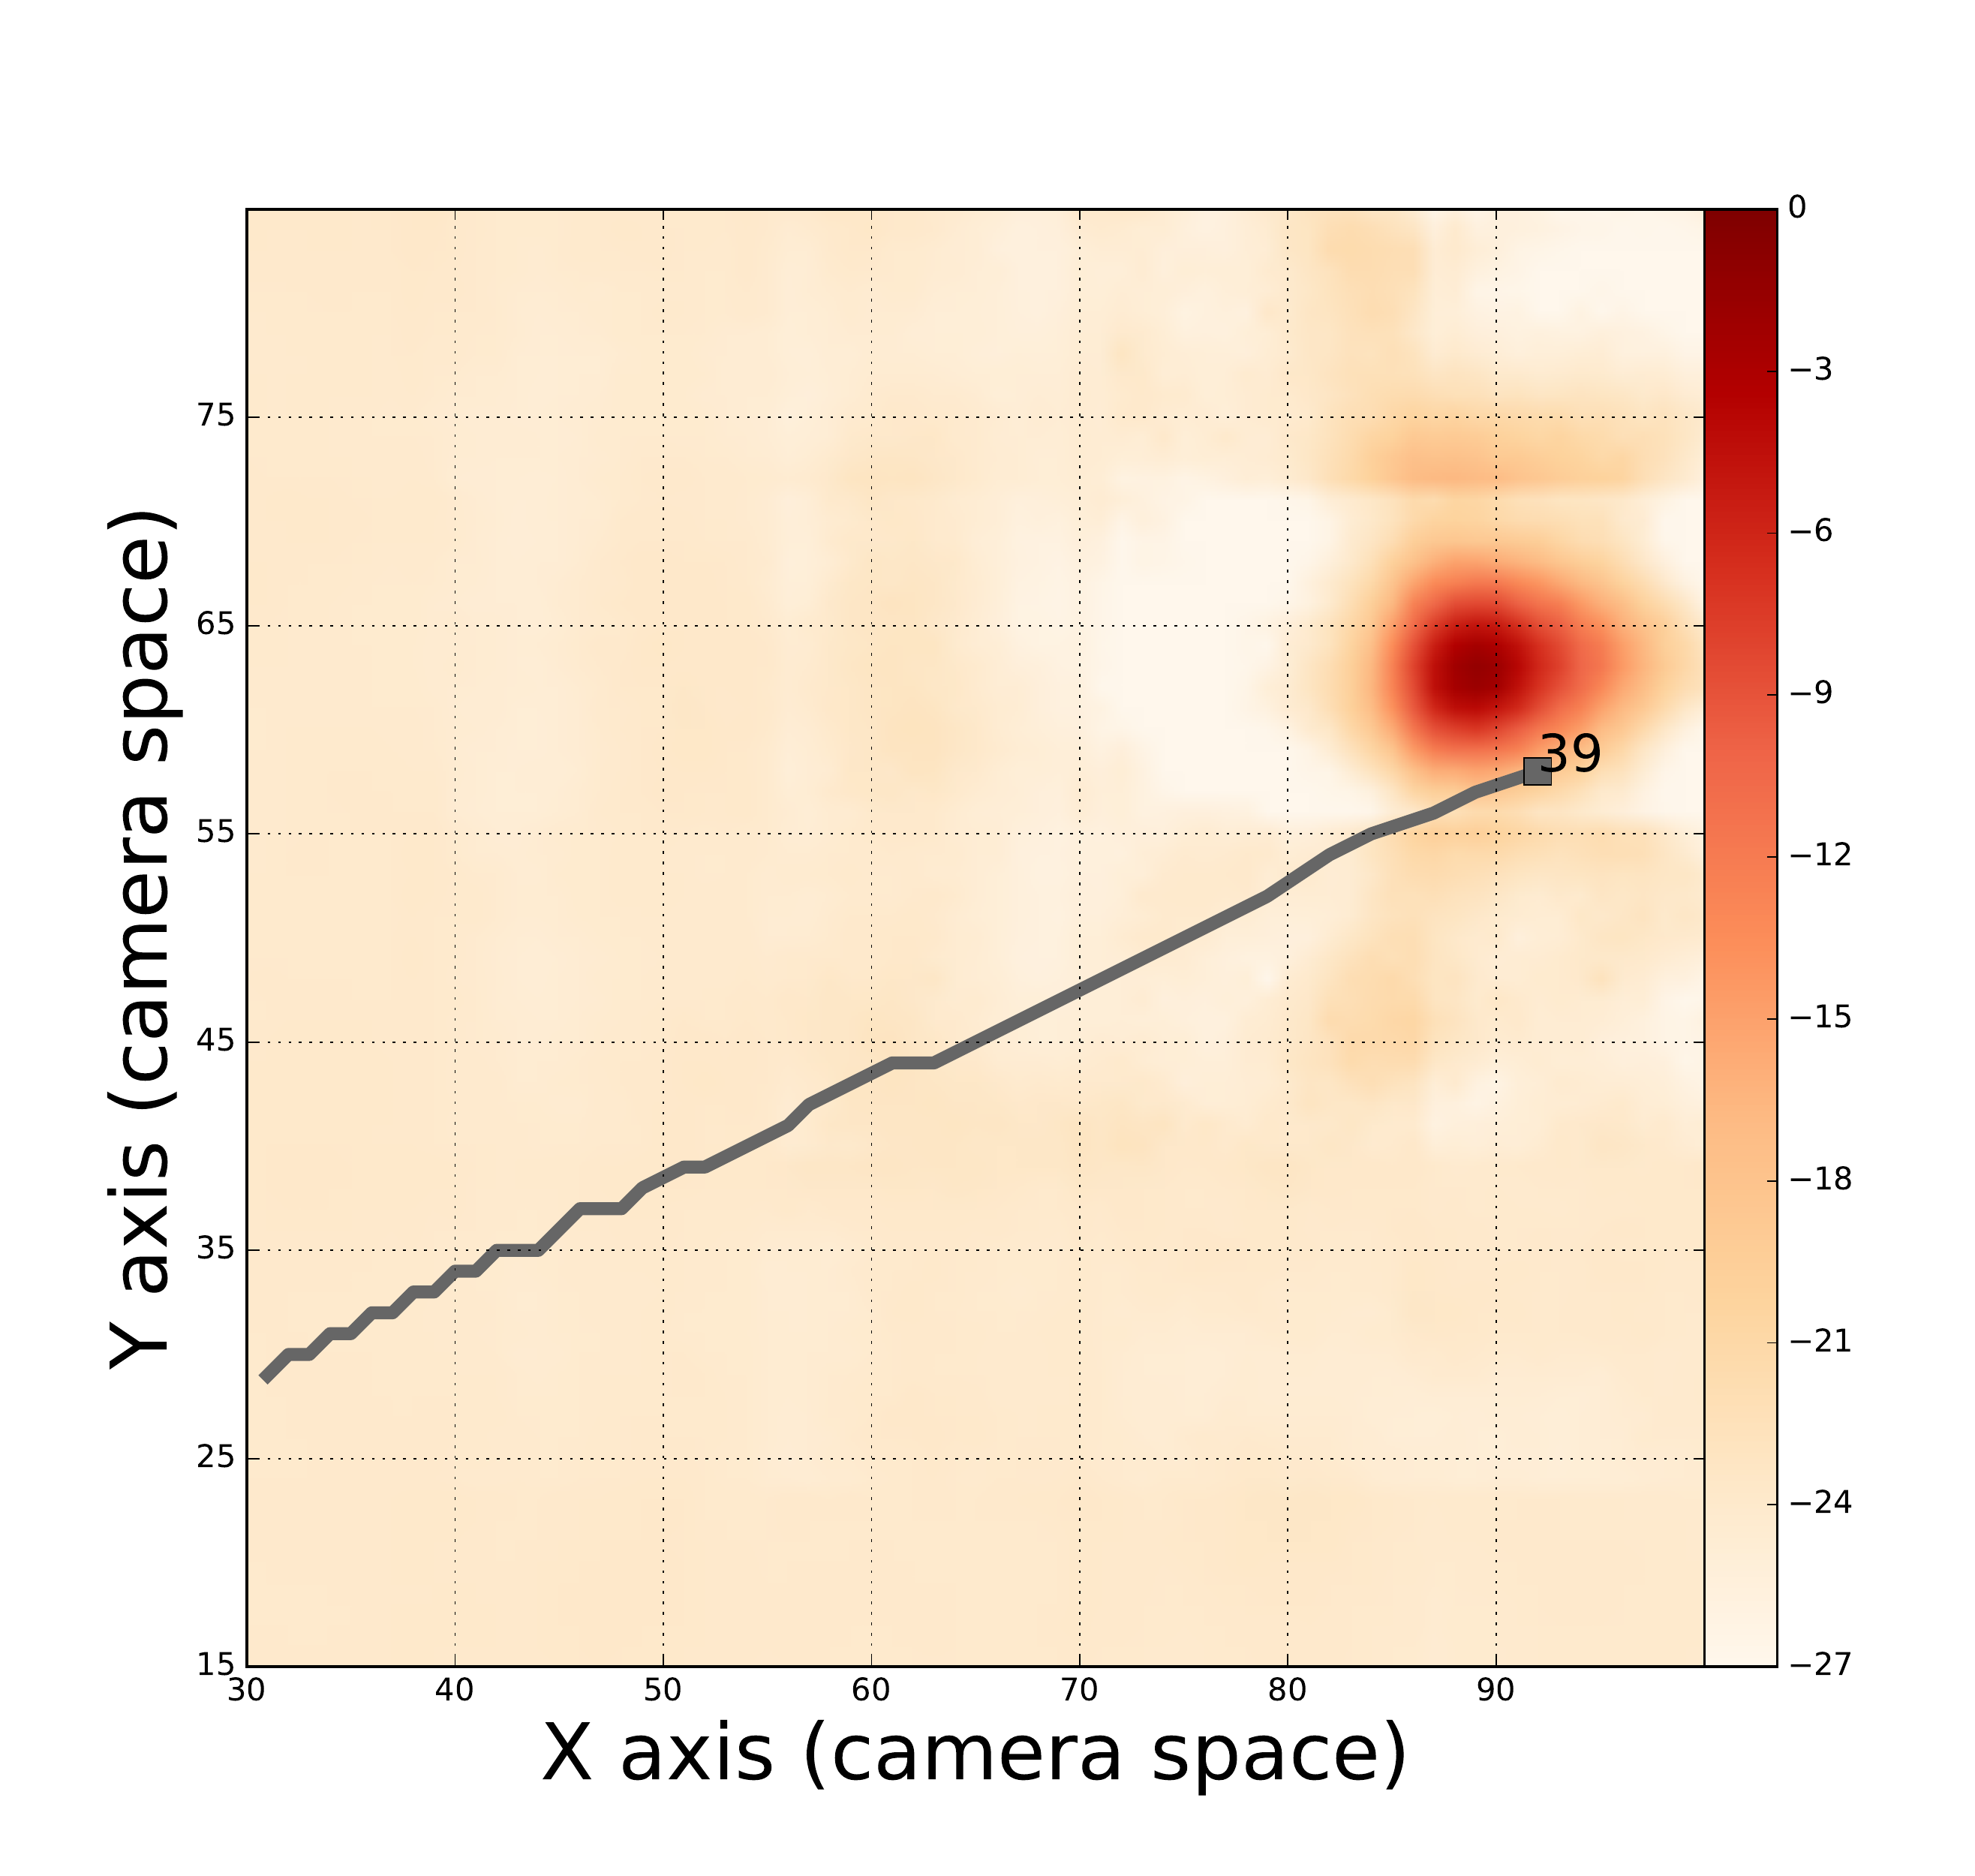}
\end{minipage}\\
\caption{Randomly chosen output experiment \#3}
\end{figure*}
\begin{figure*}[h]
\centering
\begin{minipage}[t]{\linewidth}
\includegraphics[height=\rowheight]{images/results/S1_samples/S1_04_time_40.pdf}
\includegraphics[height=\rowheight]{images/results/S1_samples/S1_04_time_40_ellipses.pdf}
\includegraphics[height=\rowheight]{images/results/S1_samples/S1_04_time_40_heatmap_20.pdf}
\includegraphics[height=\rowheight]{images/results/S1_samples/S1_04_time_40_heatmap_20_crop.pdf}
\includegraphics[height=\rowheight]{images/results/S1_samples/S1_04_time_40_heatmap_30.pdf}
\includegraphics[height=\rowheight]{images/results/S1_samples/S1_04_time_40_heatmap_30_crop.pdf}
\includegraphics[height=\rowheight]{images/results/S1_samples/S1_04_time_40_heatmap_40.pdf}
\includegraphics[height=\rowheight]{images/results/S1_samples/S1_04_time_40_heatmap_40_crop.pdf}
\end{minipage}\\
\caption{Randomly chosen output experiment \#4}
\end{figure*}
\begin{figure*}[h]
\centering
\begin{minipage}[t]{\linewidth}
\includegraphics[height=\rowheight]{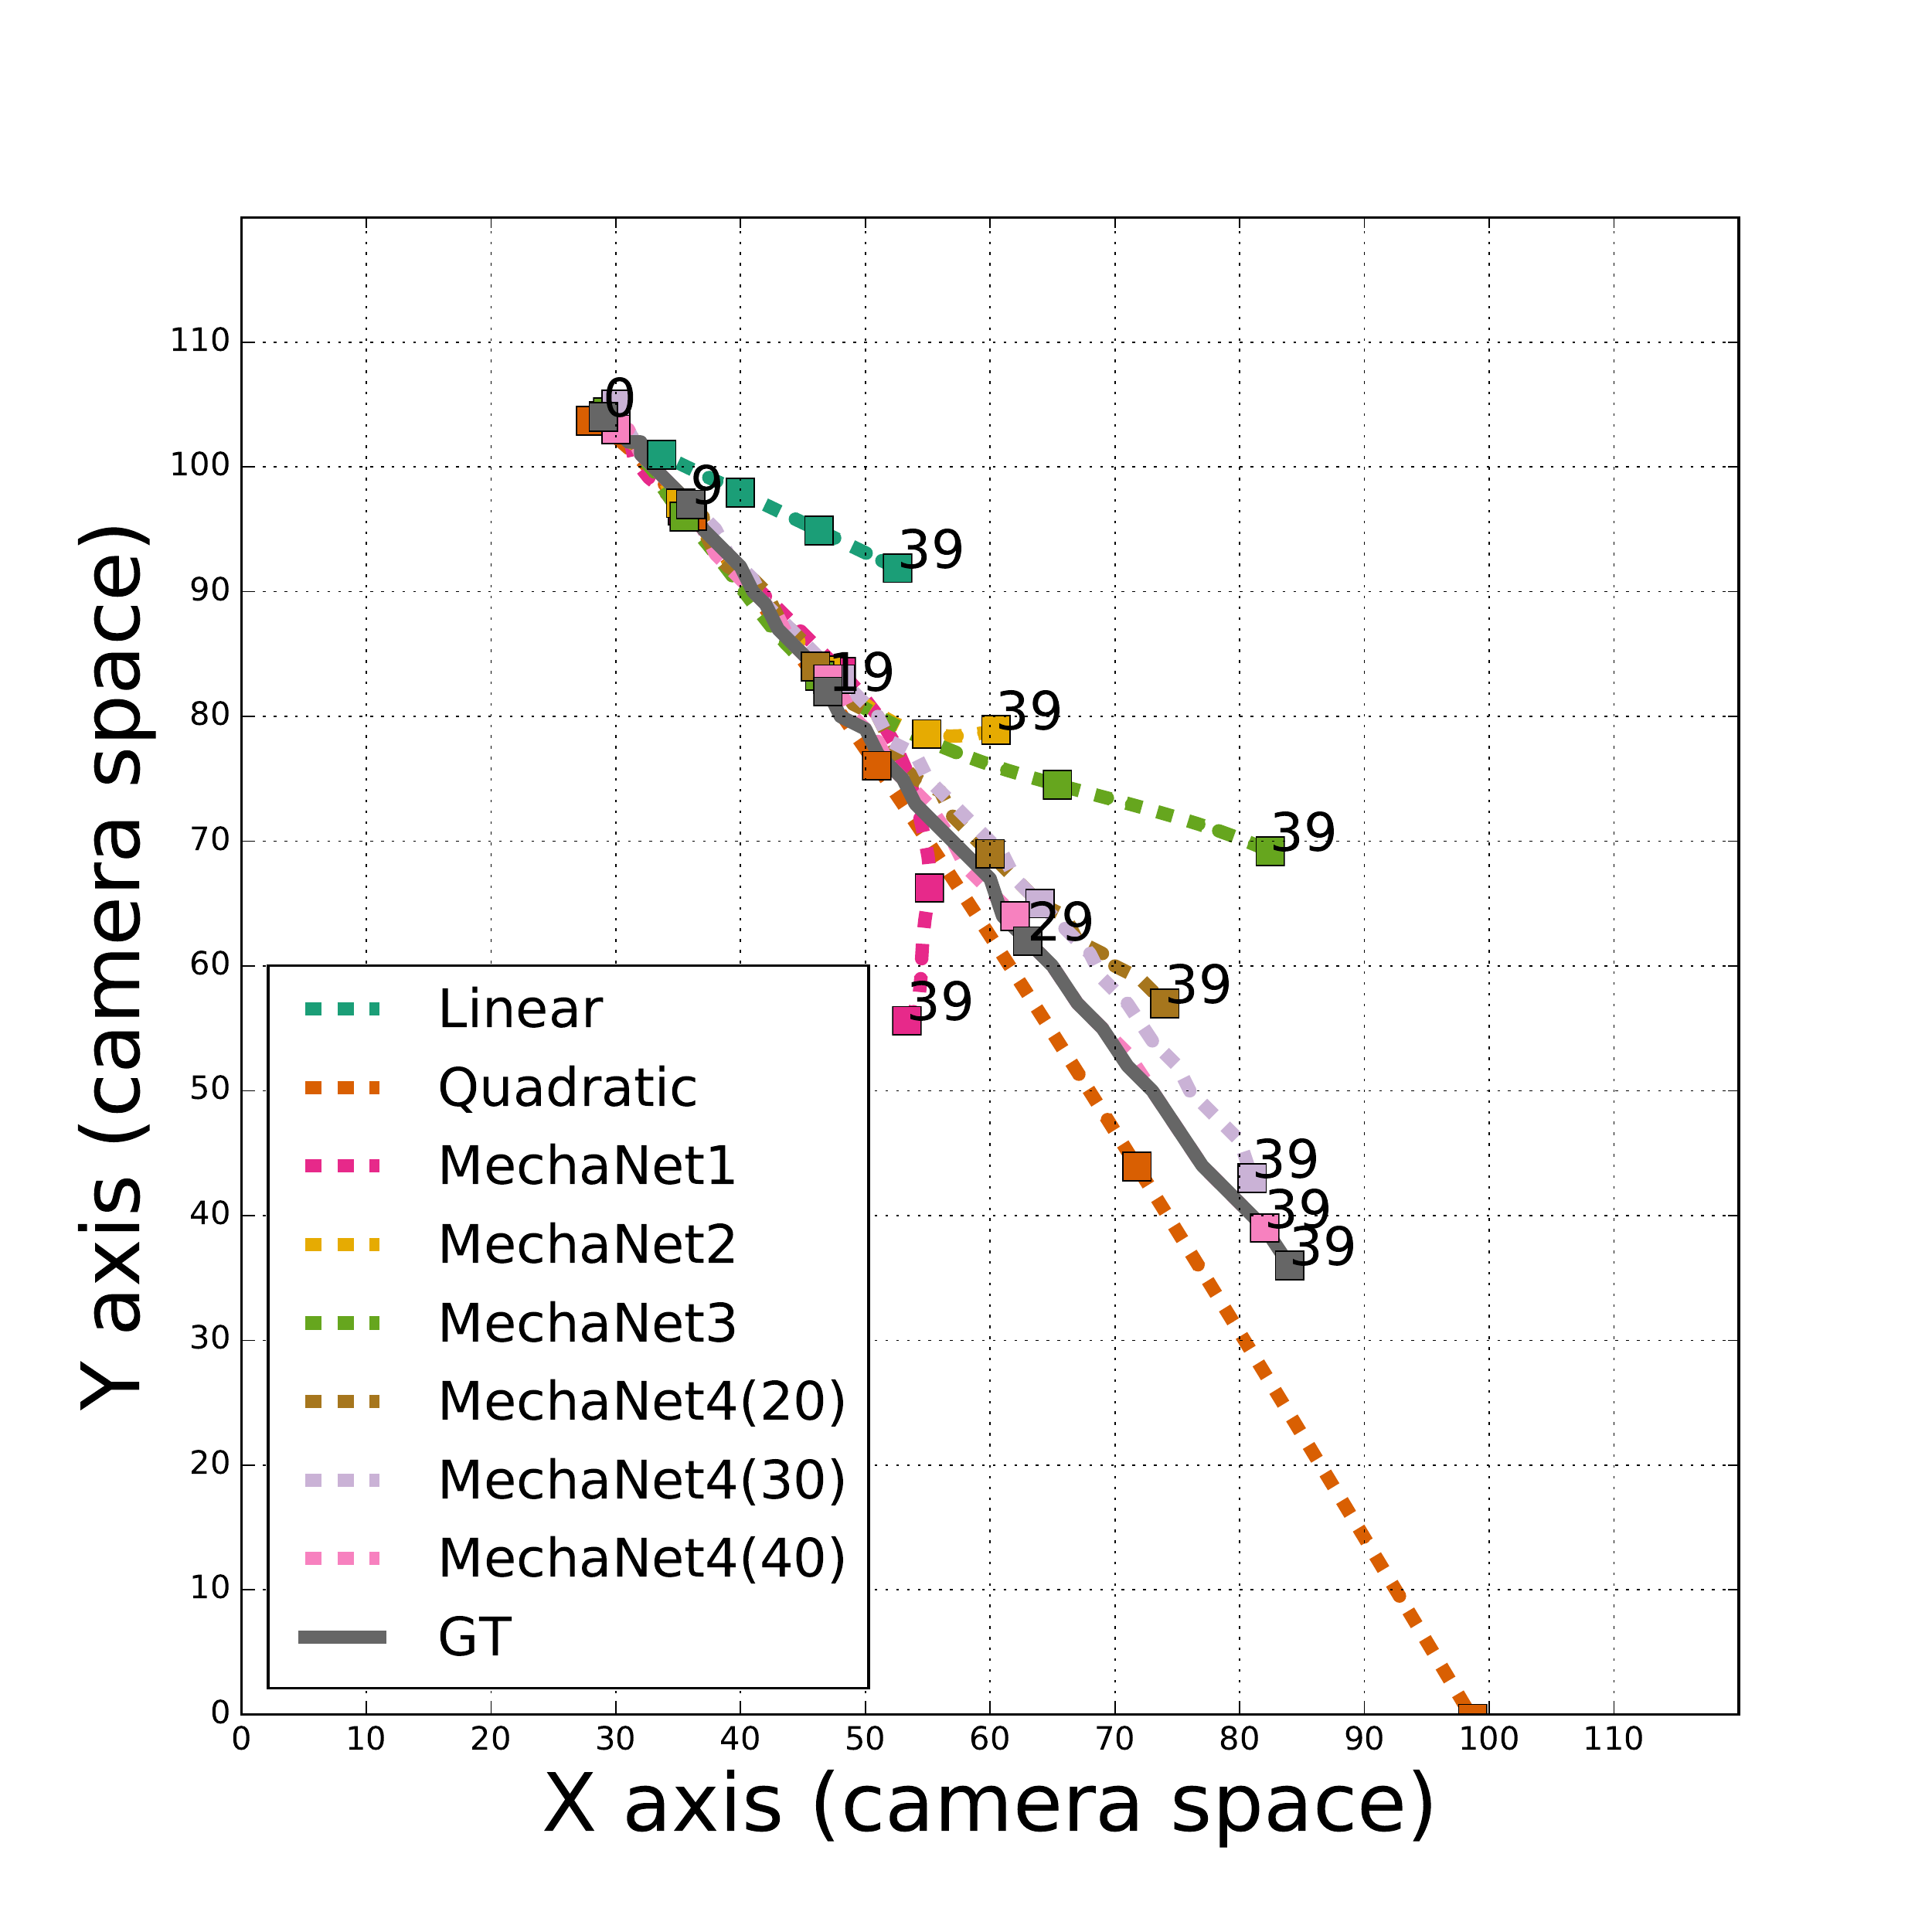}
\includegraphics[height=\rowheight]{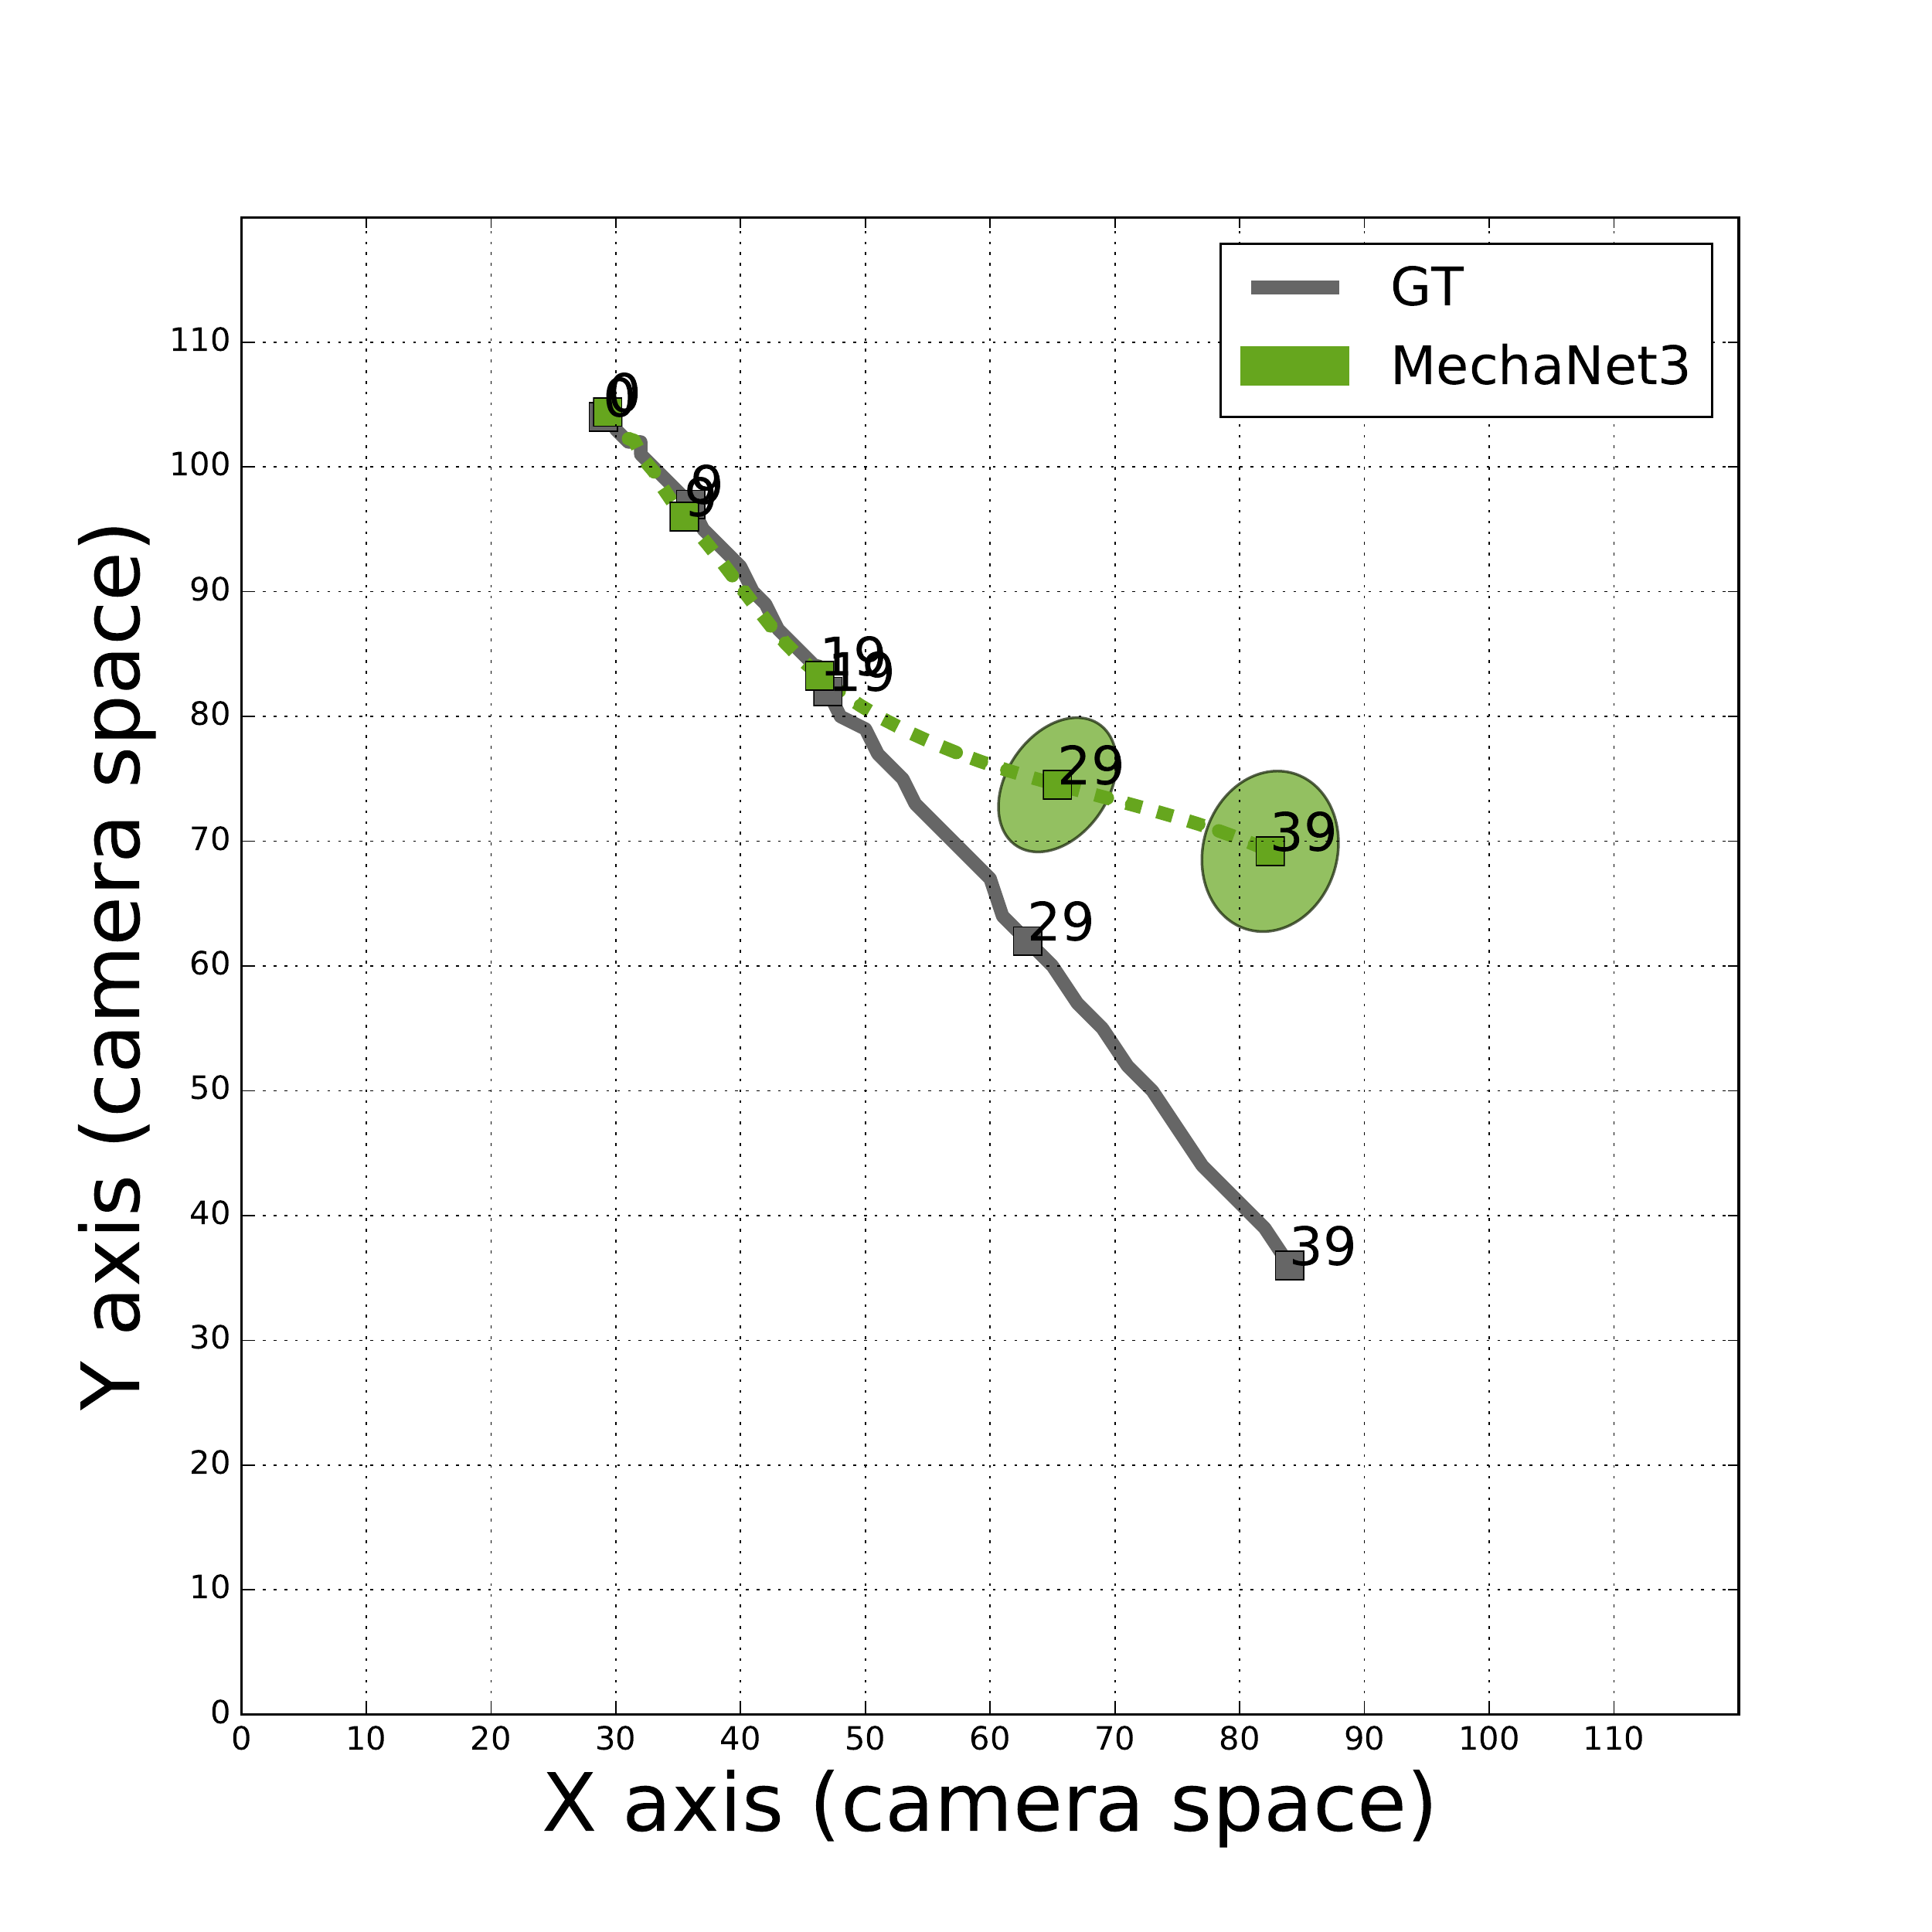}
\includegraphics[height=\rowheight]{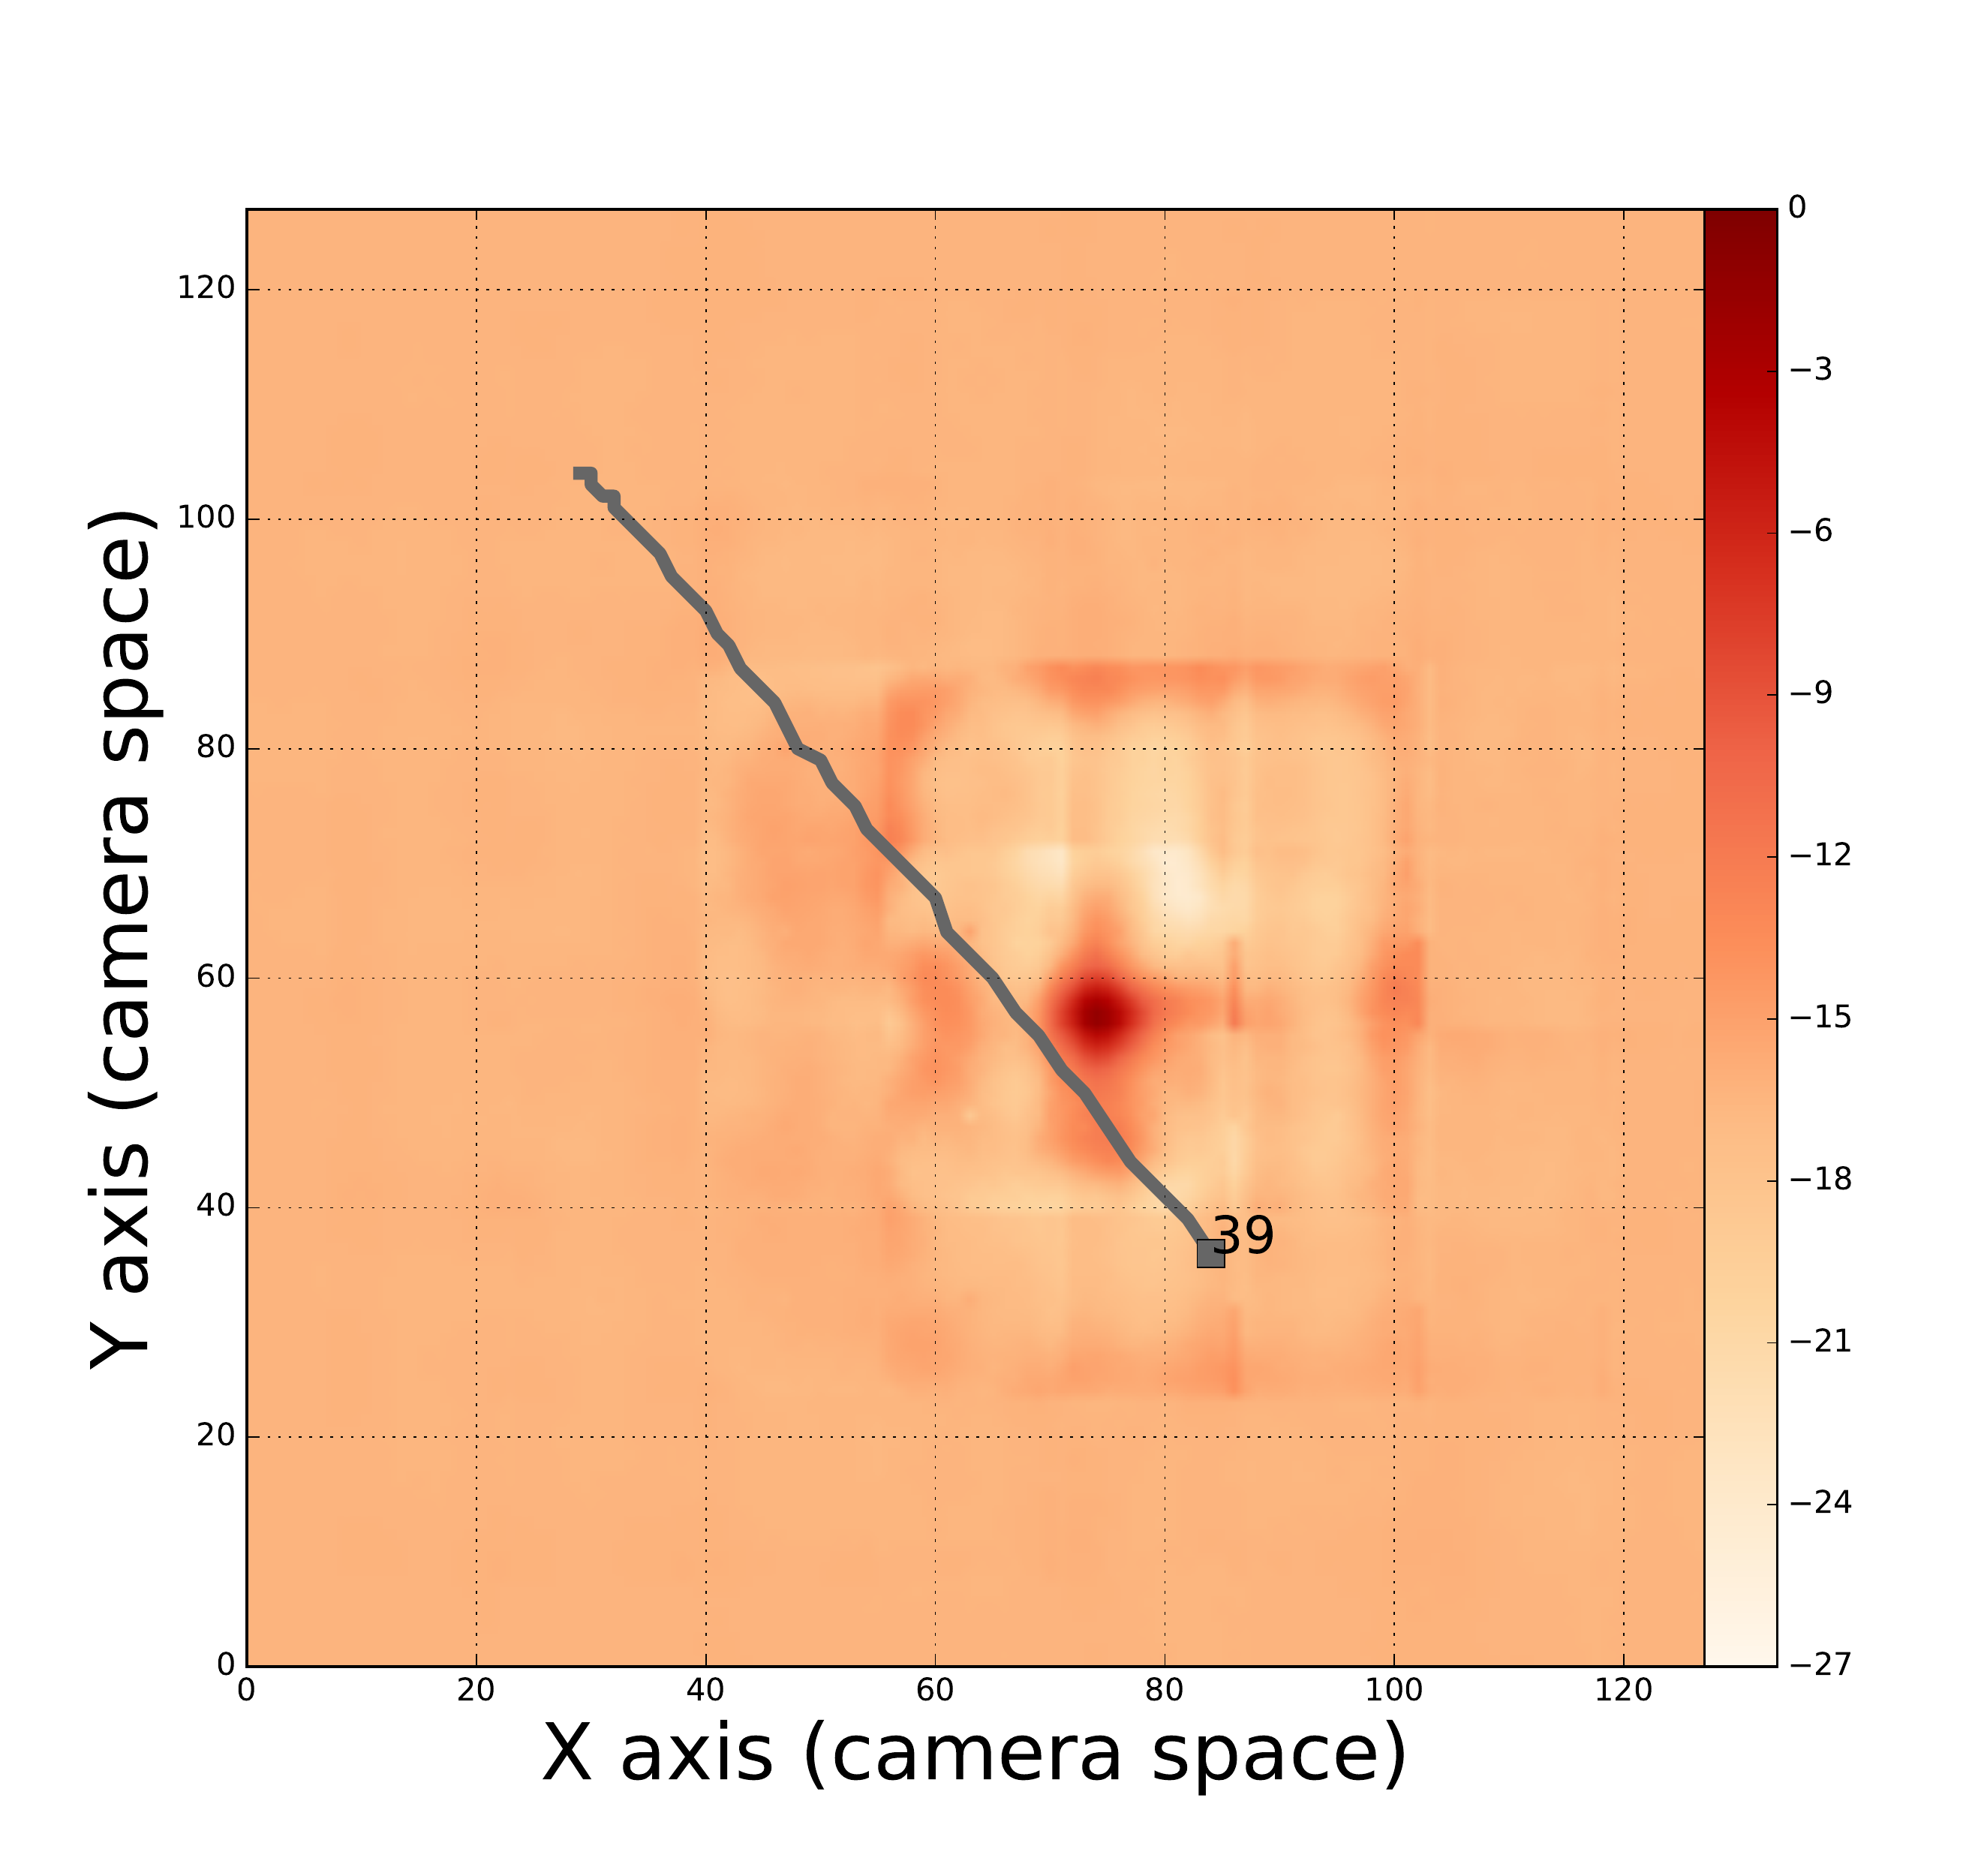}
\includegraphics[height=\rowheight]{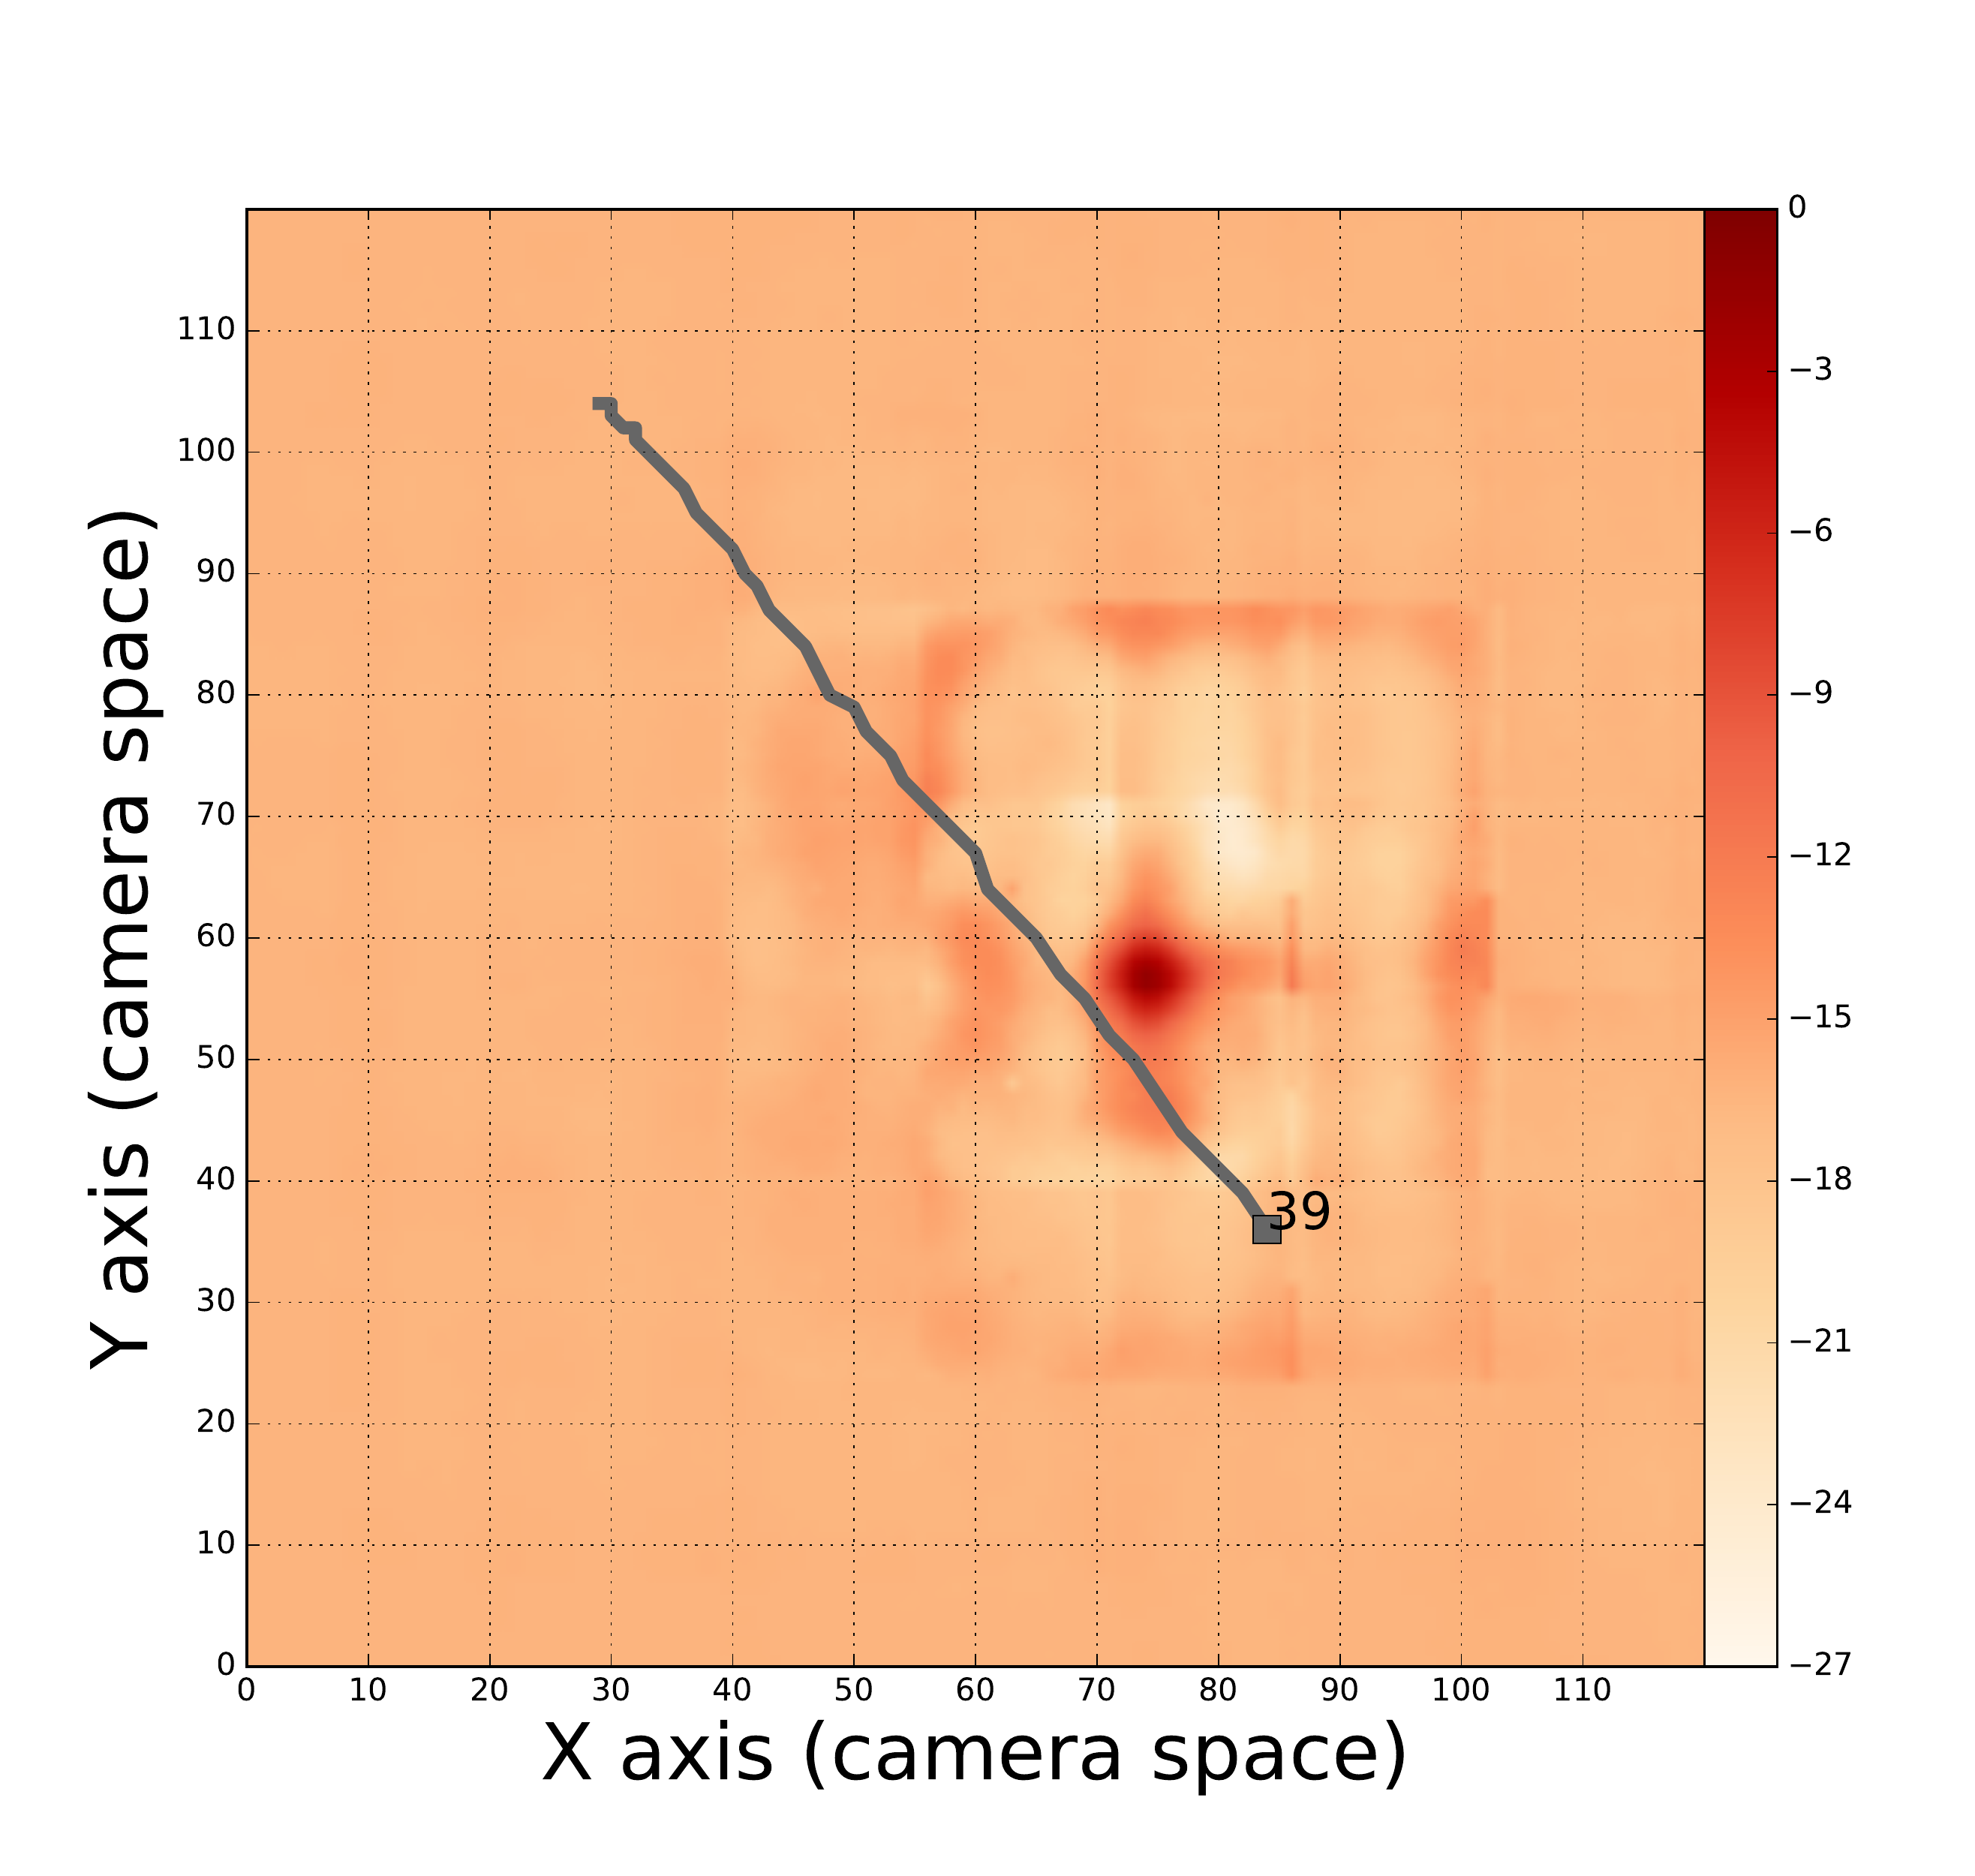}
\includegraphics[height=\rowheight]{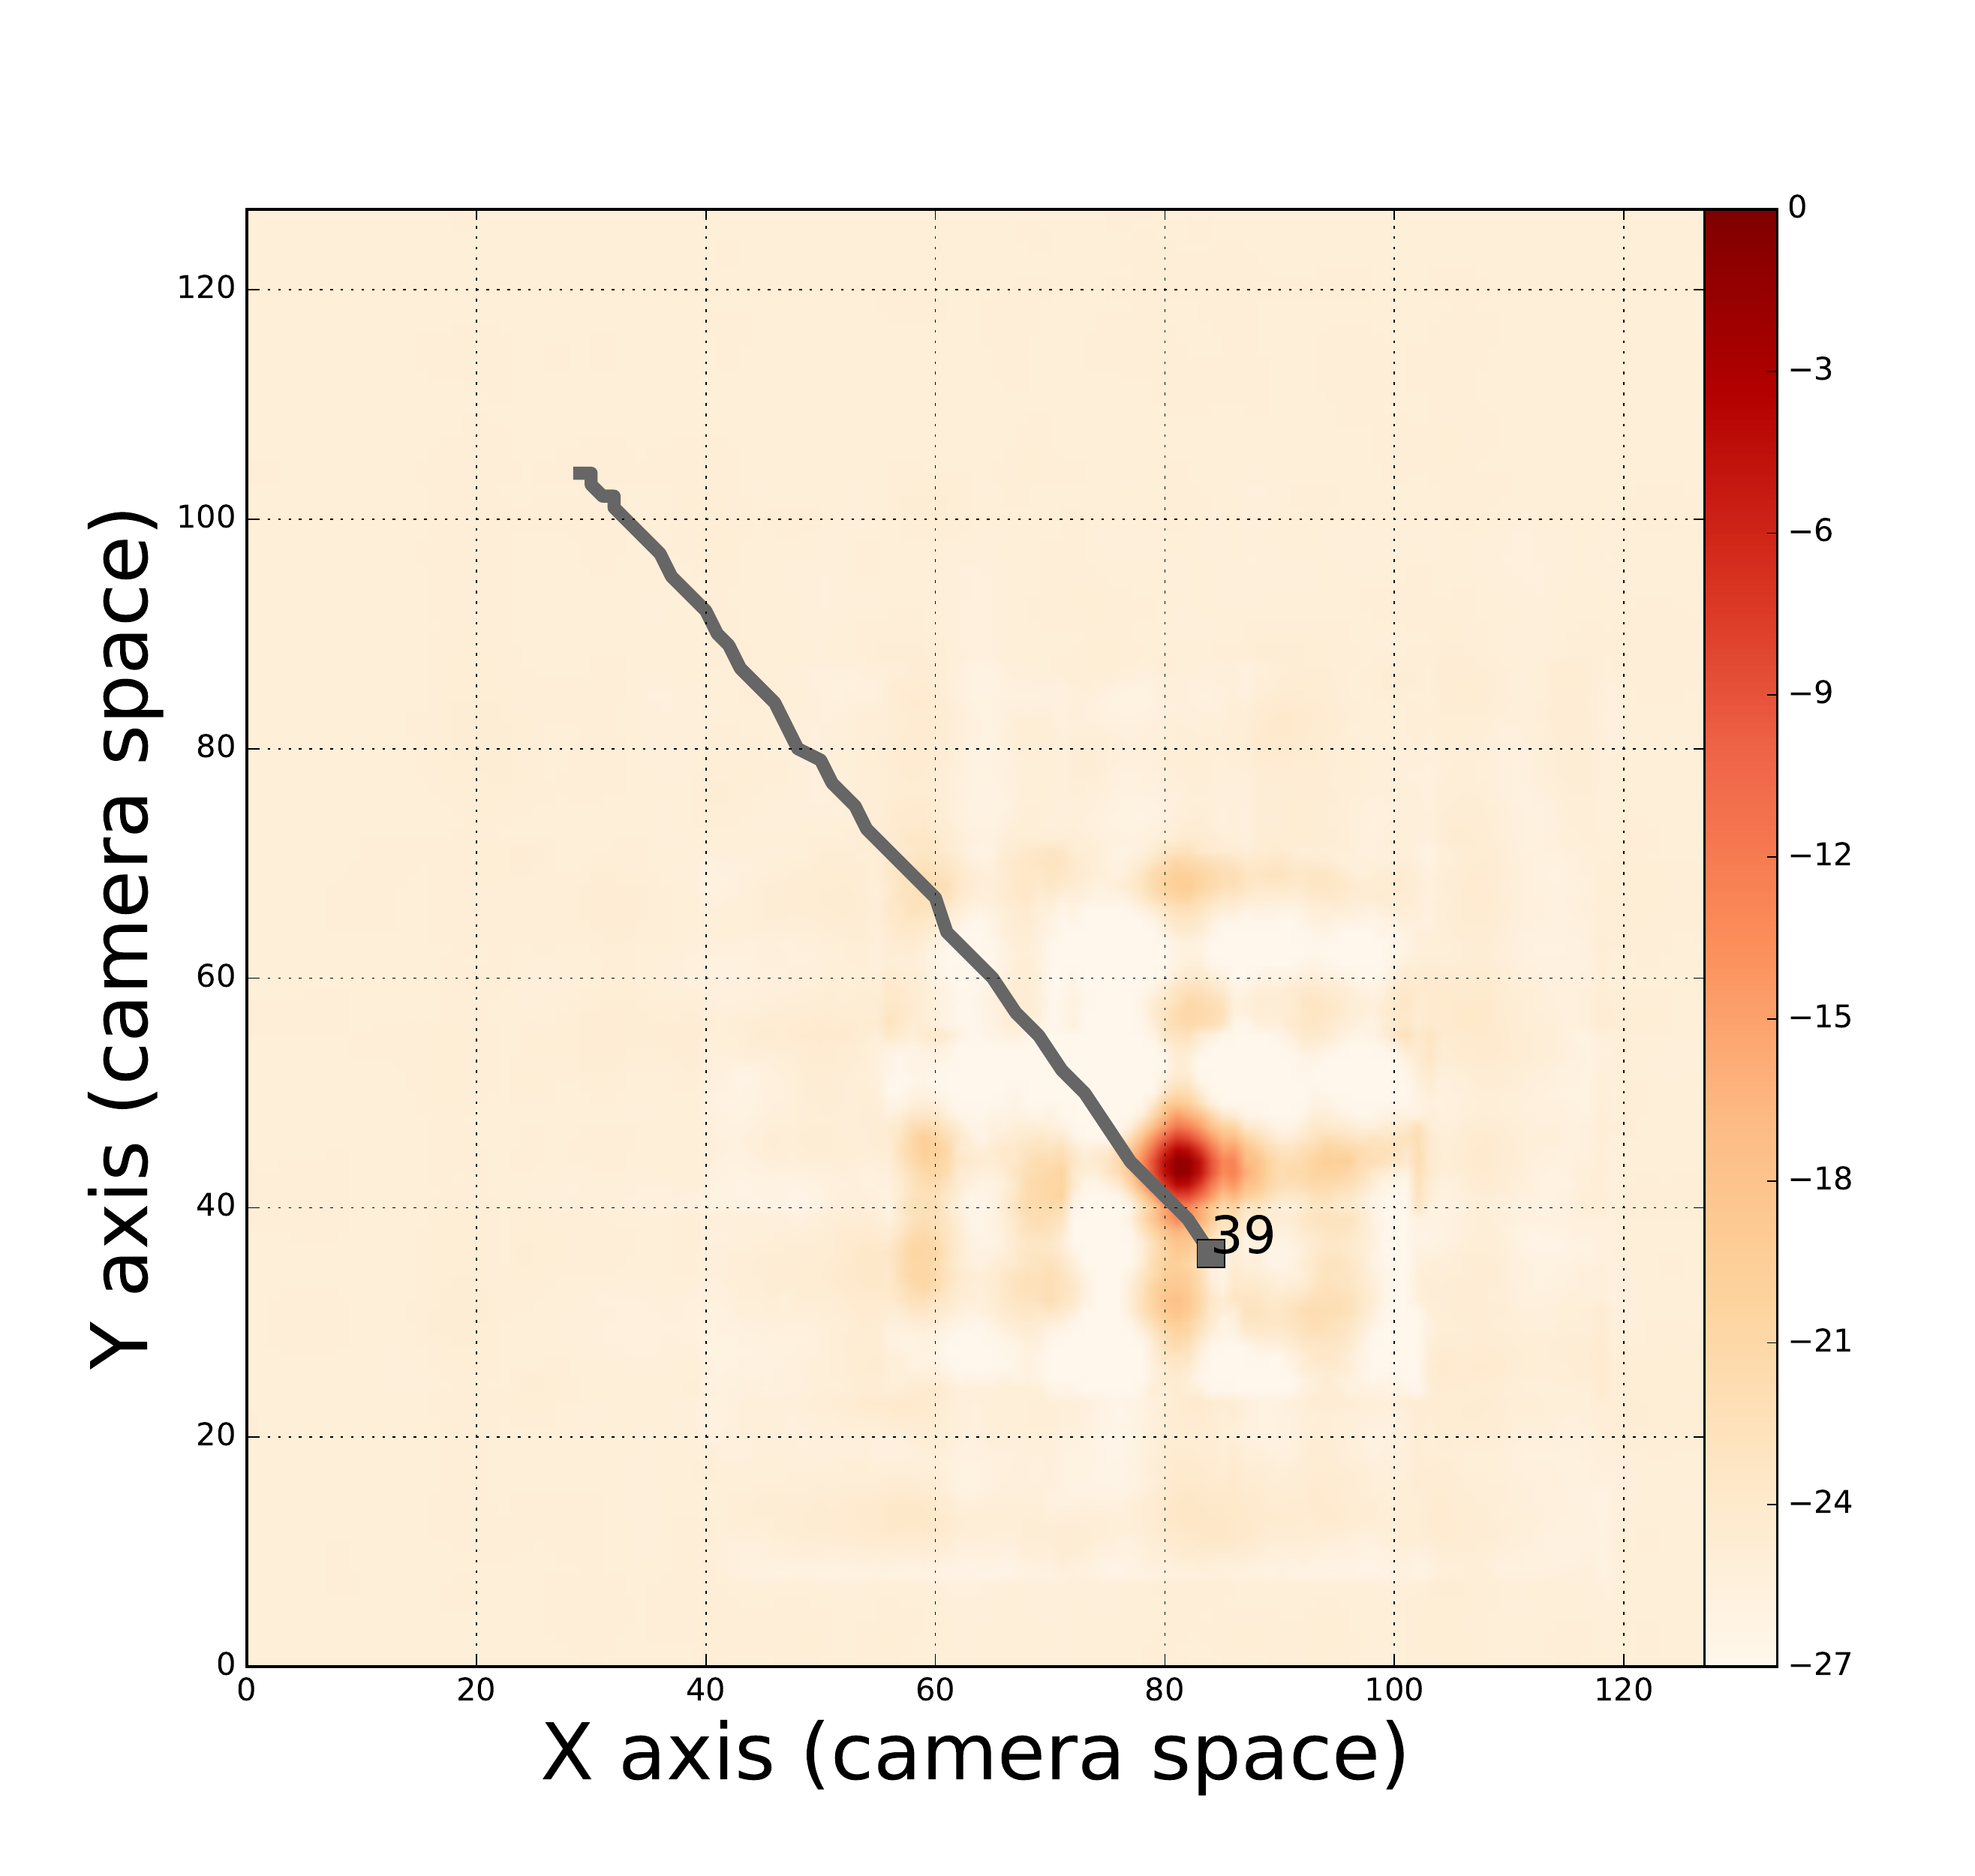}
\includegraphics[height=\rowheight]{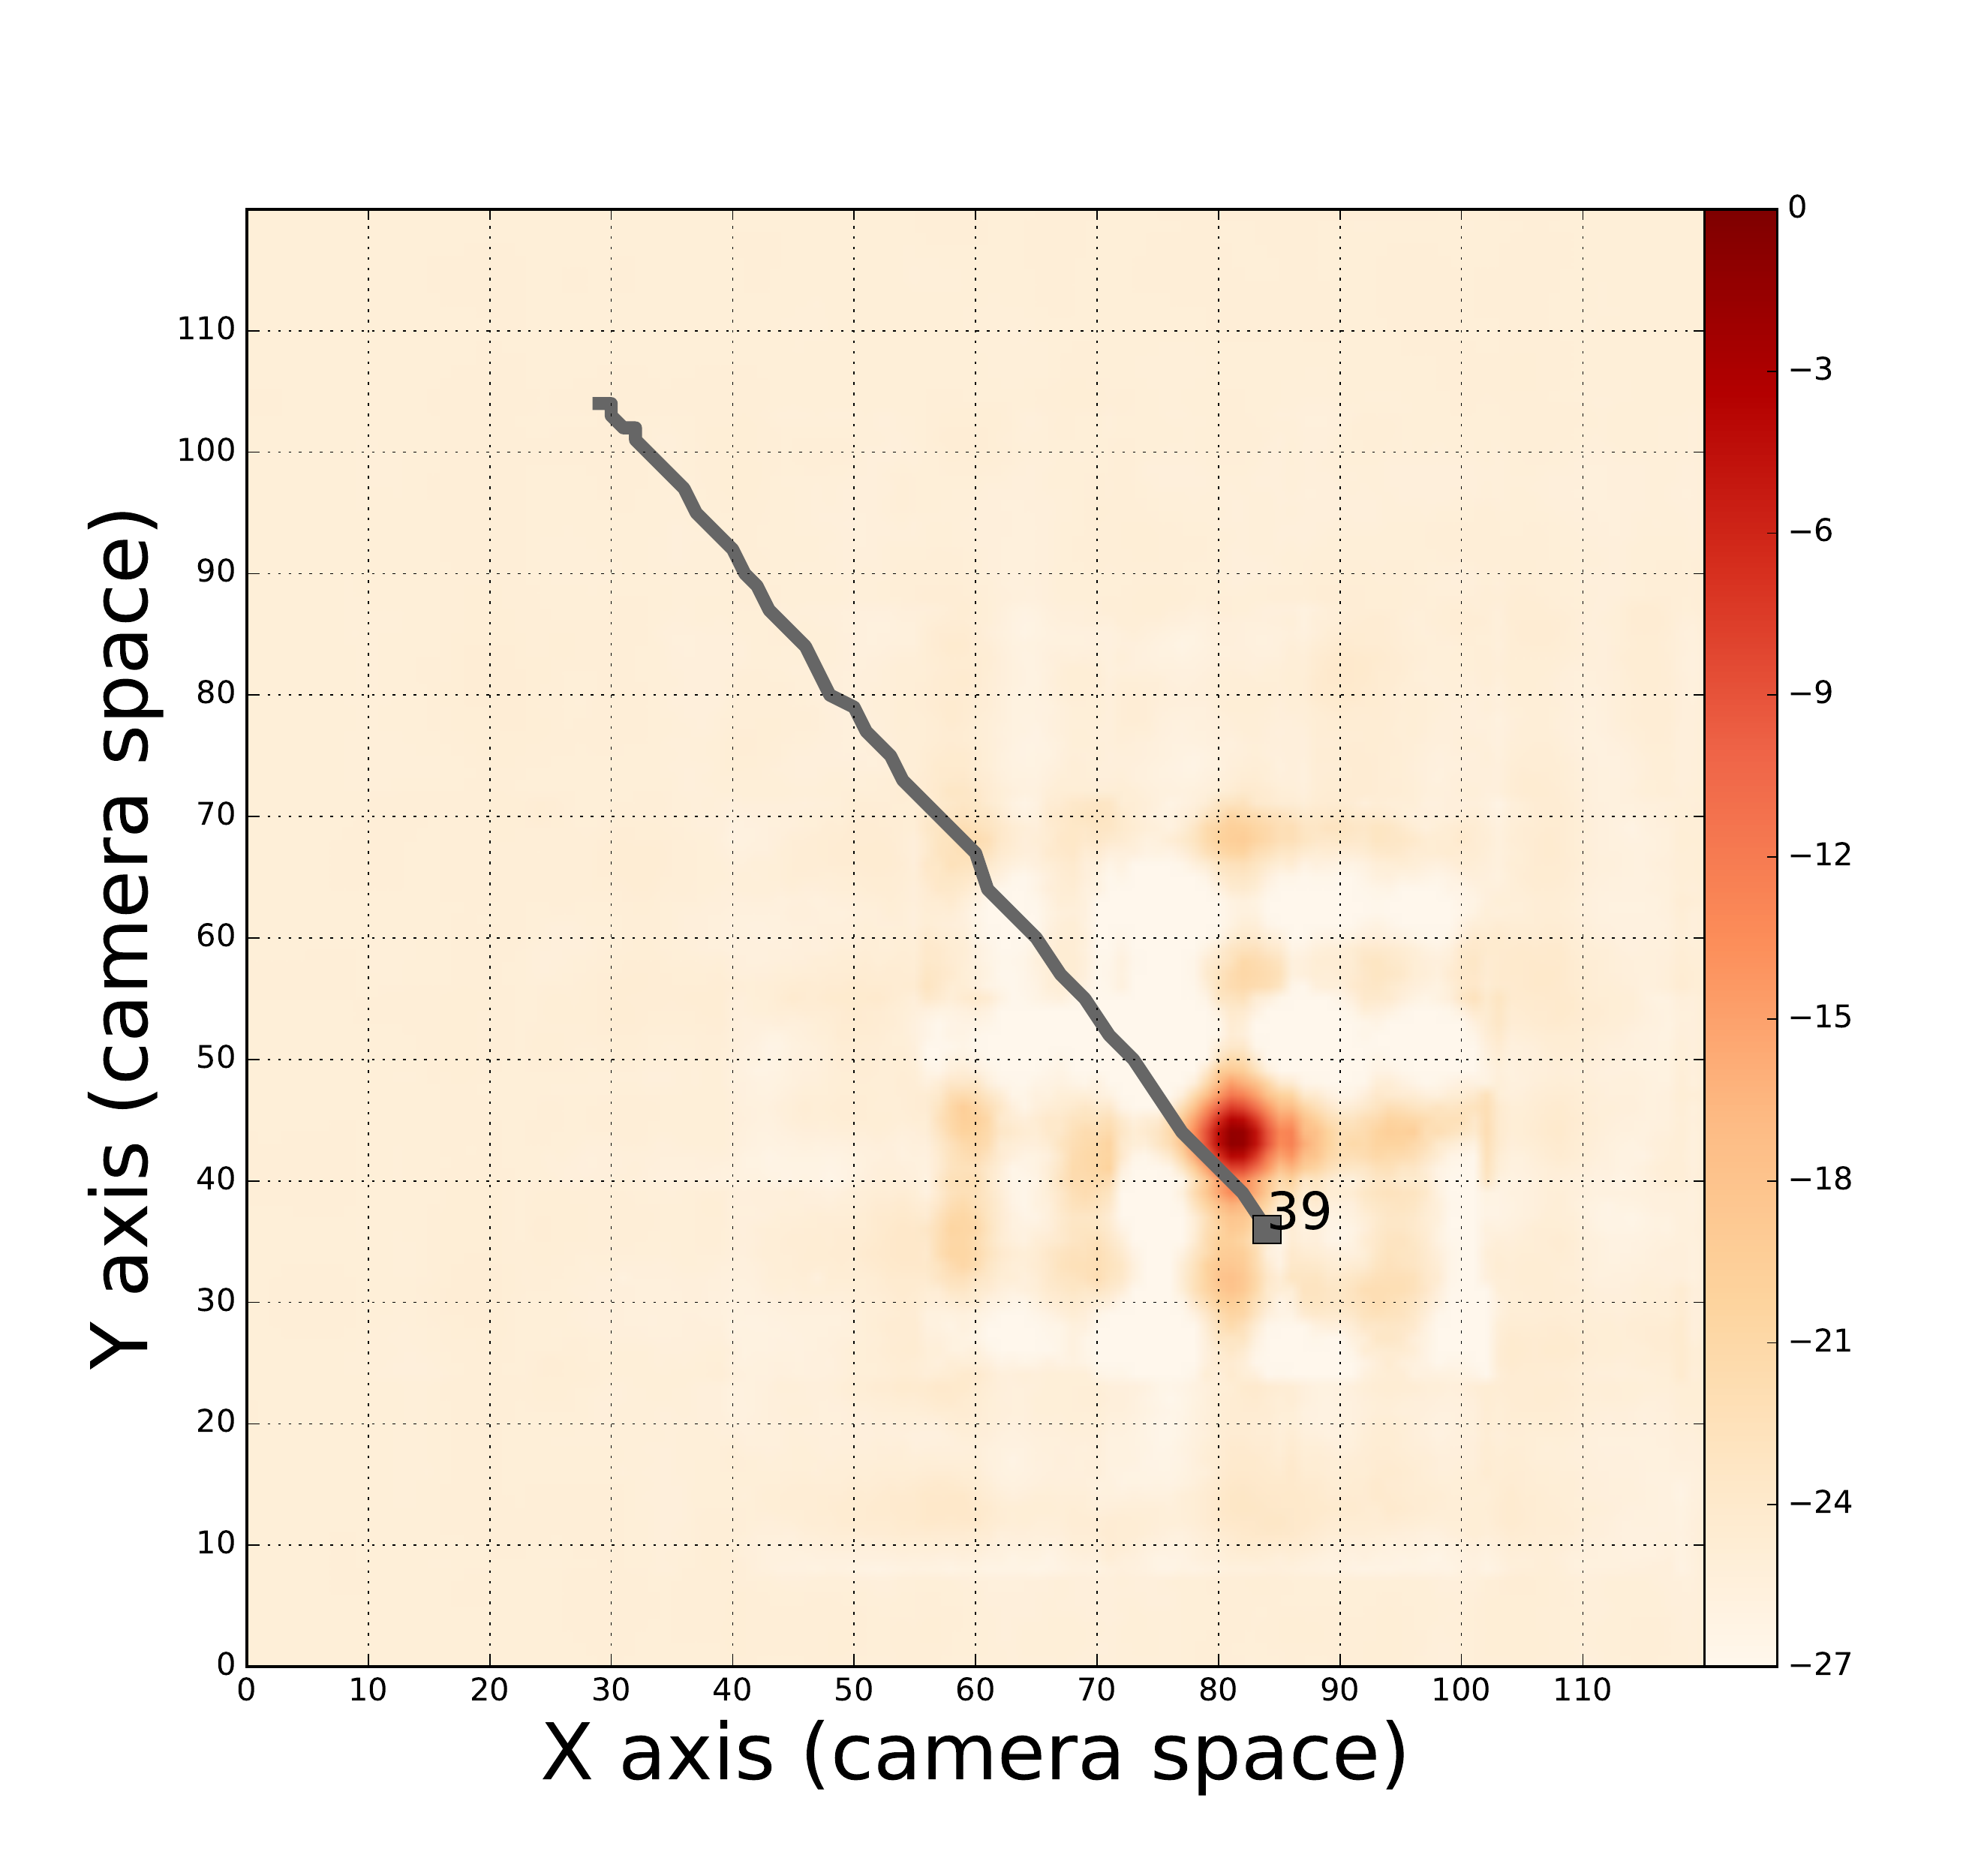}
\includegraphics[height=\rowheight]{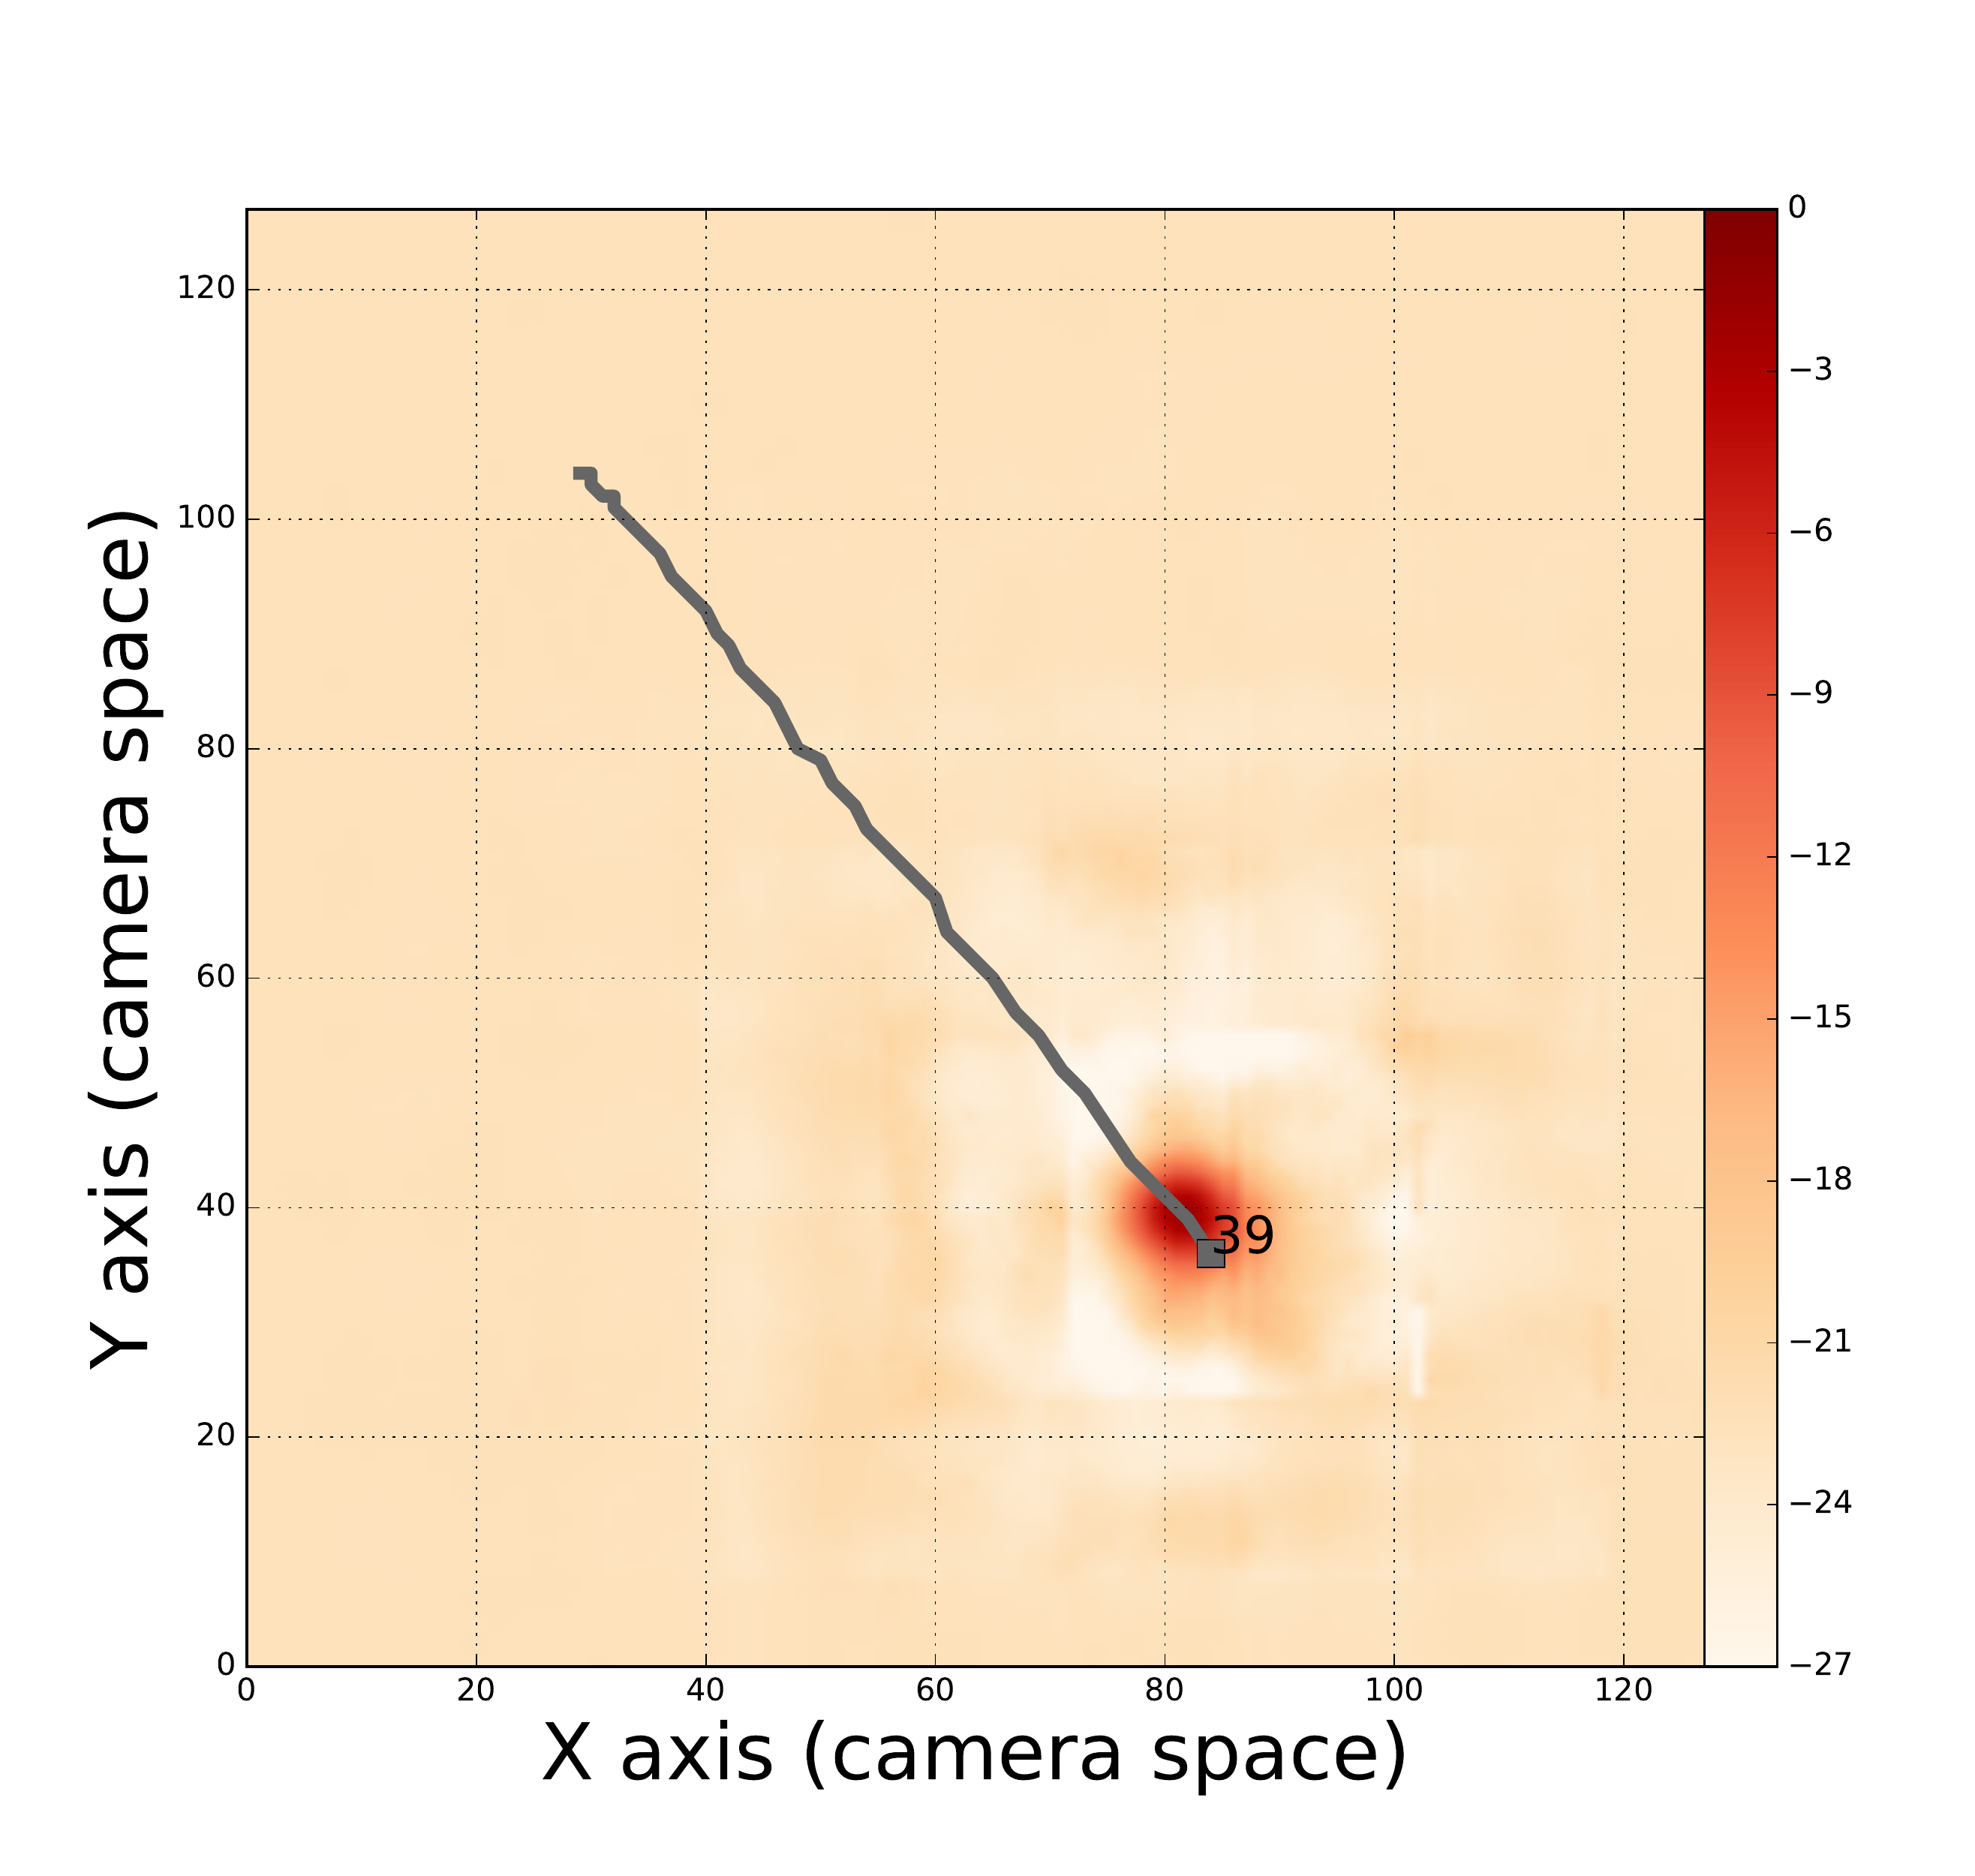}
\includegraphics[height=\rowheight]{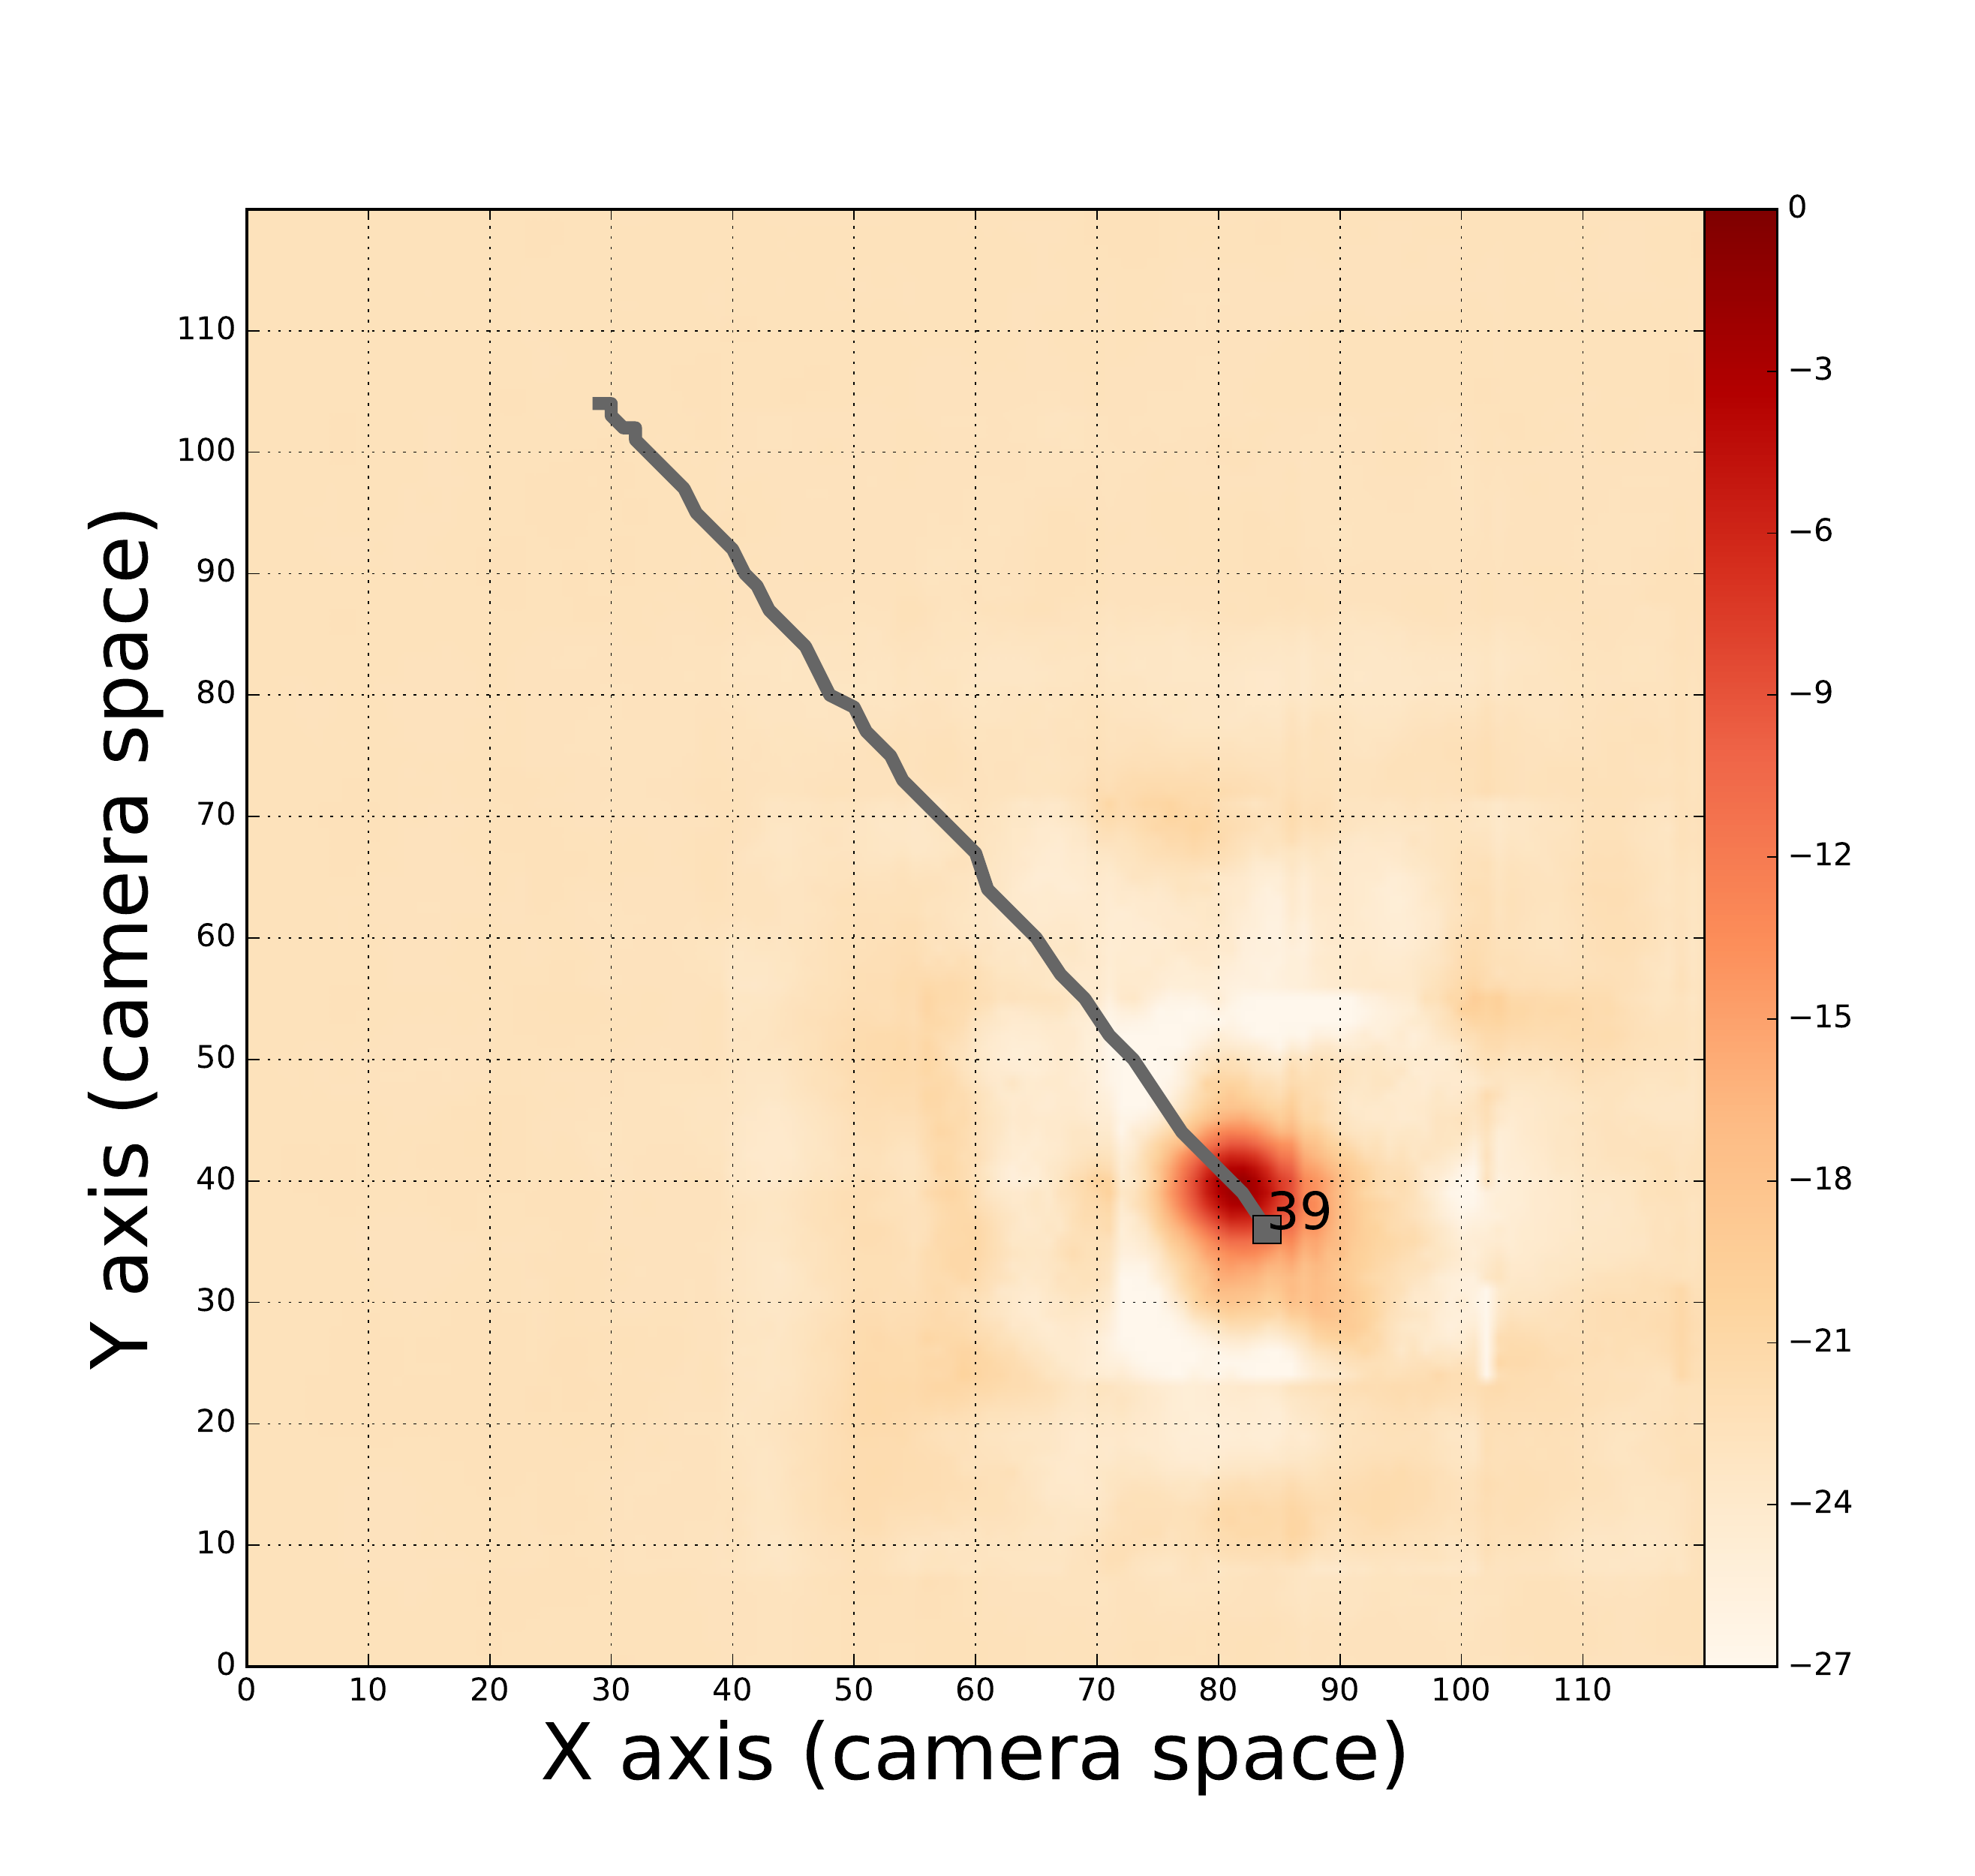}
\end{minipage}\\
\caption{Randomly chosen output experiment \#5}
\end{figure*}
\begin{figure*}[h]
\centering
\begin{minipage}[t]{\linewidth}
\includegraphics[height=\rowheight]{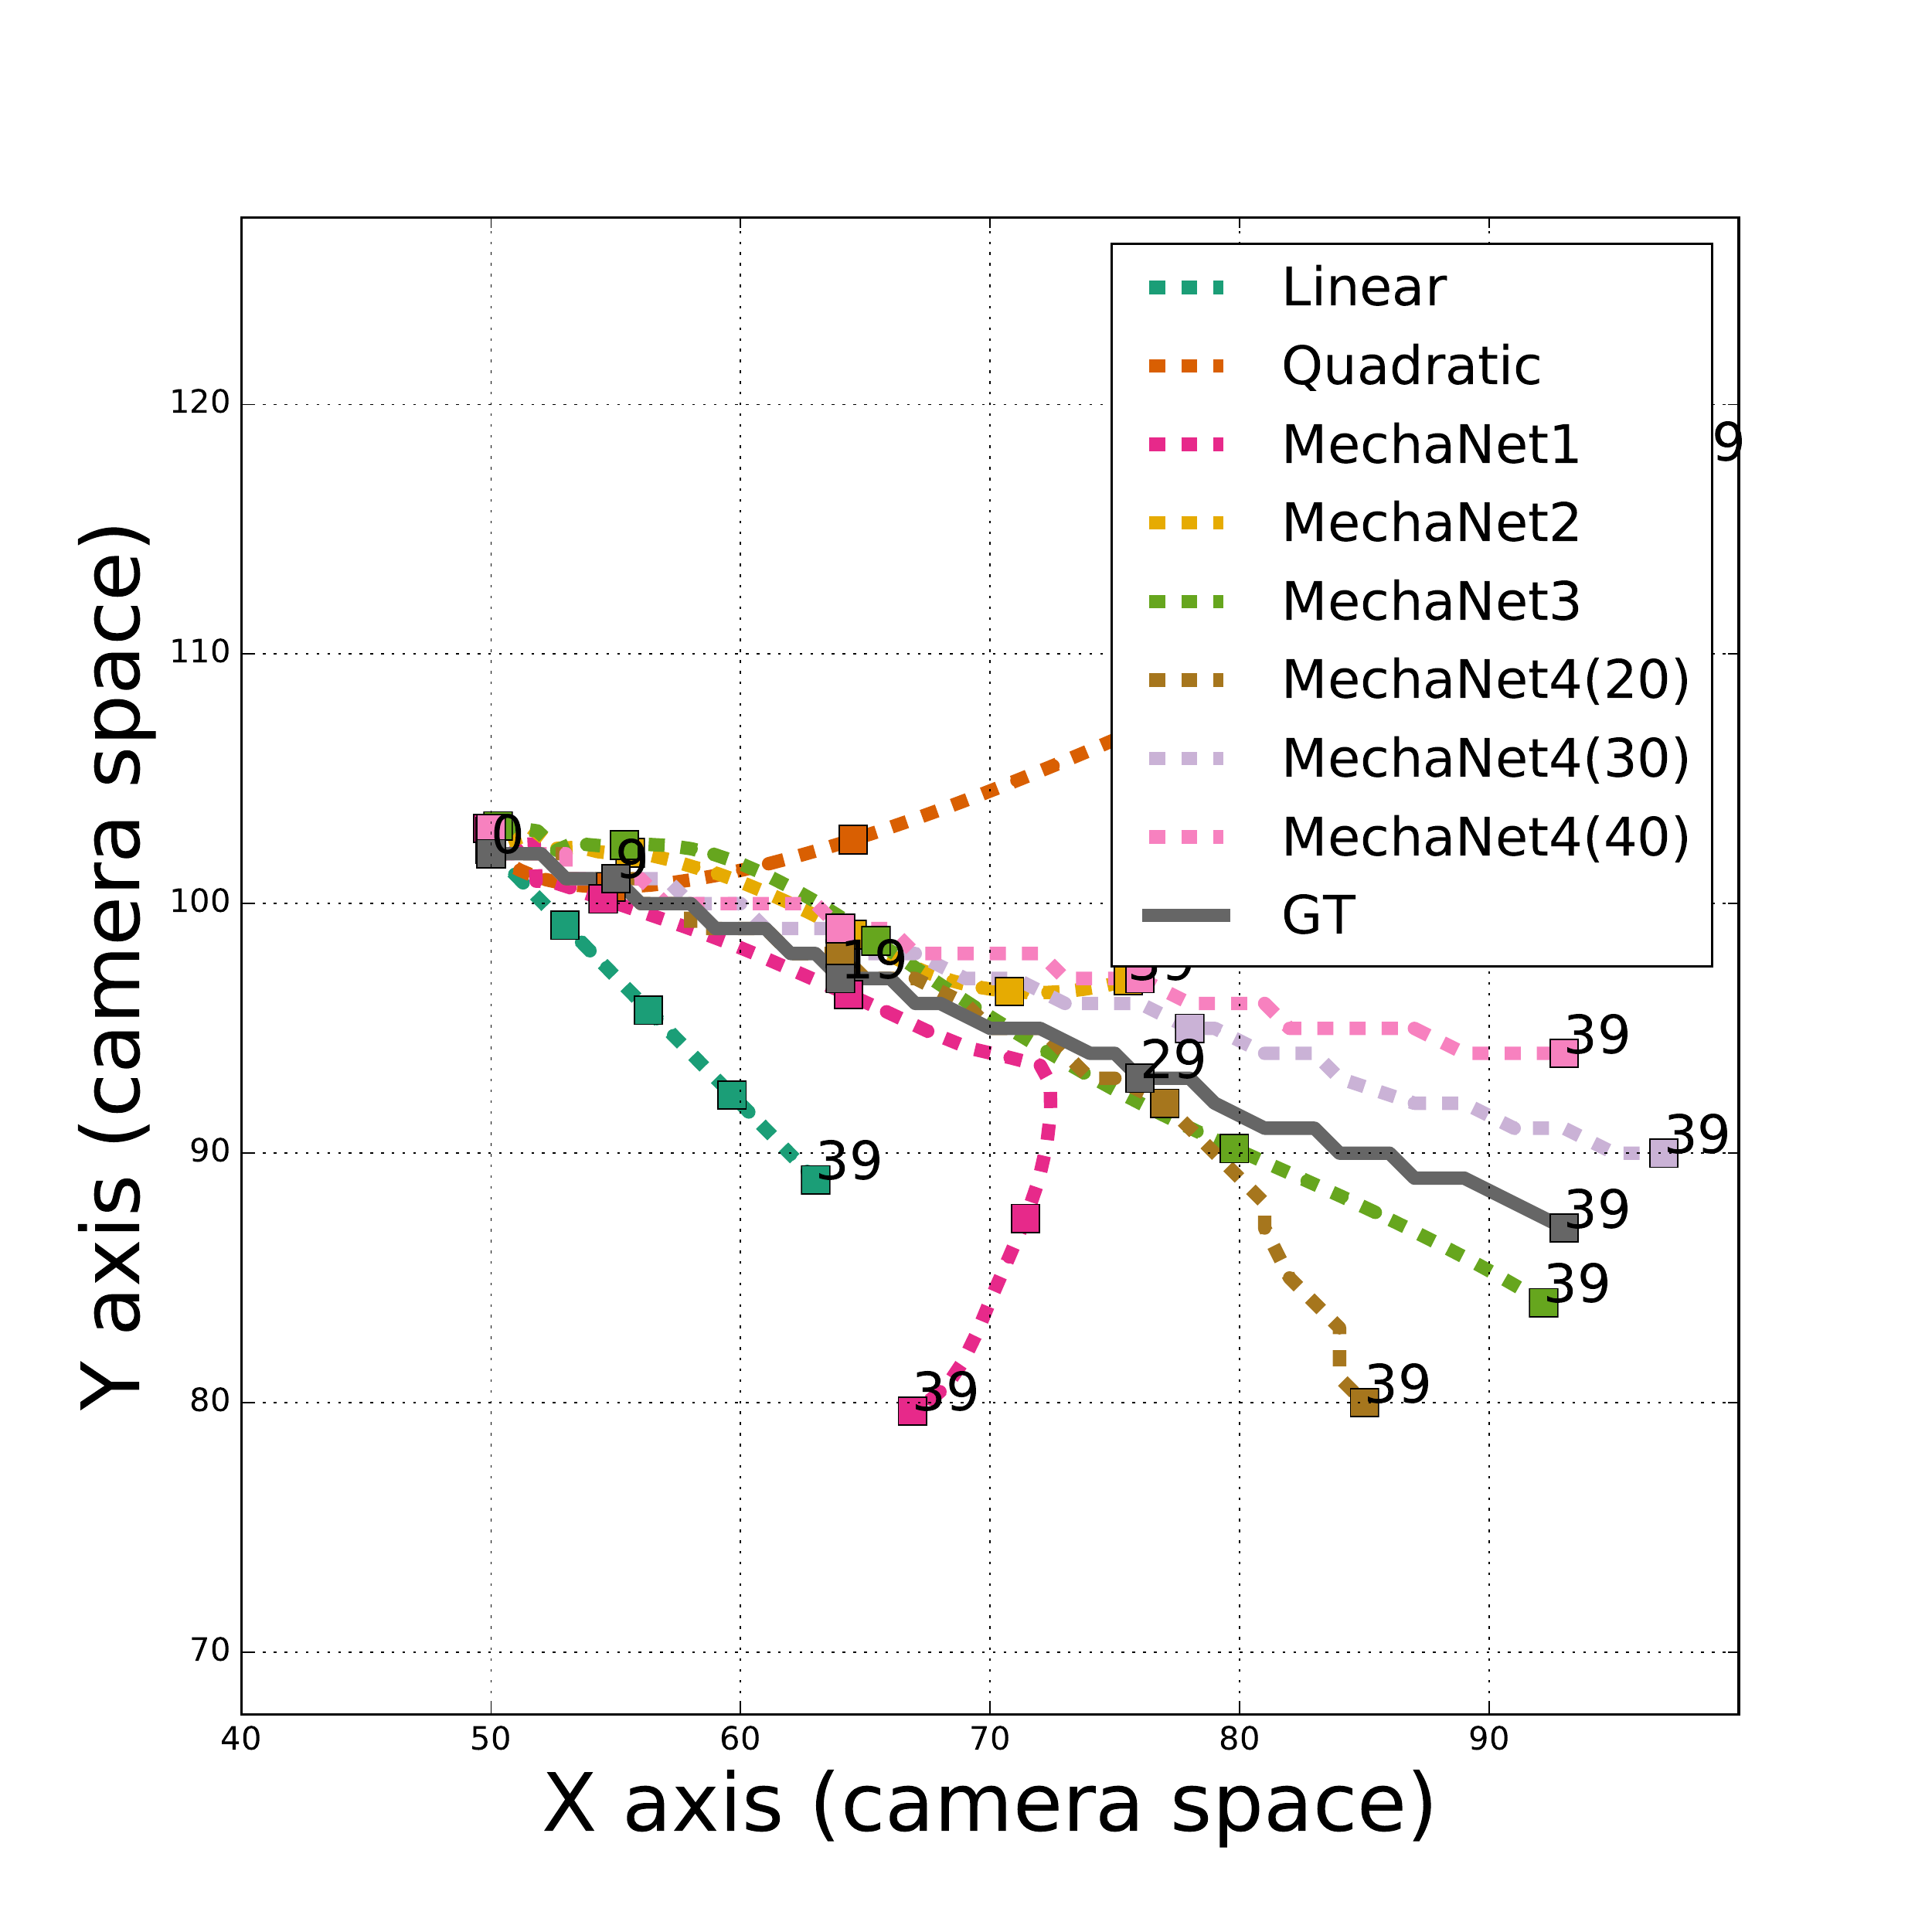}
\includegraphics[height=\rowheight]{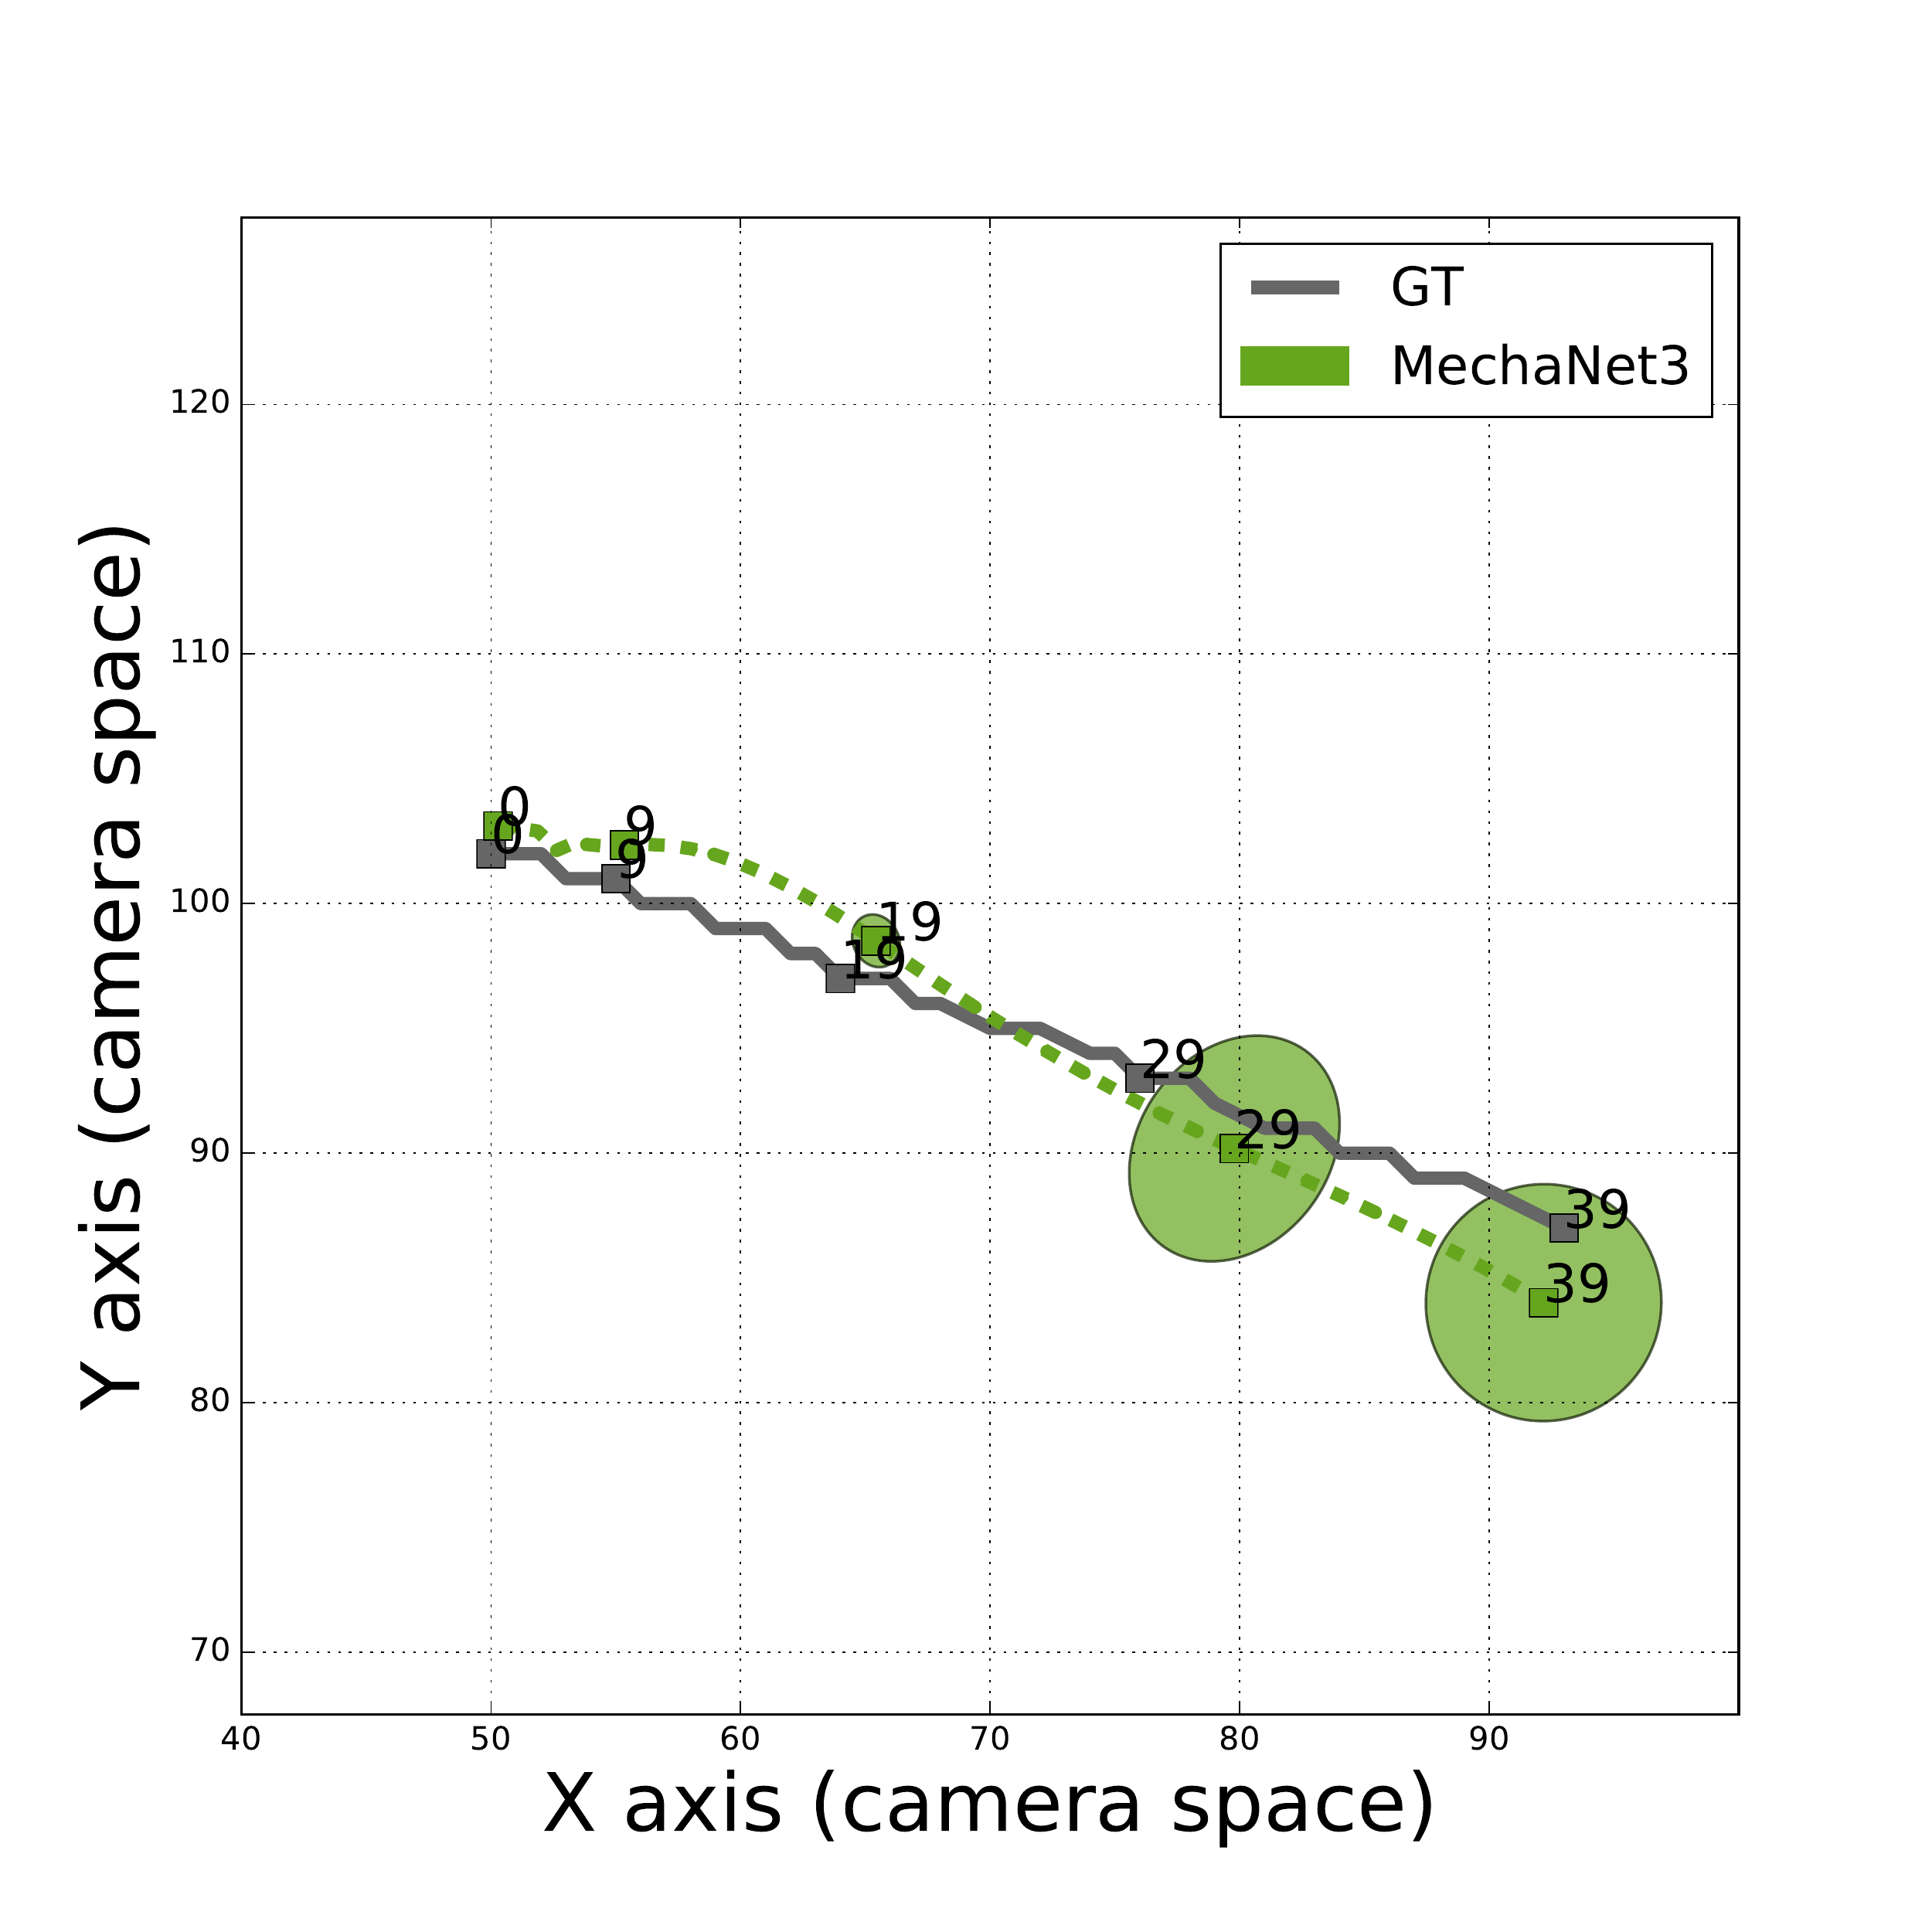}
\includegraphics[height=\rowheight]{images/results/S1_samples/S1_06_time_40_heatmap_20.pdf}
\includegraphics[height=\rowheight]{images/results/S1_samples/S1_06_time_40_heatmap_20_crop.pdf}
\includegraphics[height=\rowheight]{images/results/S1_samples/S1_06_time_40_heatmap_30.pdf}
\includegraphics[height=\rowheight]{images/results/S1_samples/S1_06_time_40_heatmap_30_crop.pdf}
\includegraphics[height=\rowheight]{images/results/S1_samples/S1_06_time_40_heatmap_40.pdf}
\includegraphics[height=\rowheight]{images/results/S1_samples/S1_06_time_40_heatmap_40_crop.pdf}
\end{minipage}\\
\caption{Randomly chosen output experiment \#6}
\end{figure*}
\begin{figure*}[h]
\centering
\begin{minipage}[t]{\linewidth}
\includegraphics[height=\rowheight]{images/results/S1_samples/S1_07_time_40.pdf}
\includegraphics[height=\rowheight]{images/results/S1_samples/S1_07_time_40_ellipses.pdf}
\includegraphics[height=\rowheight]{images/results/S1_samples/S1_07_time_40_heatmap_20.pdf}
\includegraphics[height=\rowheight]{images/results/S1_samples/S1_07_time_40_heatmap_20_crop.pdf}
\includegraphics[height=\rowheight]{images/results/S1_samples/S1_07_time_40_heatmap_30.pdf}
\includegraphics[height=\rowheight]{images/results/S1_samples/S1_07_time_40_heatmap_30_crop.pdf}
\includegraphics[height=\rowheight]{images/results/S1_samples/S1_07_time_40_heatmap_40.pdf}
\includegraphics[height=\rowheight]{images/results/S1_samples/S1_07_time_40_heatmap_40_crop.pdf}
\end{minipage}\\
\caption{Randomly chosen output experiment \#7}
\end{figure*}
\begin{figure*}[h]
\centering
\begin{minipage}[t]{\linewidth}
\includegraphics[height=\rowheight]{images/results/S1_samples/S1_08_time_40.pdf}
\includegraphics[height=\rowheight]{images/results/S1_samples/S1_08_time_40_ellipses.pdf}
\includegraphics[height=\rowheight]{images/results/S1_samples/S1_08_time_40_heatmap_20.pdf}
\includegraphics[height=\rowheight]{images/results/S1_samples/S1_08_time_40_heatmap_20_crop.pdf}
\includegraphics[height=\rowheight]{images/results/S1_samples/S1_08_time_40_heatmap_30.pdf}
\includegraphics[height=\rowheight]{images/results/S1_samples/S1_08_time_40_heatmap_30_crop.pdf}
\includegraphics[height=\rowheight]{images/results/S1_samples/S1_08_time_40_heatmap_40.pdf}
\includegraphics[height=\rowheight]{images/results/S1_samples/S1_08_time_40_heatmap_40_crop.pdf}
\end{minipage}\\
\caption{Randomly chosen output experiment \#8}
\end{figure*}
\begin{figure*}[h]
\centering
\begin{minipage}[t]{\linewidth}
\includegraphics[height=\rowheight]{images/results/S1_samples/S1_09_time_40.pdf}
\includegraphics[height=\rowheight]{images/results/S1_samples/S1_09_time_40_ellipses.pdf}
\includegraphics[height=\rowheight]{images/results/S1_samples/S1_09_time_40_heatmap_20.pdf}
\includegraphics[height=\rowheight]{images/results/S1_samples/S1_09_time_40_heatmap_20_crop.pdf}
\includegraphics[height=\rowheight]{images/results/S1_samples/S1_09_time_40_heatmap_30.pdf}
\includegraphics[height=\rowheight]{images/results/S1_samples/S1_09_time_40_heatmap_30_crop.pdf}
\includegraphics[height=\rowheight]{images/results/S1_samples/S1_09_time_40_heatmap_40.pdf}
\includegraphics[height=\rowheight]{images/results/S1_samples/S1_09_time_40_heatmap_40_crop.pdf}
\end{minipage}
\caption{Randomly chosen output experiment \#9}\end{figure*}
\endgroup
